# Supplementary material for: A search for variable subdwarf B stars in TESS Full Frame Images III. An update on variable targets in both ecliptic hemispheres -- contamination analysis and new sdB pulsators
Source: arXiv:2301.01082 ancillary file (2023-01-03)
Supplement: Supplementary file 1 [file 11-south_no_spec_FTs.pdf]

**Table 11. SEH - 1262 spectroscopically unclassified variables with amplitude spectra**

| No. | Gaia DR2            | TIC        | G     | Variable contaminator                                                                   |
|-----|---------------------|------------|-------|-----------------------------------------------------------------------------------------|
|     |                     |            | [mag] |                                                                                         |
| 1   | 2326333512204996992 | 380826878  | 15.69 | none                                                                                    |
| 2   | 2342907791000463232 | 610076106  | 17.18 | [SHM2017] J013.19449-26.56892 (RR Lyr)                                                  |
| 3   | 2342907962798690944 | 610077229  | 16.68 | [SHM2017] J013.19449-26.56892 (RR Lyr)                                                  |
| 4   | 2409630520260038784 | 2052262357 | 18.09 | Cl* NGC 7492 C 1306 (RR Lyr)                                                            |
| 5   | 2410677839445234944 | 111183765  | 14.48 | none                                                                                    |
| 6   | 2452347332977710208 | 629985497  | 17.90 | none                                                                                    |
| 7   | 2482810406432480512 | 610652043  | 18.39 | none                                                                                    |
| 8   | 2494281851762928512 | 250416977  | 14.37 | none                                                                                    |
| 9   | 2884515983209409152 | 20144117   | 14.48 | none                                                                                    |
| 10  | 2885588247565266176 | 124848134  | 13.25 | none                                                                                    |
| 11  | 2892303274314997632 | 705676754  | 18.38 | < 23 $\mu$ Hz: * lam CMa (B4V);<br>24.54 $\mu$ Hz+harmonics: CRTS J062820.0-323300 (EB) |
| 12  | 2894062664718232576 | 51902160   | 14.51 | none                                                                                    |
| 13  | 2894607919407035136 | 172461490  | 16.10 | no signal in individual pixels                                                          |
| 14  | 2895491617518092928 | 705881507  | 16.64 | CRTS J063516.1-282940 (EB)                                                              |
| 15  | 2899766827964264192 | 49707471   | 12.47 | none                                                                                    |
| 16  | 2905054104502350720 | 706315250  | 17.06 | none                                                                                    |
| 17  | 2915030450240829696 | 706688289  | 17.45 | none                                                                                    |
| 18  | 2915959404426627328 | 93443430   | 14.53 | none                                                                                    |
| 19  | 2917647704532106624 | 33598289   | 15.39 | none                                                                                    |
| 20  | 2919889883618031104 | 172410935  | 15.87 | Gaia EDR3 2919889883618032000                                                           |
| 21  | 2921905494592383104 | 53746254   | 14.11 | none                                                                                    |
| 22  | 2922129863681744896 | 172925290  | 14.96 | no signal in individual pixels                                                          |
| 23  | 2922496653888398976 | 744429291  | 10.71 | none                                                                                    |
| 24  | 2926097657551506944 | 78442527   | 16.10 | no signal in individual pixels                                                          |
| 25  | 2927754862098340864 | 80952313   | 15.69 | signal in all pixels                                                                    |
| 26  | 2927944940172059648 | 99829121   | 14.46 | none                                                                                    |
| 27  | 2929905678637186688 | 99926537   | 10.89 | no signal in individual pixels                                                          |
| 28  | 2931232303833617408 | 746001037  | 18.74 | signal in all pixels                                                                    |
| 29  | 2937043532023825024 | 707208969  | 15.87 | none                                                                                    |
| 30  | 2947467795606031744 | 322897154  | 14.09 | none                                                                                    |
| 31  | 2954990241846491648 | 708311699  | 18.95 | none                                                                                    |
| 32  | 2957939922307252992 | 708349759  | 18.78 | NGC 1904 204 (RR Lyr)                                                                   |
| 33  | 2957939926606933888 | 708349812  | 17.32 | NGC 1904 204 (RR Lyr)                                                                   |
| 34  | 2957940132760404736 | 708351233  | 17.69 | NGC 1904 204 (RR Lyr)                                                                   |
| 35  | 2957940201479869056 | 708351515  | 17.22 | NGC 1904 204 (RR Lyr)                                                                   |
| 36  | 2989388566201582848 | 671452197  | 18.94 | none                                                                                    |
| 37  | 2990095865712197632 | 24346296   | 16.63 | none                                                                                    |
| 38  | 3009561482131683328 | 46273443   | 17.13 | none                                                                                    |
| 39  | 3012930656340169216 | 710201725  | 18.62 | none                                                                                    |
| 40  | 3027974213095327616 | 385874395  | 15.03 | TYC 5966-1776-1                                                                         |
| 41  | 3032890473180888192 | 749940934  | 12.44 | none                                                                                    |
| 42  | 3035322730338241792 | 6609005    | 13.24 | none                                                                                    |



|    |                     |           |       |                                                                 |
|----|---------------------|-----------|-------|-----------------------------------------------------------------|
| 43 | 3036352663493806720 | 750695119 | 16.78 | signal in all pixels                                            |
| 44 | 3037414134591183488 | 750848412 | 18.70 | signal in all pixels                                            |
| 45 | 3040283211406168192 | 7435594   | 11.90 | none                                                            |
| 46 | 3042753882750748544 | 169612691 | 14.18 | none                                                            |
| 47 | 3048912968935428352 | 318897046 | 12.73 | none                                                            |
| 48 | 3049743061554205440 | 125417316 | 10.74 | none                                                            |
| 49 | 3051988783994430848 | 753045874 | 16.71 | TYC 4827-3532-1                                                 |
| 50 | 3053792601542364032 | 753436363 | 18.94 | TYC 5396-3209-1                                                 |
| 51 | 3055092323061883392 | 753691638 | 18.76 | signal in all pixels                                            |
| 52 | 3055411494972465536 | 753750358 | 16.99 | TIC 5773753                                                     |
| 53 | 3056100918822449024 | 753851795 | 17.78 | HD 61235 (B8)                                                   |
| 54 | 3057227922540969728 | 177959638 | 13.10 | none                                                            |
| 55 | 3058814547877917056 | 10011123  | 12.55 | signal in all pixels                                            |
| 56 | 3060604003054132480 | 754603420 | 17.54 | signal in all pixels                                            |
| 57 | 3061152212676795520 | 178000482 | 15.05 | none                                                            |
| 58 | 3061214678683288576 | 754683833 | 17.70 | TIC 65674883                                                    |
| 59 | 3064721334796393216 | 50716894  | 14.18 | none                                                            |
| 60 | 3068776574200806912 | 73235712  | 15.95 | [MVD2012] 1141 (RR Lyr)                                         |
| 61 | 3070868532509787008 | 88860201  | 16.79 | none                                                            |
| 62 | 3076824204742509184 | 169112094 | 14.15 | none                                                            |
| 63 | 3084066893994173952 | 803902678 | 18.39 | TIC 73036564                                                    |
| 64 | 3088732087470746368 | 755428156 | 17.25 | signal in all pixels                                            |
| 65 | 3094972473091480192 | 452979074 | 15.73 | none                                                            |
| 66 | 3100012771834172160 | 710884361 | 16.78 | TIC 25699555                                                    |
| 67 | 3109770044180467200 | 757141728 | 17.47 | no signal in individual pixels                                  |
| 68 | 3110019525940805248 | 757187697 | 18.05 | no signal in individual pixels                                  |
| 69 | 3111017607617553792 | 757344922 | 17.66 | TIC 51066424                                                    |
| 70 | 3116446484938378880 | 758269982 | 18.25 | TIC 291962592                                                   |
| 71 | 3123004865638910208 | 232294383 | 16.39 | no signal in individual pixels                                  |
| 72 | 3127189224638386304 | 758556337 | 18.98 | TIC 234117193                                                   |
| 73 | 3128297777176229120 | 237726623 | 10.85 | ATO J103.9600+04.4495 (V)                                       |
| 74 | 3137171179606092416 | 759620247 | 17.97 | TIC 280225751                                                   |
| 75 | 3142054488704780288 | 234479694 | 14.51 | none                                                            |
| 76 | 3142605374093836800 | 760113062 | 18.56 | HD 58406 (A2)                                                   |
| 77 | 3153112448945566592 | 760644094 | 17.53 | no signal in individual pixels                                  |
| 78 | 3154801672464733440 | 264749962 | 15.24 | none                                                            |
| 79 | 3155186711990330624 | 264415506 | 13.94 | none                                                            |
| 80 | 3155418640221805696 | 207335489 | 10.61 | none                                                            |
| 81 | 3155495876617870336 | 760951300 | 18.88 | ASAS J072708+0916.6 (EB)                                        |
| 82 | 3157513897067140736 | 235515253 | 12.69 | TIC 235515258                                                   |
| 83 | 3161668397457008896 | 234401615 | 12.21 | none                                                            |
| 84 | 3163190946185170816 | 761800223 | 18.02 | 115.74 $\mu$ Hz+harmonics: none;<br>other peaks: TYC 772-1061-1 |
| 85 | 3163565604772130560 | 247054333 | 15.67 | none                                                            |
| 86 | 3204352783173513728 | 671960065 | 17.95 | none                                                            |
| 87 | 3210749947983249408 | 50620873  | 13.99 | none                                                            |



|     |                     |            |       |                                      |
|-----|---------------------|------------|-------|--------------------------------------|
| 88  | 3224457933106833920 | 220078773  | 16.65 | CRTS J053658.0+035420 (EB)           |
| 89  | 3236668044094291584 | 713270642  | 18.81 | ASAS J053342+0504.3 (EB)             |
| 90  | 3238322194915497600 | 455004085  | 12.87 | none                                 |
| 91  | 3280760148290124544 | 449100981  | 16.84 | none                                 |
| 92  | 3297832265335277824 | 356734609  | 16.15 | none                                 |
| 93  | 3300006785800948864 | 673411302  | 18.55 | CRTS J042449.8+103700 (EB)           |
| 94  | 3331584209996218240 | 167173528  | 10.45 | none                                 |
| 95  | 3335782905601559808 | 80666246   | 14.19 | none                                 |
| 96  | 3341803483380657152 | 140376343  | 15.18 | none                                 |
| 97  | 3351616560237148800 | 202053533  | 10.90 | none                                 |
| 98  | 3351799354044509312 | 387148310  | 14.71 | none                                 |
| 99  | 3368844460038497024 | 438226559  | 11.67 | none                                 |
| 100 | 3389962028254401024 | 302759005  | 12.80 | none                                 |
| 101 | 3459702504615640704 | 165424499  | 15.65 | UNSW-V 128 (PulsV*)                  |
| 102 | 3463190189858515328 | 107116449  | 12.94 | none                                 |
| 103 | 3464526440083406336 | 900956625  | 16.35 | no signal in individual pixels       |
| 104 | 3465428932971383296 | 901002130  | 16.94 | no signal in individual pixels       |
| 105 | 3467271989337490176 | 142209224  | 13.11 | none                                 |
| 106 | 3498412078485447552 | 9523440    | 16.30 | none                                 |
| 107 | 3531600532027961728 | 901552390  | 17.28 | CRTS J112218.7-272328 (PulsV*delSct) |
| 108 | 3544298482579656704 | 386680925  | 14.27 | -                                    |
| 109 | 3753760906575421312 | 334774940  | 12.39 | none                                 |
| 110 | 3836891579134516096 | 344891958  | 13.71 | no signal in individual pixels       |
| 111 | 4035430054473947648 | 1552130379 | 18.58 | NW CrA (RR Lyr)                      |
| 112 | 4035432970746984064 | 1552137492 | 17.78 | VVV J180356.13-400120.6 (RR Lyr)     |
| 113 | 4035494852634865664 | 1552304995 | 16.78 | TIC 326268416                        |
| 114 | 4035504512081944320 | 326764721  | 15.19 | no signal in individual pixels.      |
| 115 | 4035547633505015424 | 1401445125 | 17.25 | none                                 |
| 116 | 4035596969804831872 | 1401591140 | 17.75 | signal in all pixels                 |
| 117 | 4035685381692710144 | 1552399101 | 17.93 | no signal in individual pixels       |
| 118 | 4035753512743761280 | 1401921072 | 18.40 | no signal in individual pixels       |
| 119 | 4035812684512077568 | 1552606319 | 18.80 | HD 164821 (ApSi)                     |
| 120 | 4035881885054150656 | 1552781619 | 16.76 | no signal in individual pixels       |
| 121 | 4035893807903676928 | 1552817885 | 18.56 | no signal in individual pixels       |
| 122 | 4035963042729253760 | 1553002580 | 18.71 | TIC 330361794                        |
| 123 | 4035979501052938368 | 1553044292 | 18.51 | -                                    |
| 124 | 4035983826073072896 | 1553055422 | 17.71 | TIC 331123166                        |
| 125 | 4036080033345293184 | 1553336060 | 18.07 | no signal in individual pixels       |
| 126 | 4036085947593131392 | 327530783  | 14.99 | none                                 |
| 127 | 4036097556802437120 | 1553394005 | 18.22 | no signal in individual pixels       |
| 128 | 4036122368854810368 | 1553479446 | 18.19 | VVV J180457.98-383144.8 (RR Lyr)     |
| 129 | 4036149994109534592 | 1553574306 | 18.12 | no signal in individual pixels       |
| 130 | 4036188030360075776 | 1553721154 | 18.91 | FI CrA (RR Lyr)                      |
| 131 | 4036371408222958720 | 1402053616 | 18.61 | no signal in individual pixels       |
| 132 | 4036382948815373056 | 1402096286 | 18.22 | HD 162727 (RotV*alf2CVn)             |
| 133 | 4036425490484442368 | 1402244525 | 18.32 | no signal in individual pixels       |



|     |                     |            |       |                                                  |
|-----|---------------------|------------|-------|--------------------------------------------------|
| 134 | 4036508366135605248 | 1402553784 | 18.37 | TIC 112582374                                    |
| 135 | 4036925630798513664 | 1554364389 | 18.59 | no signal in individual pixels                   |
| 136 | 4037072548747347456 | 1554698949 | 17.86 | TIC 326580683                                    |
| 137 | 4037295891419329152 | 1404992031 | 18.88 | OGLE BLG-RRLYR-32416 (RR Lyr)                    |
| 138 | 4037614371800103936 | 1555926348 | 16.79 | -                                                |
| 139 | 4037726281455166336 | 1556209354 | 18.54 | V2743 Sgr (RR Lyr)                               |
| 140 | 4037855817685474944 | 1556644020 | 18.92 | none                                             |
| 141 | 4037922338167472512 | 1556886513 | 17.59 | -                                                |
| 142 | 4037933573728126208 | 1556924444 | 18.83 | TIC 332183980                                    |
| 143 | 4037946110752316288 | 1556965429 | 18.02 | no signal in individual pixels                   |
| 144 | 4037947111474332800 | 1556968636 | 18.79 | VVV J181333.94-362436.3 (RR Lyr)                 |
| 145 | 4037949924682971136 | 1556977464 | 17.59 | no signal in individual pixels                   |
| 146 | 4037958587636998528 | 1557007082 | 18.45 | TIC 332192081                                    |
| 147 | 4038147291340920192 | 1557578483 | 18.52 | V2854 Sgr (RR Lyr)                               |
| 148 | 4038187423465706496 | 1557679873 | 18.63 | no signal in individual pixels                   |
| 149 | 4038241230835885440 | 1557802210 | 19.00 | no signal in individual pixels                   |
| 150 | 4038323930448123648 | 1558012861 | 18.38 | signal in all pixels                             |
| 151 | 4038354411802116608 | 1558110935 | 18.69 | no signal in individual pixels                   |
| 152 | 4038482500636483200 | 1558513990 | 18.30 | no signal in individual pixels                   |
| 153 | 4038598881417360000 | 1558887210 | 18.59 | V705 Sgr (EB)                                    |
| 154 | 4038830878347472256 | 1559862810 | 18.79 | none                                             |
| 155 | 4039236873001321472 | 1561697475 | 18.69 | HD 321392 (A0)                                   |
| 156 | 4039258107336798976 | 1561786826 | 18.72 | no signal in individual pixels                   |
| 157 | 4039334106745707008 | 1562101896 | 17.92 | no signal in individual pixels                   |
| 158 | 4040405241583808896 | 1408448635 | 15.21 | signal in all pixels                             |
| 159 | 4042163871810793600 | 1564372072 | 13.95 | none                                             |
| 160 | 4044267310456915328 | 1569088281 | 16.83 | signal in all pixels                             |
| 161 | 4044583896814458496 | 1569870934 | 18.16 | TIC 64501119                                     |
| 162 | 4044587852483690496 | 1569884641 | 18.88 | no signal in individual pixels                   |
| 163 | 4044733572133754240 | 1570330815 | 18.67 | VVV J182059.77-333350.6 (RR Lyr)                 |
| 164 | 4044733847009004288 | 1570331728 | 18.08 | no signal in individual pixels                   |
| 165 | 4044757860173080064 | 1570409464 | 17.24 | TIC 1572480613                                   |
| 166 | 4044790673714836736 | 1570505846 | 17.91 | signal in all pixels                             |
| 167 | 4044834344947358208 | 1570598064 | 17.70 | signal in all pixels                             |
| 168 | 4044838300592702336 | 1570605971 | 18.78 | V2560 Sgr (RR Lyr)                               |
| 169 | 4044926673883075968 | 1570796204 | 18.17 | signal in all pixels                             |
| 170 | 4045407607115907200 | 1572081687 | 18.83 | V2979 Sgr (RR Lyr)                               |
| 171 | 4045478113352304512 | 1572362317 | 17.45 | V2898 Sgr (EB)                                   |
| 172 | 4045542056834007168 | 1572601998 | 18.37 | TIC 64238011                                     |
| 173 | 4045574595458610304 | 1572719068 | 18.69 | -                                                |
| 174 | 4045599781165667840 | 1572822653 | 16.08 | Gaia EDR3 4045599742451867136 (RR Lyr candidate) |
| 175 | 4045690765727858816 | 1573185473 | 18.52 | no signal in individual pixels                   |
| 176 | 4045802778452674176 | 1573672780 | 18.51 | no signal in individual pixels                   |
| 177 | 4045894587741284096 | 1574041872 | 18.69 | OGLE BLG-ECL-394209 (EB)                         |
| 178 | 4046287250869543808 | 1575483033 | 17.56 | signal in all pixels                             |



|     |                     |            |       |                                |
|-----|---------------------|------------|-------|--------------------------------|
| 179 | 4046523955036858368 | 405191890  | 16.12 | TIC 405191861                  |
| 180 | 4046527803288414976 | 1576395688 | 18.84 | -                              |
| 181 | 4046542745494717824 | 1576425868 | 18.71 | TIC 273001069                  |
| 182 | 4046561750722585984 | 1576465525 | 18.69 | V3521 Sgr (RR Lyr)             |
| 183 | 4046615386295719040 | 1576586722 | 18.28 | no signal in individual pixels |
| 184 | 4046812744324108800 | 1577014099 | 18.14 | signal in all pixels           |
| 185 | 4047039385468392448 | 1577619106 | 18.78 | signal in all pixels           |
| 186 | 4047339444749947776 | 1577855225 | 17.78 | no signal in individual pixels |
| 187 | 4047686997812881152 | 1578639977 | 18.71 | signal in all pixels           |
| 188 | 4047760871207790080 | 1578894919 | 17.90 | no signal in individual pixels |
| 189 | 4047856253895905792 | 1579199348 | 18.81 | -                              |
| 190 | 4047904593728818432 | 1579368204 | 17.73 | TIC 1579368307                 |
| 191 | 4049002219928777856 | 1583397261 | 18.80 | OGLE BLG-RRLYR-34994 (RR Lyr)  |
| 192 | 4049392031146869248 | 1585230166 | 18.06 | OGLE BLG526.29 26706 (RR Lyr)  |
| 193 | 4049758512074496256 | 1586950368 | 18.83 | OGLE BLG-RRLYR-35896 (RR Lyr)  |
| 194 | 4651851491766500608 | 280046882  | 14.74 | no signal in individual pixels |
| 195 | 4675773188253643648 | 38813070   | 15.43 | none                           |
| 196 | 4676030027297506432 | 38587008   | 14.21 | none                           |
| 197 | 4679132574232217216 | 358290394  | 16.82 | none                           |
| 198 | 4684361812878040192 | 180791583  | 14.89 | none                           |
| 199 | 4685494589034397056 | 180793878  | 16.73 | none                           |
| 200 | 4692223531471453824 | 52256144   | 16.62 | none                           |
| 201 | 4692540804999269376 | 615617106  | 17.04 | TIC 52153898                   |
| 202 | 4707501790999568128 | 615772150  | 18.32 | no signal in individual pixels |
| 203 | 4719018973437787648 | 231004822  | 15.20 | signal in all pixels           |
| 204 | 4737093845086555392 | 200767936  | 13.25 | none                           |
| 205 | 4747210309839466752 | 650797741  | 18.53 | signal in all pixels           |
| 206 | 4751122681448407680 | 650843770  | 18.01 | none                           |
| 207 | 4765026280860205440 | 734488865  | 18.27 | no signal in individual pixels |
| 208 | 4777242988915707776 | 685303558  | 18.54 | no signal in individual pixels |
| 209 | 4777378297565864320 | 685306000  | 18.83 | no signal in individual pixels |
| 210 | 4794410458529805440 | 452376397  | 16.27 | none                           |
| 211 | 4797703702012277120 | 685545073  | 17.14 | no signal in individual pixels |
| 212 | 4804695423438691200 | 734907771  | 15.26 | none                           |
| 213 | 4818077721196079232 | 685708760  | 17.65 | no signal in individual pixels |
| 214 | 4819197573787862016 | 685734472  | 18.44 | CI* NGC 1851 PML 41 (RR Lyr)   |
| 215 | 4825483924145787648 | 685810468  | 18.76 | TIC 1527210                    |
| 216 | 4832374396013713152 | 206412692  | 15.70 | none                           |
| 217 | 4834640970515267968 | 101102117  | 15.47 | none                           |
| 218 | 4858847646713152128 | 651125907  | 17.28 | no signal in individual pixels |
| 219 | 4865965507034625024 | 7739368    | 15.71 | no signal in individual pixels |
| 220 | 4909690606274233344 | 631615853  | 18.74 | signal in all pixels           |
| 221 | 4932663497284027776 | 382525144  | 15.62 | none                           |
| 222 | 4953527726852147328 | 91635434   | 14.57 | none                           |
| 223 | 5091939988633728640 | 139680713  | 11.76 | none                           |
| 224 | 5153423785504601216 | 98758637   | 13.58 | none                           |



|     |                     |           |       |                                                             |
|-----|---------------------|-----------|-------|-------------------------------------------------------------|
| 225 | 5159571498612745344 | 441499552 | 14.77 | none                                                        |
| 226 | 5190966433940608000 | 903876014 | 18.96 | TIC 383260696                                               |
| 227 | 5191289694657338880 | 369894636 | 13.20 | none                                                        |
| 228 | 5193984254058575616 | 278183255 | 16.12 | no signal in individual pixels                              |
| 229 | 5195578335465624064 | 842640177 | 17.78 | no signal in individual pixels                              |
| 230 | 5198995102206653952 | 904070333 | 17.45 | signal in all pixels                                        |
| 231 | 5199818468915025024 | 904138607 | 16.71 | 2MASS J11110663-7917358 (V);<br>2MASS J11112084-7917101 (V) |
| 232 | 5206159008877165184 | 843206897 | 18.79 | TIC 453363852                                               |
| 233 | 5206820365117740288 | 278140516 | 16.14 | no signal in individual pixels                              |
| 234 | 5210030045718111104 | 804723852 | 18.33 | TIC 272472682                                               |
| 235 | 5218949490203157248 | 452385021 | 13.71 | TIC 452385022                                               |
| 236 | 5219079541812683264 | 805057675 | 17.46 | none                                                        |
| 237 | 5220931188111998080 | 805184004 | 17.75 | TIC 287430039                                               |
| 238 | 5222544201732728320 | 805347551 | 17.30 | signal in all pixels                                        |
| 239 | 5224061459059273600 | 805549787 | 17.32 | signal in all pixels                                        |
| 240 | 5224132553657682688 | 302525114 | 13.03 | none                                                        |
| 241 | 5226895901258861696 | 454755425 | 16.26 | signal in all pixels                                        |
| 242 | 5227185034156035072 | 905021054 | 18.56 | no signal in individual pixels                              |
| 243 | 5228029016713146240 | 905301591 | 17.31 | no signal in individual pixels                              |
| 244 | 5228454390274972032 | 905471181 | 17.85 | TYC 9229-1045-1                                             |
| 245 | 5228959714643856768 | 449492139 | 12.50 | none                                                        |
| 246 | 5230267755524822528 | 843699281 | 18.80 | no signal in individual pixels                              |
| 247 | 5230269787048223616 | 453936887 | 15.27 | none                                                        |
| 248 | 5230640902282702336 | 843801810 | 18.41 | no signal in individual pixels                              |
| 249 | 5231780756547275264 | 906040170 | 17.49 | signal in all pixels                                        |
| 250 | 5234945013581534592 | 296047888 | 15.06 | no signal in individual pixels.                             |
| 251 | 5235000779437867776 | 295386806 | 15.27 | TIC 295386839                                               |
| 252 | 5235726938155549312 | 296799532 | 15.84 | signal in all pixels                                        |
| 253 | 5235795893834257024 | 908169448 | 18.86 | TIC 392616391                                               |
| 254 | 5236657842232619264 | 909318010 | 17.49 | no signal in individual pixels                              |
| 255 | 5237711453552382208 | 910458858 | 17.99 | signal in all pixels                                        |
| 256 | 5237994783954394240 | 910646470 | 18.62 | no signal in individual pixels                              |
| 257 | 5239201218787130752 | 844369546 | 18.37 | no signal in individual pixels                              |
| 258 | 5239206304032533504 | 844373125 | 18.55 | no signal in individual pixels                              |
| 259 | 5240462294234795392 | 912664884 | 16.14 | no signal in individual pixels                              |
| 260 | 5242349807763697280 | 844585854 | 18.50 | V637 Car (RR Lyr)                                           |
| 261 | 5242837651629887488 | 372372750 | 13.88 | no signal in individual pixels                              |
| 262 | 5244655586727634176 | 845173186 | 18.51 | no signal in individual pixels                              |
| 263 | 5244976300535071488 | 845291963 | 18.07 | signal in all pixels                                        |
| 264 | 5245799078820115200 | 845700942 | 18.49 | no signal in individual pixels                              |
| 265 | 5246014136421865856 | 845780091 | 16.86 | none                                                        |
| 266 | 5246166384423306624 | 845847767 | 17.48 | signal in all pixels                                        |
| 267 | 5246711329872492544 | 304082289 | 13.48 | no signal in individual pixels                              |
| 268 | 5247119699663365888 | 846234731 | 17.97 | no signal in individual pixels                              |
| 269 | 5247284488969176704 | 370558231 | 15.47 | none                                                        |



|     |                     |           |       |                                |
|-----|---------------------|-----------|-------|--------------------------------|
| 270 | 5247855066784344448 | 805597946 | 16.80 | none                           |
| 271 | 5249439600477740160 | 846666380 | 18.80 | no signal in individual pixels |
| 272 | 5249872223955673088 | 846910599 | 17.32 | no signal in individual pixels |
| 273 | 5250190940576295680 | 847076196 | 18.71 | no signal in individual pixels |
| 274 | 5251102263917170048 | 847508238 | 18.17 | signal in all pixels           |
| 275 | 5251639169189308800 | 847902915 | 17.71 | no signal in individual pixels |
| 276 | 5252255376741428608 | 848616007 | 17.83 | signal in all pixels           |
| 277 | 5252355878981408768 | 848739398 | 18.23 | TIC 376414794                  |
| 278 | 5252398794287406208 | 848776574 | 17.31 | no signal in individual pixels |
| 279 | 5253000025309142144 | 849389551 | 18.36 | TIC 377576240                  |
| 280 | 5253245693140142080 | 849738256 | 17.62 | TIC 375746688                  |
| 281 | 5253315065450598656 | 849833337 | 17.90 | no signal in individual pixels |
| 282 | 5253356438892124032 | 849895099 | 17.47 | signal in all pixels           |
| 283 | 5253644472239997312 | 390094921 | 15.61 | TIC 390094806                  |
| 284 | 5253918873456326016 | 460863334 | 12.26 | TIC 460863280.                 |
| 285 | 5254015626152420224 | 915504882 | 17.66 | TIC 390685381                  |
| 286 | 5254701794448754304 | 378325642 | 15.29 | TIC 378325663                  |
| 287 | 5255758047127028864 | 852561440 | 18.86 | signal in all pixels           |
| 288 | 5255832397304667264 | 852628533 | 17.78 | TIC 270086297                  |
| 289 | 5256673454977322624 | 853582964 | 17.91 | signal in all pixels           |
| 290 | 5257714525010318208 | 444537148 | 14.97 | HD 302393 (F0)                 |
| 291 | 5258319630042489088 | 462170252 | 16.56 | none                           |
| 292 | 5258531977522961536 | 854992353 | 16.93 | no signal in individual pixels |
| 293 | 5260463682011363584 | 142109447 | 15.55 | no signal in individual pixels |
| 294 | 5263888695091870976 | 271554913 | 15.96 | no signal in individual pixels |
| 295 | 5270326537535726208 | 805857938 | 18.24 | no signal in individual pixels |
| 296 | 5271448284210652928 | 307027969 | 14.49 | none                           |
| 297 | 5271674229551996544 | 805944182 | 16.66 | none                           |
| 298 | 5272113553168105984 | 805997069 | 18.43 | no signal in individual pixels |
| 299 | 5273984617016821760 | 765068821 | 17.66 | no signal in individual pixels |
| 300 | 5276947934000401536 | 806375852 | 18.53 | no signal in individual pixels |
| 301 | 5278070191772384512 | 806506187 | 18.40 | no signal in individual pixels |
| 302 | 5279058961961831040 | 765184738 | 17.65 | no signal in individual pixels |
| 303 | 5279289550165529728 | 765189918 | 16.93 | TIC 176932559                  |
| 304 | 5280144768350837888 | 736208356 | 18.30 | no signal in individual pixels |
| 305 | 5281283828034802048 | 765250340 | 18.57 | no signal in individual pixels |
| 306 | 5282634371914454912 | 349408306 | 16.05 | none                           |
| 307 | 5285464377404208128 | 167811155 | 16.59 | TIC 167811160                  |
| 308 | 5285924209485874560 | 765393972 | 17.73 | signal in all pixels           |
| 309 | 5286214175614534400 | 765410266 | 17.24 | CRTS J064752.4-635158 (RR Lyr) |
| 310 | 5288693711775341312 | 349572491 | 15.01 | none                           |
| 311 | 5288885232956603136 | 349784237 | 16.45 | none                           |
| 312 | 5290282162482108928 | 309293646 | 14.80 | none                           |
| 313 | 5290692589556889472 | 765648311 | 17.17 | TIC 410449364                  |
| 314 | 5291929437056010496 | 349682410 | 14.71 | none                           |
| 315 | 5293807609074450304 | 339961027 | 13.04 | none                           |



|     |                     |           |       |                                 |
|-----|---------------------|-----------|-------|---------------------------------|
| 316 | 5294081726770000128 | 765841903 | 16.52 | no signal in individual pixels  |
| 317 | 5298391060742148608 | 807305254 | 16.44 | TIC 357120271                   |
| 318 | 5298764001347869184 | 359451530 | 16.25 | signal in all pixels            |
| 319 | 5299166560047415936 | 855685073 | 18.23 | no signal in individual pixels  |
| 320 | 5299279290038392960 | 855759088 | 17.36 | no signal in individual pixels  |
| 321 | 5299425426314526336 | 358985529 | 12.48 | TIC 358985523                   |
| 322 | 5299601893616875392 | 855955042 | 17.71 | -                               |
| 323 | 5299753007755839488 | 807528961 | 18.75 | no signal in individual pixels  |
| 324 | 5300023251392076032 | 807646804 | 18.44 | no signal in individual pixels  |
| 325 | 5300050700520510336 | 807659239 | 17.56 | no signal in individual pixels  |
| 326 | 5300162339621000192 | 384718210 | 16.74 | none                            |
| 327 | 5300518031634067456 | 807849536 | 17.22 | none                            |
| 328 | 5300536409791626240 | 807860050 | 18.80 | no signal in individual pixels  |
| 329 | 5301260232029153152 | 354940751 | 12.20 | no signal in individual pixels  |
| 330 | 5302553502522498944 | 808374596 | 18.07 | no signal in individual pixels  |
| 331 | 5302635209984826496 | 121811003 | 13.74 | no signal in individual pixels  |
| 332 | 5303151769986558336 | 808565133 | 18.35 | no signal in individual pixels  |
| 333 | 5303768497247613568 | 808863275 | 18.03 | TIC 385004580                   |
| 334 | 5304155181733078272 | 122264219 | 15.18 | no signal in individual pixels. |
| 335 | 5304484515520209152 | 809229443 | 18.52 | no signal in individual pixels  |
| 336 | 5304725102407737472 | 809335210 | 17.41 | TIC 384032429                   |
| 337 | 5305593854040242048 | 856317213 | 18.46 | signal in all pixels            |
| 338 | 5307946881949072000 | 442750342 | 12.85 | none                            |
| 339 | 5310418270539764224 | 859084682 | 18.41 | no signal in individual pixels  |
| 340 | 5313049268735645312 | 299705972 | 16.24 | no signal in individual pixels  |
| 341 | 5315335286539670016 | 811435326 | 17.82 | no signal in individual pixels  |
| 342 | 5316701704614137472 | 811760100 | 17.27 | none                            |
| 343 | 5317230775863438464 | 812007039 | 18.81 | no signal in individual pixels  |
| 344 | 5317638767700229632 | 812247788 | 17.28 | no signal in individual pixels  |
| 345 | 5319789927839251584 | 139830503 | 15.61 | TIC 139830552                   |
| 346 | 5332775190225061504 | 321662350 | 15.44 | no signal in individual pixels  |
| 347 | 5333606627173404032 | 318667177 | 16.01 | none                            |
| 348 | 5336022219874953984 | 921255821 | 17.93 | HD 99416 (B2III)                |
| 349 | 5337006630678731776 | 467486257 | 14.41 | signal in all pixels            |
| 350 | 5340301145490047104 | 927605255 | 15.06 | TIC 307871938                   |
| 351 | 5340389724892633984 | 306375414 | 14.96 | no signal in individual pixels  |
| 352 | 5341565893098163328 | 268898738 | 15.80 | none                            |
| 353 | 5341632722785320320 | 929158789 | 16.62 | -                               |
| 354 | 5342226321623258112 | 929810893 | 18.96 | TIC 268256646                   |
| 355 | 5342575107324151808 | 267072776 | 15.83 | none                            |
| 356 | 5343990969037546112 | 931392032 | 18.32 | no signal in individual pixels  |
| 357 | 5344289275990539008 | 931580567 | 18.61 | signal in all pixels            |
| 358 | 5344290723406022656 | 376272707 | 15.19 | TIC 376272735                   |
| 359 | 5344630472499580928 | 931760369 | 18.22 | no signal in individual pixels  |
| 360 | 5345331235052723968 | 932150009 | 18.14 | no signal in individual pixels  |
| 361 | 5345407273152519040 | 932184276 | 18.65 | signal in all pixels            |



|     |                     |           |       |                                |
|-----|---------------------|-----------|-------|--------------------------------|
| 362 | 5345765546448222976 | 932329584 | 18.46 | no signal in individual pixels |
| 363 | 5346517578051379584 | 451639729 | 15.41 | no signal in individual pixels |
| 364 | 5346641410549392768 | 932984327 | 17.20 | no signal in individual pixels |
| 365 | 5347227965647133184 | 306247349 | 13.16 | none                           |
| 366 | 5348039989335089408 | 92167387  | 15.98 | none                           |
| 367 | 5348816004023739520 | 934131546 | 17.46 | HD 99641 (G3IV/V)              |
| 368 | 5352157793516577152 | 935475454 | 18.67 | signal in all pixels           |
| 369 | 5353771674747981056 | 458473363 | 15.89 | none                           |
| 370 | 5354100325613614336 | 861345064 | 12.51 | none                           |
| 371 | 5357218123978608512 | 863253270 | 17.99 | TIC 448119771                  |
| 372 | 5358583653013806720 | 864051305 | 17.77 | no signal in individual pixels |
| 373 | 5360762541457368448 | 303494766 | 15.46 | signal in all pixels           |
| 374 | 5363685932410946304 | 938089081 | 18.78 | signal in all pixels           |
| 375 | 5365038198575553536 | 864760271 | 18.74 | TYC 8188-4047-1                |
| 376 | 5365758103812937344 | 103064270 | 16.49 | TIC 103064288                  |
| 377 | 5366666433556604800 | 938193456 | 18.54 | signal in all pixels           |
| 378 | 5366900049716301568 | 146719029 | 15.54 | none                           |
| 379 | 5367809620710374144 | 865242836 | 17.14 | no signal in individual pixels |
| 380 | 5368563331636796032 | 938377350 | 18.50 | signal in all pixels           |
| 381 | 5368624595048917760 | 938404965 | 18.19 | TIC 389092347                  |
| 382 | 5369134321767811072 | 938591664 | 18.15 | TIC 400864696                  |
| 383 | 5369149478711902464 | 938597068 | 16.58 | TIC 389094756                  |
| 384 | 5370607637290164864 | 332163220 | 15.33 | no signal in individual pixels |
| 385 | 5371709279219789440 | 939279077 | 17.60 | none                           |
| 386 | 5374213142070700288 | 939807244 | 18.42 | no signal in individual pixels |
| 387 | 5374644253706949632 | 162583323 | 13.69 | none                           |
| 388 | 5375190053851090688 | 939980818 | 18.44 | no signal in individual pixels |
| 389 | 5375311794705734528 | 163144312 | 11.39 | none                           |
| 390 | 5376389109940771328 | 940146008 | 16.95 | no signal in individual pixels |
| 391 | 5377737862811245440 | 940326628 | 18.67 | TIC 61986506                   |
| 392 | 5378260611871280256 | 61876577  | 11.26 | none                           |
| 393 | 5387205143261650304 | 178713476 | 15.79 | no signal in individual pixels |
| 394 | 5387711708884117120 | 147620145 | 15.05 | none                           |
| 395 | 5388173847365565440 | 941392387 | 18.73 | TIC 941392385                  |
| 396 | 5388932441668451072 | 178615544 | 13.24 | none                           |
| 397 | 5390228834596755200 | 941603746 | 17.47 | none                           |
| 398 | 5392305812062637440 | 105994999 | 15.92 | none                           |
| 399 | 5395799063581860224 | 152021686 | 15.41 | none                           |
| 400 | 5402896204979498368 | 57185765  | 16.11 | TIC 57185763                   |
| 401 | 5407149012888838528 | 867241796 | 17.37 | TIC 259660452                  |
| 402 | 5407274838253246720 | 867297951 | 17.82 | -                              |
| 403 | 5407636367110433408 | 867442832 | 18.27 | TIC 375435567                  |
| 404 | 5407689938244160640 | 867461747 | 18.24 | signal in all pixels           |
| 405 | 5408609920233585920 | 867830964 | 17.73 | TIC 36386815                   |
| 406 | 5408748385684471424 | 867877236 | 17.95 | signal in all pixels           |
| 407 | 5411333062643264128 | 869009101 | 17.97 | signal in all pixels           |



|     |                     |           |       |                                |
|-----|---------------------|-----------|-------|--------------------------------|
| 408 | 5413343455236193024 | 102207188 | 12.23 | none                           |
| 409 | 5413498314580660352 | 102291871 | 14.79 | none                           |
| 410 | 5413589638460478720 | 869764492 | 18.66 | SV* HV 10335 (RR Lyr)          |
| 411 | 5415345077494077440 | 870183237 | 17.71 | -                              |
| 412 | 5415837937878684672 | 870272017 | 17.04 | signal in all pixels           |
| 413 | 5415884319224886528 | 870279987 | 17.61 | signal in all pixels           |
| 414 | 5416091856344970880 | 102332341 | 15.55 | none                           |
| 415 | 5416177790051166464 | 870329007 | 17.58 | no signal in individual pixels |
| 416 | 5416420228064531328 | 870362582 | 18.97 | signal in all pixels           |
| 417 | 5416786571595520768 | 870414976 | 17.57 | TIC 101915841                  |
| 418 | 5417595953892026240 | 73435422  | 14.79 | no signal in individual pixels |
| 419 | 5418573351010496640 | 870706534 | 17.61 | no signal in individual pixels |
| 420 | 5418658593222906624 | 870720185 | 16.64 | no signal in individual pixels |
| 421 | 5418855543243041024 | 870752612 | 18.06 | TIC 286999395                  |
| 422 | 5419514773481634944 | 45237026  | 16.55 | none                           |
| 423 | 5421695139398941440 | 287043517 | 13.94 | none                           |
| 424 | 5430272017292658816 | 3589671   | 15.25 | none                           |
| 425 | 5430326305680773248 | 816914609 | 16.35 | TIC 3354992                    |
| 426 | 5432279485003926144 | 872598873 | 18.24 | TIC 44692620                   |
| 427 | 5433010247919403136 | 872711043 | 16.56 | TIC 44306559                   |
| 428 | 5434342581134109312 | 872872614 | 17.91 | CRTS J100644.1-354500 (RotV)   |
| 429 | 5438018690883729152 | 873312330 | 18.03 | signal in all pixels           |
| 430 | 5444891158252124544 | 73544285  | 14.66 | none                           |
| 431 | 5449404924062965632 | 942597272 | 17.80 | none                           |
| 432 | 5449580158729020928 | 48942631  | 15.48 | none                           |
| 433 | 5449580266104595712 | 48942634  | 15.62 | Gaia EDR3 5449580158729020928  |
| 434 | 5450950360672474368 | 48768301  | 15.12 | CRTS J104924.8-320500 (EB)     |
| 435 | 5452257130241574272 | 942728880 | 18.53 | no signal in individual pixels |
| 436 | 5453213911516139776 | 363444403 | 14.23 | none                           |
| 437 | 5454691964381612928 | 942815867 | 18.15 | no signal in individual pixels |
| 438 | 5461231584667801856 | 71671894  | 16.65 | none                           |
| 439 | 5464629556631919104 | 22148636  | 16.49 | no signal in individual pixels |
| 440 | 5465087125267504384 | 22234651  | 14.56 | none                           |
| 441 | 5478232989368582144 | 150439866 | 16.27 | TYC 8898-7-1 (EB)              |
| 442 | 5479385037036573440 | 349091180 | 15.76 | none                           |
| 443 | 5481999057212019456 | 260653949 | 14.94 | none                           |
| 444 | 5484435192726246528 | 766162694 | 16.74 | no signal in individual pixels |
| 445 | 5484959767147218944 | 279216015 | 14.08 | no signal in individual pixels |
| 446 | 5486042579942991104 | 339772356 | 16.04 | none                           |
| 447 | 5486545533496209792 | 766285566 | 18.69 | CRTS J071213.4-582653 (EB)     |
| 448 | 5487114393324146816 | 766319960 | 17.27 | TIC 339768609                  |
| 449 | 5493350754558065024 | 766897399 | 18.16 | TIC 766897407                  |
| 450 | 5493446656886309504 | 267457227 | 14.40 | none                           |
| 451 | 5505576194285665280 | 767305478 | 17.12 | none                           |
| 452 | 5506584613949825280 | 767416301 | 18.97 | TIC 445388907                  |
| 453 | 5507148358474299520 | 767482214 | 17.37 | none                           |



|     |                     |           |       |                                                                               |
|-----|---------------------|-----------|-------|-------------------------------------------------------------------------------|
| 454 | 5510484998308765824 | 59757289  | 16.32 | none                                                                          |
| 455 | 5511237854536885632 | 60500411  | 14.93 | TIC 60500408                                                                  |
| 456 | 5512856125193586176 | 238373107 | 11.88 | none                                                                          |
| 457 | 5516314196650079744 | 82126345  | 16.04 | none                                                                          |
| 458 | 5518792461496084096 | 818322329 | 17.98 | no signal in individual pixels                                                |
| 459 | 5521176786824872192 | 81427796  | 14.26 | 2MASS J08123971-4331202 (YSO)                                                 |
| 460 | 5521425718824174464 | 819223214 | 18.27 | no signal in individual pixels                                                |
| 461 | 5522048493390273792 | 141745052 | 16.87 | none                                                                          |
| 462 | 5527134731095076352 | 82469453  | 14.11 | none                                                                          |
| 463 | 5531436879575891200 | 143732676 | 15.08 | TIC 143732705                                                                 |
| 464 | 5531498108631141760 | 143496219 | 15.56 | none                                                                          |
| 465 | 5532951078890956800 | 821414494 | 18.36 | no signal in individual pixels                                                |
| 466 | 5536165466764699264 | 123109867 | 15.66 | signal in all pixels                                                          |
| 467 | 5541063378756070144 | 134320640 | 15.67 | none                                                                          |
| 468 | 5543711002760540544 | 55513753  | 15.92 | TIC 55513750                                                                  |
| 469 | 5545705001452362496 | 418972243 | 14.54 | none                                                                          |
| 470 | 5547176903927857152 | 147528018 | 14.08 | none                                                                          |
| 471 | 5551496124891134592 | 770639577 | 18.95 | TIC 237974015                                                                 |
| 472 | 5553638939909612416 | 238923481 | 12.55 | none                                                                          |
| 473 | 5554340973787678720 | 737807060 | 18.79 | CRTS J061236.6-473124 (EB)                                                    |
| 474 | 5556042953365726592 | 156933503 | 14.86 | none                                                                          |
| 475 | 5560591014496851584 | 59896227  | 15.88 | none                                                                          |
| 476 | 5563724450835110144 | 156809481 | 15.57 | none                                                                          |
| 477 | 5563978742961343232 | 156843549 | 11.69 | CRTS J065449.0-400626 (EB)                                                    |
| 478 | 5565582591127646336 | 157451427 | 15.80 | none                                                                          |
| 479 | 5565971268488957952 | 771605262 | 17.01 | no signal in individual pixels                                                |
| 480 | 5566220544092375808 | 771636412 | 18.55 | no signal in individual pixels                                                |
| 481 | 5570524827173062656 | 147803573 | 15.58 | none                                                                          |
| 482 | 5571863070262844160 | 393320488 | 14.66 | none                                                                          |
| 483 | 5572008721193797632 | 393320233 | 13.26 | none                                                                          |
| 484 | 5575181121478415104 | 393454453 | 14.50 | none                                                                          |
| 485 | 5578307823308779520 | 771860682 | 18.64 | TIC 157307309                                                                 |
| 486 | 5579589265455174656 | 771992940 | 18.09 | none                                                                          |
| 487 | 5579855179769135616 | 96580348  | 16.72 | CRTS J065800.6-334409 (EB)                                                    |
| 488 | 5582784072586681600 | 53125314  | 15.01 | none                                                                          |
| 489 | 5585326792009677056 | 772399021 | 17.79 | no signal in individual pixels                                                |
| 490 | 5589960580683738880 | 773554411 | 18.96 | no signal in individual pixels                                                |
| 491 | 5594201263898894976 | 152683125 | 16.64 | TIC 152683130                                                                 |
| 492 | 5594391097148387712 | 151005205 | 16.89 | 49.65 $\mu$ Hz: none;<br>other signal: TYC 7123-1718-1                        |
| 493 | 5596703374413665664 | 154072020 | 13.81 | TIC 154072038                                                                 |
| 494 | 5596751409325049856 | 154909544 | 15.07 | none                                                                          |
| 495 | 5597879950620891264 | 154077803 | 13.24 | no signal in individual pixels                                                |
| 496 | 5601882864452671488 | 776741908 | 17.23 | no signal in individual pixels                                                |
| 497 | 5602330537486293504 | 127808778 | 14.38 | none                                                                          |
| 498 | 5602460520380593408 | 128337007 | 12.87 | 65.97 $\mu$ Hz: none;<br>31.25 $\mu$ Hz: ATO J118.0075-25.0650 (EB candidate) |



|     |                     |           |       |                                                  |
|-----|---------------------|-----------|-------|--------------------------------------------------|
| 499 | 5604235505787962624 | 777294186 | 18.40 | none                                             |
| 500 | 5605157583727723776 | 777517836 | 18.70 | Gaia EDR3 5605063648503377408 (RR Lyr candidate) |
| 501 | 5606037128612616576 | 231483009 | 15.37 | none                                             |
| 502 | 5606816922877511424 | 66340558  | 13.22 | ATO J109.2457-28.3647 (V)                        |
| 503 | 5607248786123936384 | 96587458  | 15.07 | none                                             |
| 504 | 5608801468341667840 | 778383608 | 18.65 | no signal in individual pixels                   |
| 505 | 5609358340921279744 | 64303358  | 14.47 | none                                             |
| 506 | 5610443936854458880 | 63475048  | 16.75 | HD 52618 (B9V)                                   |
| 507 | 5610452114472366208 | 63202939  | 15.24 | none                                             |
| 508 | 5610727198536681600 | 778822592 | 16.06 | TIC 63195379                                     |
| 509 | 5611300555191309824 | 63884928  | 11.71 | TIC 63884938                                     |
| 510 | 5611403668764166272 | 778986392 | 18.91 | no signal in individual pixels                   |
| 511 | 5611674977567099648 | 109931573 | 15.90 | no signal in individual pixels                   |
| 512 | 5615673351602576512 | 140535775 | 11.84 | TIC 140535818                                    |
| 513 | 5617301071183981056 | 781077205 | 18.38 | no signal in individual pixels                   |
| 514 | 5617655702343147136 | 781192259 | 18.13 | no signal in individual pixels                   |
| 515 | 5617876047041466752 | 412386553 | 11.51 | none                                             |
| 516 | 5620459624489278080 | 456652145 | 17.15 | no signal in individual pixels                   |
| 517 | 5624566613956874752 | 826825114 | 17.18 | TIC 18658764                                     |
| 518 | 5628726238245009792 | 186461402 | 16.09 | none                                             |
| 519 | 5629304100323516032 | 186976962 | 16.27 | TIC 186976949                                    |
| 520 | 5630711062890539648 | 827950411 | 17.32 | CRTS J091548.6-332630 (EB)                       |
| 521 | 5633416475669561216 | 875119468 | 17.65 | signal in all pixels                             |
| 522 | 5633654386793798016 | 189589633 | 15.47 | signal in all pixels                             |
| 523 | 5633681084310290688 | 875137158 | 17.48 | no signal in individual pixels                   |
| 524 | 5637827583177740800 | 828285146 | 18.78 | Gaia EDR3 5637827617537477504                    |
| 525 | 5639068107180896896 | 828499719 | 17.20 | TIC 47791970                                     |
| 526 | 5644919742422869632 | 287473982 | 12.41 | ATO J127.1262-28.7198 (EB candidate)             |
| 527 | 5645974345864728192 | 830331649 | 17.70 | CRTS J084558.2-273942 (EB)                       |
| 528 | 5647303827227273088 | 283497784 | 16.08 | none                                             |
| 529 | 5653015687046953856 | 2221045   | 16.21 | none                                             |
| 530 | 5653584856113899520 | 831206143 | 16.52 | TIC 941297                                       |
| 531 | 5661991584579213568 | 189642089 | 12.65 | none                                             |
| 532 | 5664376421004019200 | 875624496 | 18.22 | UCAC4 345-059549 (PulsV)                         |
| 533 | 5674617890780564480 | 875876976 | 17.83 | TYC 6588-537-1                                   |
| 534 | 5676281524888361600 | 875927603 | 18.90 | CRTS J092334.1-212113 (EB)                       |
| 535 | 5693771490724184832 | 831953467 | 17.08 | no signal in individual pixels                   |
| 536 | 5694405943289480192 | 156259914 | 16.92 | none                                             |
| 537 | 5695444668235526912 | 832437114 | 18.36 | none                                             |
| 538 | 5695725632118550784 | 258233590 | 14.42 | none                                             |
| 539 | 5695954738551356928 | 832527150 | 18.35 | no signal in individual pixels                   |
| 540 | 5696328748608315520 | 156264909 | 14.19 | none                                             |
| 541 | 5696337613421063040 | 832616218 | 18.90 | signal in all pixels                             |
| 542 | 5697958323614202752 | 154320905 | 12.36 | rho Pup (PulsV*delSct)                           |
| 543 | 5698111228755357184 | 154362255 | 13.94 | rho Pup (PulsV*delSct)                           |



|     |                     |            |       |                                                                                      |
|-----|---------------------|------------|-------|--------------------------------------------------------------------------------------|
| 544 | 5698268012249950720 | 782115272  | 17.54 | none                                                                                 |
| 545 | 5698291445592308224 | 129923314  | 14.40 | TIC 129923311                                                                        |
| 546 | 5698779044631002240 | 833171269  | 17.16 | no signal in individual pixels                                                       |
| 547 | 5698927100741737216 | 833215719  | 17.68 | no signal in individual pixels                                                       |
| 548 | 5702622559313845632 | 415341431  | 16.25 | none                                                                                 |
| 549 | 5703049032389637248 | 412893245  | 13.33 | none                                                                                 |
| 550 | 5706158103378655744 | 834204893  | 18.86 | no signal in individual pixels                                                       |
| 551 | 5706653609462271872 | 434415105  | 12.68 | no signal in individual pixels                                                       |
| 552 | 5709867924332995072 | 386435486  | 15.34 | TYC 6011-1986-1                                                                      |
| 553 | 5710601405970309504 | 128898027  | 14.06 | no signal in individual pixels                                                       |
| 554 | 5710627210133676416 | 142294213  | 13.25 | signal in all pixels                                                                 |
| 555 | 5710747297419335168 | 142841028  | 11.62 | none                                                                                 |
| 556 | 5711073268257108608 | 141929042  | 11.45 | none                                                                                 |
| 557 | 5713066476668938240 | 834750064  | 18.21 | no signal in individual pixels                                                       |
| 558 | 5714647329577757312 | 834986703  | 18.00 | signal in all pixels                                                                 |
| 559 | 5716059347328019712 | 141014907  | 14.30 | signal in all pixels                                                                 |
| 560 | 5718305061164380288 | 783826251  | 17.24 | no signal in individual pixels                                                       |
| 561 | 5718339631362116992 | 56541907   | 13.89 | none                                                                                 |
| 562 | 5718613547198076160 | 347101265  | 14.66 | none                                                                                 |
| 563 | 5718737001739477120 | 333708089  | 15.22 | none                                                                                 |
| 564 | 5719128565318352128 | 54275618   | 14.16 | TIC 54221871                                                                         |
| 565 | 5719825277727577984 | 218791808  | 15.95 | 68.98 $\mu$ Hz+harmonic: none;<br>81.25 $\mu$ Hz+harmonic: ATO J124.4930-17.9750 (V) |
| 566 | 5721142419640136576 | 835309448  | 17.60 | ATO J122.1425-16.6179 (EB candidate)                                                 |
| 567 | 5722771380477406720 | 409896363  | 14.03 | no signal in individual pixels                                                       |
| 568 | 5723707889504619392 | 835566304  | 18.03 | HD 72009 (A9V)                                                                       |
| 569 | 5724560354614681344 | 835672447  | 18.37 | ATO J121.2044-15.0215 (V)                                                            |
| 570 | 5725325064950852736 | 784154417  | 18.83 | no signal in individual pixels                                                       |
| 571 | 5725554175687361408 | 784175336  | 18.04 | TIC 54391224                                                                         |
| 572 | 5725626438516309632 | 784188056  | 17.57 | ATO J119.7165-14.3186 (candidate EB)                                                 |
| 573 | 5746111916389101312 | 876368336  | 18.58 | no signal in individual pixels                                                       |
| 574 | 5758065776742268544 | 60659496   | 15.34 | CRTS J091250.9-060923 (EB)                                                           |
| 575 | 5767544872645965440 | 451530230  | 15.41 | TIC 451530226                                                                        |
| 576 | 5771934226144030080 | 1104041117 | 16.74 | no signal in individual pixels                                                       |
| 577 | 5773909979818514560 | 1309527575 | 16.31 | no signal in individual pixels                                                       |
| 578 | 5778256074403636352 | 1104216937 | 17.59 | TIC 407221993                                                                        |
| 579 | 5780781064202713344 | 1205372466 | 17.09 | signal in all pixels                                                                 |
| 580 | 5782096153129640320 | 1205542525 | 16.90 | Gaia EDR3 5782095702151569792 (RR Lyr candidate)                                     |
| 581 | 5782415252021067520 | 426135737  | 13.82 | none                                                                                 |
| 582 | 5784814248951042688 | 269981028  | 16.69 | TIC 269981015                                                                        |
| 583 | 5786080194851644032 | 1003595250 | 18.37 | no signal in individual pixels                                                       |
| 584 | 5788454766310501760 | 954816608  | 17.41 | TIC 357784273                                                                        |
| 585 | 5788543685014228352 | 954832208  | 17.93 | no signal in individual pixels                                                       |
| 586 | 5790483670203047424 | 1004170731 | 18.06 | no signal in individual pixels                                                       |
| 587 | 5790692336892822784 | 1004227549 | 18.02 | HD 119034 (A3Vn)                                                                     |
| 588 | 5791375374134559232 | 395331816  | 11.49 | no signal in individual pixels                                                       |



|     |                     |            |       |                                |
|-----|---------------------|------------|-------|--------------------------------|
| 589 | 5792895964356495616 | 1105014050 | 18.00 | TIC 402513601                  |
| 590 | 5793332126880112256 | 1105095032 | 17.88 | signal in all pixels           |
| 591 | 5794445966509893376 | 1105473674 | 17.57 | TIC 426061785                  |
| 592 | 5795225387121705216 | 1105758734 | 18.70 | signal in all pixels           |
| 593 | 5795399316120688128 | 1105833452 | 17.49 | signal in all pixels           |
| 594 | 5795863821114045696 | 1106043510 | 18.65 | TIC 263349964                  |
| 595 | 5795877294427092992 | 1106050204 | 18.34 | none                           |
| 596 | 5796067338156065024 | 263352137  | 13.30 | none                           |
| 597 | 5796414229767021056 | 1004719662 | 18.99 | TIC 396648272                  |
| 598 | 5796595924070763648 | 1004792139 | 18.75 | signal in all pixels           |
| 599 | 5797130909493408000 | 1106335253 | 18.35 | TIC 258489335                  |
| 600 | 5797771679951039360 | 1005141638 | 18.50 | no signal in individual pixels |
| 601 | 5798969529149741440 | 1106776321 | 18.56 | no signal in individual pixels |
| 602 | 5799930777187394432 | 1107425811 | 18.96 | TYC 9257-1957-1                |
| 603 | 5800069182534948224 | 1107553189 | 17.40 | no signal in individual pixels |
| 604 | 5800232047667964672 | 1107696532 | 17.07 | TIC 260829757                  |
| 605 | 5800326124664001536 | 1107787932 | 18.39 | TIC 1107800063                 |
| 606 | 5800601174371223808 | 1108081480 | 17.93 | TYC 9032-826-1                 |
| 607 | 5800806027099401216 | 343448758  | 15.94 | signal in all pixels           |
| 608 | 5802262570771179648 | 1309862966 | 16.89 | no signal in individual pixels |
| 609 | 5802422820292199424 | 1309882690 | 18.80 | no signal in individual pixels |
| 610 | 5804157063664343040 | 1509140148 | 18.49 | no signal in individual pixels |
| 611 | 5804443035467670144 | 1310003642 | 18.62 | no signal in individual pixels |
| 612 | 5804655413010037504 | 1509171317 | 18.68 | no signal in individual pixels |
| 613 | 5804719768801499520 | 1509178835 | 18.74 | TIC 293578567                  |
| 614 | 5805200358463388288 | 1310114039 | 18.49 | no signal in individual pixels |
| 615 | 5805333334948752896 | 310507132  | 15.95 | HD 150995 (B8/9V)              |
| 616 | 5805971360931188736 | 1310206160 | 17.30 | signal in all pixels           |
| 617 | 5806814823792631168 | 361082409  | 15.03 | none                           |
| 618 | 5807013659294172416 | 1205987472 | 18.77 | TYC 9278-2110-1                |
| 619 | 5807178482962267392 | 1206039770 | 18.21 | no signal in individual pixels |
| 620 | 5808932375808220800 | 1206259410 | 17.44 | TIC 362325680                  |
| 621 | 5809843325487481472 | 294886960  | 15.95 | TIC 294886947                  |
| 622 | 5810928887062712960 | 293574993  | 14.42 | no signal in individual pixels |
| 623 | 5812395704296707200 | 1509663145 | 18.51 | no signal in individual pixels |
| 624 | 5812946937575469056 | 1509782361 | 18.60 | signal in all pixels           |
| 625 | 5813108393995312896 | 1509841385 | 17.16 | no signal in individual pixels |
| 626 | 5813717695228823936 | 1509980952 | 18.66 | no signal in individual pixels |
| 627 | 5814140487511460736 | 1510099842 | 17.71 | TIC 304663375                  |
| 628 | 5814742199551036544 | 1310978801 | 18.23 | no signal in individual pixels |
| 629 | 5815292638255116544 | 1311185220 | 18.23 | no signal in individual pixels |
| 630 | 5815333354547286784 | 1311202631 | 17.24 | signal in all pixels           |
| 631 | 5815934791716030976 | 1311362512 | 17.36 | signal in all pixels           |
| 632 | 5817044198944489984 | 304068663  | 14.49 | no signal in individual pixels |
| 633 | 5817506504915304576 | 290814091  | 12.19 | TIC 290814065                  |
| 634 | 5817603850371030528 | 447448883  | 15.68 | none                           |



|     |                     |            |       |                                |
|-----|---------------------|------------|-------|--------------------------------|
| 635 | 5818570527244772480 | 447471886  | 13.72 | TIC 447471894                  |
| 636 | 5818617840606728704 | 1312656204 | 17.84 | no signal in individual pixels |
| 637 | 5818655155273204608 | 1108123490 | 17.90 | TIC 426236341                  |
| 638 | 5820219863408835072 | 1108622035 | 18.86 | TIC 263303021                  |
| 639 | 5820270578372605440 | 1108654661 | 18.54 | TIC 447006364                  |
| 640 | 5821727083384403200 | 1207369013 | 18.73 | TIC 362475056                  |
| 641 | 5821884042982412160 | 1207467934 | 18.61 | ASTEP V-1104 (V)               |
| 642 | 5822038386923564032 | 1207570636 | 17.72 | signal in all pixels           |
| 643 | 5822373600540446208 | 1109255247 | 18.49 | no signal in individual pixels |
| 644 | 5822441598466662784 | 1109318520 | 17.62 | TYC 9035-1908-1                |
| 645 | 5822512104626666496 | 1109380147 | 18.89 | signal in all pixels           |
| 646 | 5822579965124305920 | 1109444403 | 18.78 | TIC 340169117                  |
| 647 | 5822634902031563008 | 1207701463 | 18.76 | no signal in individual pixels |
| 648 | 5822767363138063104 | 1207810577 | 17.57 | signal in all pixels           |
| 649 | 5823903296069305728 | 1110247140 | 18.99 | no signal in individual pixels |
| 650 | 5824214148655299712 | 461238865  | 15.26 | none                           |
| 651 | 5824276442854075648 | 1110663012 | 17.89 | TIC 271315403                  |
| 652 | 5824477000651703936 | 1110881415 | 18.03 | no signal in individual pixels |
| 653 | 5825168559114899712 | 1111810662 | 17.83 | TIC 455603263                  |
| 654 | 5825317989584775296 | 1112039648 | 18.66 | no signal in individual pixels |
| 655 | 5825436182777346944 | 1112218792 | 18.93 | signal in all pixels           |
| 656 | 5825514252433778048 | 1112301257 | 16.94 | no signal in individual pixels |
| 657 | 5825518852310368384 | 1112306141 | 18.73 | signal in all pixels           |
| 658 | 5825579188012454400 | 1112370447 | 18.62 | no signal in individual pixels |
| 659 | 5825671890580599168 | 1112472157 | 18.79 | no signal in individual pixels |
| 660 | 5825857781094805248 | 1112702157 | 18.73 | CD-63 1109                     |
| 661 | 5826010230932184320 | 1112895512 | 18.04 | signal in all pixels           |
| 662 | 5826637059946662016 | 1113735682 | 18.49 | no signal in individual pixels |
| 663 | 5826738661718005760 | 423016147  | 15.37 | TIC 423016159                  |
| 664 | 5826871732648937344 | 1114124355 | 18.90 | HP TrA (EB)                    |
| 665 | 5826872218025185280 | 456278935  | 14.99 | none                           |
| 666 | 5827770862587814912 | 1208111532 | 18.14 | signal in all pixels           |
| 667 | 5827890468846403968 | 1208191120 | 18.00 | TIC 350847864                  |
| 668 | 5828087380188820864 | 1208335965 | 17.91 | TIC 350181335                  |
| 669 | 5828530693828790016 | 1208671538 | 18.96 | signal in all pixels           |
| 670 | 5828750458746605440 | 350804607  | 15.53 | none                           |
| 671 | 5829423325484401024 | 1209571177 | 18.28 | no signal in individual pixels |
| 672 | 5829429853854340992 | 1209578048 | 17.81 | no signal in individual pixels |
| 673 | 5829521422529516416 | 1209679630 | 18.81 | TIC 300763561                  |
| 674 | 5829979918898739712 | 1210226154 | 16.52 | no signal in individual pixels |
| 675 | 5830401753419017856 | 1210569307 | 18.15 | TIC 402700560                  |
| 676 | 5830677932661741184 | 1312862967 | 18.18 | signal in all pixels           |
| 677 | 5830988235473614080 | 1210942057 | 18.80 | FX Nor (RR Lyr)                |
| 678 | 5831076853529185792 | 1211044038 | 18.52 | signal in all pixels           |
| 679 | 5831159557441951488 | 1211145726 | 18.84 | no signal in individual pixels |
| 680 | 5831359840371186688 | 1211417231 | 17.82 | signal in all pixels           |



|     |                     |            |       |                                        |
|-----|---------------------|------------|-------|----------------------------------------|
| 681 | 5831513909421222272 | 1211662258 | 18.95 | no signal in individual pixels         |
| 682 | 5831694469872124800 | 1211944398 | 18.98 | TIC 220771986                          |
| 683 | 5831747830535693184 | 1212028981 | 18.03 | Gaia EDR3 5831745833331476992 (RR Lyr) |
| 684 | 5831770164327935872 | 1212059075 | 17.30 | TIC 221301000                          |
| 685 | 5831867264991717504 | 1212202225 | 17.86 | TIC 221047381                          |
| 686 | 5832178839050684928 | 1115553747 | 18.72 | signal in all pixels                   |
| 687 | 5832506592315498880 | 1115821806 | 18.94 | no signal in individual pixels         |
| 688 | 5832798688751705472 | 1213078262 | 17.99 | signal in all pixels                   |
| 689 | 5833924382554707456 | 79909416   | 15.27 | none                                   |
| 690 | 5834191082863051008 | 73995531   | 11.67 | signal in all pixels                   |
| 691 | 5834436784992036736 | 1213775838 | 18.48 | no signal in individual pixels         |
| 692 | 5834500213072076800 | 1213897915 | 18.64 | no signal in individual pixels         |
| 693 | 5835101336698034304 | 1215387446 | 18.57 | no signal in individual pixels         |
| 694 | 5836303691397414400 | 429797824  | 16.45 | none                                   |
| 695 | 5837325927857851904 | 955130455  | 17.65 | signal in all pixels                   |
| 696 | 5839006011691771648 | 393976056  | 13.43 | TIC 393976075                          |
| 697 | 5839016422691618048 | 955641277  | 17.84 | signal in all pixels                   |
| 698 | 5839477672124221952 | 1005648015 | 16.73 | signal in all pixels                   |
| 699 | 5840274538868808576 | 955786147  | 17.86 | no signal in individual pixels         |
| 700 | 5840449533016550656 | 955853876  | 18.44 | no signal in individual pixels         |
| 701 | 5840464548227687936 | 955862575  | 18.21 | no signal in individual pixels         |
| 702 | 5840566841476999936 | 955902616  | 17.18 | signal in all pixels                   |
| 703 | 5841069421374403968 | 1006325087 | 16.15 | TIC 1006325065                         |
| 704 | 5841739676778285824 | 360412948  | 15.55 | no signal in individual pixels         |
| 705 | 5841978408247865984 | 956216302  | 17.22 | no signal in individual pixels         |
| 706 | 5841981053947246720 | 956217692  | 17.66 | signal in all pixels                   |
| 707 | 5842817473052628480 | 447994235  | 13.07 | none                                   |
| 708 | 5843275076052357888 | 956846129  | 16.51 | no signal in individual pixels         |
| 709 | 5843554111485447040 | 957045866  | 18.79 | EU Mus (RR Lyr)                        |
| 710 | 5843556684161637120 | 957047724  | 18.82 | no signal in individual pixels         |
| 711 | 5843566274839760000 | 957054229  | 17.28 | signal in all pixels                   |
| 712 | 5843659286654396416 | 957111944  | 18.02 | TIC 338140307                          |
| 713 | 5843985906014534912 | 1006435185 | 18.99 | signal in all pixels                   |
| 714 | 5844098193634825216 | 1006535733 | 17.96 | no signal in individual pixels         |
| 715 | 5844112148000611456 | 1006549634 | 18.68 | signal in all pixels                   |
| 716 | 5844864317021035392 | 957705955  | 18.58 | no signal in individual pixels         |
| 717 | 5844979628299579264 | 957834233  | 18.00 | TIC 957834257                          |
| 718 | 5846837077099568128 | 1008420332 | 18.17 | TIC 448256778                          |
| 719 | 5848489132008094080 | 258603810  | 16.10 | no signal in individual pixels         |
| 720 | 5848913680900988800 | 258611445  | 16.39 | HD 129795 (B2/3Vn)                     |
| 721 | 5849606716896266368 | 387425815  | 15.16 | no signal in individual pixels.        |
| 722 | 5850318199663644288 | 1012045630 | 18.95 | no signal in individual pixels         |
| 723 | 5850392279250691328 | 1012153152 | 18.51 | no signal in individual pixels         |
| 724 | 5850711622986006272 | 1012682181 | 16.29 | no signal in individual pixels         |
| 725 | 5852288734995259008 | 324848434  | 15.65 | TIC 324848407                          |
| 726 | 5852600377818703744 | 337900666  | 16.32 | no signal in individual pixels         |



|     |                     |            |       |                                       |
|-----|---------------------|------------|-------|---------------------------------------|
| 727 | 5852787840208469760 | 1017631564 | 16.34 | no signal in individual pixels        |
| 728 | 5852948437604395008 | 335085652  | 15.83 | no signal in individual pixels        |
| 729 | 5855027957693863552 | 958402522  | 18.54 | TIC 312804529                         |
| 730 | 5855332556771444096 | 958621883  | 18.28 | no signal in individual pixels        |
| 731 | 5856031472517744000 | 959314686  | 18.20 | no signal in individual pixels        |
| 732 | 5856141011354230400 | 959413900  | 18.95 | TIC 311842027                         |
| 733 | 5856176157068779136 | 959444093  | 17.80 | no signal in individual pixels        |
| 734 | 5856228624388963712 | 959492809  | 17.74 | signal in all pixels                  |
| 735 | 5856264775132757632 | 959527836  | 17.94 | no signal in individual pixels        |
| 736 | 5856324286212114048 | 959593444  | 18.89 | signal in all pixels                  |
| 737 | 5856428151396440064 | 959721186  | 18.48 | no signal in individual pixels        |
| 738 | 5856650978589405696 | 960039415  | 18.91 | signal in all pixels                  |
| 739 | 5856780755350239232 | 960245774  | 18.81 | signal in all pixels                  |
| 740 | 5856829821035392512 | 960340325  | 18.99 | signal in all pixels                  |
| 741 | 5857083529041956480 | 960777912  | 18.89 | signal in all pixels                  |
| 742 | 5857220349523071232 | 960986184  | 18.14 | signal in all pixels                  |
| 743 | 5858111679833161472 | 334339335  | 15.96 | Gaia DR2 5858111057014774400 (RR Lyr) |
| 744 | 5859738888326349312 | 965968658  | 16.79 | TIC 448017139                         |
| 745 | 5859931332899891200 | 966362012  | 17.60 | TIC 328842239                         |
| 746 | 5860659931128631552 | 967880862  | 17.44 | HD 311107 (B8)                        |
| 747 | 5861489684447376768 | 434801330  | 13.51 | no signal in individual pixels        |
| 748 | 5864039799897173504 | 449891534  | 15.36 | no signal in individual pixels        |
| 749 | 5864236165779760384 | 1023824714 | 16.17 | TIC 318720437                         |
| 750 | 5866716526516462592 | 335678265  | 15.31 | none                                  |
| 751 | 5869157987778544256 | 316893114  | 11.88 | no signal in individual pixels        |
| 752 | 5869375970282455808 | 449374594  | 16.46 | no signal in individual pixels        |
| 753 | 5869749254509572608 | 1030971374 | 16.33 | none                                  |
| 754 | 5870766543280392832 | 1032968755 | 14.63 | signal in all pixels                  |
| 755 | 5872222296667659904 | 208346128  | 14.43 | no signal in individual pixels        |
| 756 | 5872653992388283264 | 1036023325 | 18.63 | TIC 208837337                         |
| 757 | 5874138470576015104 | 293171001  | 15.58 | no signal in individual pixels        |
| 758 | 5875446992500886784 | 455460222  | 10.75 | none                                  |
| 759 | 5878436220983726336 | 392632624  | 16.12 | no signal in individual pixels        |
| 760 | 5886385827467871488 | 46197886   | 16.03 | no signal in individual pixels        |
| 761 | 5895627566324908032 | 210635816  | 16.68 | signal in all pixels                  |
| 762 | 5898485020906555904 | 1149937067 | 17.62 | signal in all pixels                  |
| 763 | 5898674652303523712 | 1042876519 | 18.59 | TYC 8289-810-1                        |
| 764 | 5899324536703881856 | 446364401  | 14.71 | no signal in individual pixels        |
| 765 | 5899732455544950528 | 313781919  | 14.56 | signal in all pixels                  |
| 766 | 5901546512278549504 | 370091691  | 15.14 | TIC 370091739                         |
| 767 | 5904341058511655168 | 250144006  | 16.32 | none                                  |
| 768 | 5905131431257671552 | 1154686323 | 17.63 | no signal in individual pixels        |
| 769 | 5905744168475316864 | 1043521606 | 17.79 | TYC 8283-3278-1                       |
| 770 | 5908697976404258816 | 1156213494 | 16.72 | no signal in individual pixels        |
| 771 | 5909243398587632256 | 1510223540 | 18.29 | signal in all pixels                  |
| 772 | 5909624795984270208 | 1510315966 | 17.51 | TIC 306882685                         |



|     |                     |            |       |                                                                                                        |
|-----|---------------------|------------|-------|--------------------------------------------------------------------------------------------------------|
| 773 | 5910260313710193152 | 1510514907 | 18.53 | no signal in individual pixels                                                                         |
| 774 | 5910274985315765120 | 305424845  | 15.01 | no signal in individual pixels                                                                         |
| 775 | 5910623152545379584 | 306010553  | 16.40 | TIC 305947198                                                                                          |
| 776 | 5911201117703147008 | 380460749  | 13.47 | VX Pav                                                                                                 |
| 777 | 5911947823541993216 | 1511076990 | 17.42 | TIC 306638921                                                                                          |
| 778 | 5912491841279017984 | 1511288572 | 16.93 | TIC 305186122                                                                                          |
| 779 | 5912875124161312128 | 1511464487 | 14.57 | TIC 74183935                                                                                           |
| 780 | 5912878457055996544 | 1511466048 | 16.53 | no signal in individual pixels                                                                         |
| 781 | 5912950612506611328 | 1511501931 | 18.17 | signal in all pixels                                                                                   |
| 782 | 5913074994762804608 | 1511568388 | 18.53 | no signal in individual pixels                                                                         |
| 783 | 5913583209648609536 | 290997905  | 13.50 | none                                                                                                   |
| 784 | 5913613235755146240 | 1313090772 | 17.97 | signal in all pixels                                                                                   |
| 785 | 5913634508739084288 | 1313102045 | 17.77 | TIC 290811927                                                                                          |
| 786 | 5913840422347943296 | 1511687960 | 18.36 | no signal in individual pixels                                                                         |
| 787 | 5913928555078888320 | 1313232954 | 17.48 | no signal in individual pixels                                                                         |
| 788 | 5913966458169513728 | 1511706171 | 17.50 | signal in all pixels                                                                                   |
| 789 | 5913966488226977536 | 304745339  | 15.56 | signal in all pixels                                                                                   |
| 790 | 5913980820540596480 | 1511713110 | 17.58 | V522 Ara (RR Lyr)                                                                                      |
| 791 | 5914336512556478464 | 173194752  | 16.91 | no signal in individual pixels                                                                         |
| 792 | 5914664575028652672 | 1313633708 | 17.86 | no signal in individual pixels                                                                         |
| 793 | 5914822698545656192 | 1313753636 | 18.34 | no signal in individual pixels                                                                         |
| 794 | 5914963058077697024 | 1313865854 | 16.77 | signal in all pixels                                                                                   |
| 795 | 5915059304013286016 | 1313937260 | 16.33 | no signal in individual pixels                                                                         |
| 796 | 5915195987049950336 | 1314041719 | 18.31 | no signal in individual pixels                                                                         |
| 797 | 5915374481581769856 | 1314203722 | 18.05 | TIC 171550067                                                                                          |
| 798 | 5915495603966207360 | 1511730545 | 18.10 | TIC 304833926                                                                                          |
| 799 | 5915601191440196352 | 1314334862 | 18.65 | no signal in individual pixels                                                                         |
| 800 | 5915615107133861248 | 1314343279 | 18.73 | ASTEP V-1638 (EB)                                                                                      |
| 801 | 5915874518865405568 | 1314448966 | 18.06 | no signal in individual pixels                                                                         |
| 802 | 5915888915589867008 | 380163678  | 15.02 | none                                                                                                   |
| 803 | 5916147129019888128 | 1511876241 | 18.93 | TIC 367746024                                                                                          |
| 804 | 5916496709313788032 | 1314715953 | 17.75 | signal in all pixels                                                                                   |
| 805 | 5916635793217885696 | 1314827632 | 18.54 | V467 Ara (RR Lyr)                                                                                      |
| 806 | 5916827662300514048 | 1314986049 | 17.30 | TIC 172636779                                                                                          |
| 807 | 5916870813829744384 | 1315027363 | 17.68 | TIC 172638589                                                                                          |
| 808 | 5916872501764463872 | 1315029046 | 18.85 | signal in all pixels                                                                                   |
| 809 | 5916958263667362816 | 171215892  | 14.25 | none                                                                                                   |
| 810 | 5917060342160958720 | 1315225168 | 17.92 | signal in all pixels                                                                                   |
| 811 | 5917095943138304640 | 1315264570 | 18.71 | TIC 171738431                                                                                          |
| 812 | 5917096561635149696 | 1315265389 | 18.68 | signal in all pixels                                                                                   |
| 813 | 5917446343776662912 | 1315622784 | 17.27 | TIC 172808758                                                                                          |
| 814 | 5917447958684459648 | 1315624695 | 18.00 | TIC 1315624260                                                                                         |
| 815 | 5917501486827858432 | 1315686590 | 18.05 | signal in all pixels                                                                                   |
| 816 | 5917560482495449728 | 1315761536 | 17.13 | V714 Ara (RR Lyr)                                                                                      |
| 817 | 5917678267689959808 | 1315911100 | 18.79 | 23.61 $\mu$ Hz: V429 Ara (RR Lyr);<br>15.05 $\mu$ Hz: Gaia EDR3 5917681536188862464 (RR Lyr candidate) |



|     |                     |            |       |                                                                                   |
|-----|---------------------|------------|-------|-----------------------------------------------------------------------------------|
| 818 | 5917795400028702720 | 1512001875 | 17.64 | signal in all pixels                                                              |
| 819 | 5917945826965005440 | 76063800   | 14.73 | no signal in individual pixels                                                    |
| 820 | 5918072137660735232 | 75222051   | 16.02 | DE Pav (RR Lyr)                                                                   |
| 821 | 5918674390857151616 | 1512301694 | 18.61 | no signal in individual pixels                                                    |
| 822 | 5918720712084075136 | 1512321018 | 18.63 | TIC 75668886                                                                      |
| 823 | 5918752941519223424 | 337190387  | 16.50 | 161.11 $\mu$ Hz, 167.59 $\mu$ Hz: none;<br>44.68 $\mu$ Hz+harmonic: TIC 337190401 |
| 824 | 5918985690088663296 | 360677156  | 16.00 | ASTEP V-1418 (EB)                                                                 |
| 825 | 5919111863348783232 | 1512495381 | 17.82 | no signal in individual pixels                                                    |
| 826 | 5919118804007300992 | 1512499020 | 18.15 | signal in all pixels                                                              |
| 827 | 5919475110196972416 | 1512700761 | 18.43 | no signal in individual pixels                                                    |
| 828 | 5919475385082440192 | 1512700908 | 18.17 | signal in all pixels                                                              |
| 829 | 5919831699872564480 | 360327923  | 13.61 | no signal in individual pixels                                                    |
| 830 | 5920026519573591680 | 1513024042 | 17.91 | signal in all pixels                                                              |
| 831 | 5920588503158763648 | 1513264598 | 17.14 | signal in all pixels                                                              |
| 832 | 5920658807487485824 | 1513295139 | 17.23 | signal in all pixels                                                              |
| 833 | 5920779135290822272 | 1513348322 | 18.34 | Gaia EDR3 5920779272729779840 (RR Lyr)                                            |
| 834 | 5920848468939288704 | 1513381609 | 18.29 | TIC 75528597                                                                      |
| 835 | 5920910350832882688 | 1513413154 | 18.92 | TIC 75305674                                                                      |
| 836 | 5921199767200727680 | 1513570515 | 18.88 | signal in all pixels                                                              |
| 837 | 5921888263345597696 | 1514060057 | 18.86 | no signal in individual pixels                                                    |
| 838 | 5922555533763349888 | 1316015281 | 18.63 | none                                                                              |
| 839 | 5922784678868831488 | 1316196509 | 18.03 | TIC 174123557                                                                     |
| 840 | 5923022345162266240 | 1514744393 | 17.62 | signal in all pixels                                                              |
| 841 | 5923154355285680128 | 1316238371 | 18.37 | signal in all pixels                                                              |
| 842 | 5923572994356468992 | 1316619520 | 17.20 | TIC 173502035                                                                     |
| 843 | 5923629653567353088 | 173054589  | 14.40 | no signal in individual pixels                                                    |
| 844 | 5923721114870906496 | 1316808618 | 18.10 | TIC 172147254                                                                     |
| 845 | 5923753623503344768 | 1316858764 | 18.94 | signal in all pixels                                                              |
| 846 | 5924062685029320576 | 1317285527 | 17.71 | -                                                                                 |
| 847 | 5924163569527084928 | 1317414272 | 17.59 | TIC 213474487                                                                     |
| 848 | 5924696626515555840 | 412539331  | 15.16 | no signal in individual pixels                                                    |
| 849 | 5924780429894823424 | 1515157838 | 18.66 | no signal in individual pixels                                                    |
| 850 | 5924816851223108864 | 1515195026 | 17.83 | -                                                                                 |
| 851 | 5924999572026806784 | 1317974388 | 18.92 | TIC 372665467                                                                     |
| 852 | 5925165774378938368 | 1515460601 | 17.81 | signal in all pixels                                                              |
| 853 | 5925170893978306560 | 1515466728 | 18.43 | no signal in individual pixels                                                    |
| 854 | 5925187317943921280 | 1515487054 | 17.39 | -                                                                                 |
| 855 | 5925267715411204864 | 412562559  | 15.56 | no signal in individual pixels                                                    |
| 856 | 5925476283316535424 | 1515819280 | 18.35 | TIC 214357475                                                                     |
| 857 | 5926790921271538304 | 1320023085 | 18.67 | signal in all pixels                                                              |
| 858 | 5926930215671513472 | 1320160048 | 18.53 | BZ Ara (RR Lyr candidate)                                                         |
| 859 | 5926998003119107712 | 1320231527 | 18.28 | signal in all pixels                                                              |
| 860 | 5927163758817055488 | 222239788  | 14.97 | no signal in individual pixels                                                    |
| 861 | 5927341707899291008 | 170049602  | 15.11 | none                                                                              |
| 862 | 5927503129953431424 | 1320614705 | 17.94 | V610 Ara (EB)                                                                     |



|     |                     |            |       |                                                  |
|-----|---------------------|------------|-------|--------------------------------------------------|
| 863 | 5927882628960248704 | 1218810004 | 18.89 | signal in all pixels                             |
| 864 | 5928433591680768256 | 1219783062 | 17.15 | signal in all pixels                             |
| 865 | 5929029660088311936 | 1321164747 | 17.49 | signal in all pixels                             |
| 866 | 5929244034811756800 | 1321468539 | 18.26 | no signal in individual pixels                   |
| 867 | 5929423250886362240 | 1321765583 | 16.72 | no signal in individual pixels.                  |
| 868 | 5929424316039231488 | 1321767384 | 18.20 | Gaia EDR3 5929421537240422272 (RR Lyr candidate) |
| 869 | 5929627730026309760 | 1322108447 | 16.63 | signal in all pixels                             |
| 870 | 5929734137799211648 | 1322280157 | 17.14 | signal in all pixels                             |
| 871 | 5929873058569911424 | 1322526846 | 18.20 | TIC 170151063                                    |
| 872 | 5930078495456807936 | 49117380   | 15.33 | no signal in individual pixels                   |
| 873 | 5930373679974910080 | 222186461  | 16.02 | TIC 222186458                                    |
| 874 | 5930853852961332608 | 1323805483 | 18.26 | signal in all pixels                             |
| 875 | 5945578035948729984 | 1516496324 | 18.91 | TYC 8356-449-1                                   |
| 876 | 5945662079857514752 | 1516554961 | 16.26 | TIC 396910578                                    |
| 877 | 5946436067338415872 | 1517239265 | 16.74 | TIC 388821174                                    |
| 878 | 5946979088657489920 | 1517867980 | 15.77 | signal in all pixels                             |
| 879 | 5947809387409633280 | 1518544829 | 19.00 | signal in all pixels                             |
| 880 | 5947838833700689792 | 1518570655 | 16.82 | no signal in individual pixels                   |
| 881 | 5947897490092362112 | 1518623844 | 16.83 | no signal in individual pixels                   |
| 882 | 5947996544906108672 | 1518726102 | 18.05 | no signal in individual pixels                   |
| 883 | 5948008678207992448 | 1518738535 | 17.80 | no signal in individual pixels                   |
| 884 | 5948043514666252672 | 1518774975 | 18.88 | no signal in individual pixels                   |
| 885 | 5948530259048620928 | 16796885   | 14.84 | no signal in individual pixels                   |
| 886 | 5950297655279565440 | 1522195966 | 18.25 | no signal in individual pixels                   |
| 887 | 5950530889137719168 | 1522394636 | 18.47 | TIC 214020620                                    |
| 888 | 5952080715231994496 | 1523900865 | 16.70 | TIC 16141385                                     |
| 889 | 5952149129760917760 | 1524069810 | 18.35 | signal in all pixels                             |
| 890 | 5953840659677202816 | 23318705   | 13.92 | none                                             |
| 891 | 5953846496519902336 | 1526612114 | 18.51 | TIC 22889795                                     |
| 892 | 5953985859618704768 | 23309679   | 16.36 | V586 Ara (RR Lyr)                                |
| 893 | 5953998267787073792 | 1526763125 | 17.54 | signal in all pixels                             |
| 894 | 5954096772853080448 | 1526877224 | 17.48 | V569 Ara (RR Lyr)                                |
| 895 | 5954340555193511168 | 1527179146 | 16.90 | none                                             |
| 896 | 5954409553857609216 | 1527253460 | 18.92 | signal in all pixels                             |
| 897 | 5954477203873970304 | 1527332906 | 18.12 | TYC 8344-261-1                                   |
| 898 | 5954623267122357376 | 1527511271 | 17.43 | TIC 21998764                                     |
| 899 | 5954673432342022144 | 21770030   | 15.89 | no signal in individual pixels                   |
| 900 | 5954720062822377216 | 1527638631 | 17.83 | no signal in individual pixels                   |
| 901 | 5955264454204347392 | 1528425275 | 18.25 | V968 Sco (RR Lyr)                                |
| 902 | 5956155784503677824 | 1529942174 | 17.97 | no signal in individual pixels                   |
| 903 | 5956246421166957824 | 1530071187 | 17.77 | HD 162747 (Irregular_V, B9III/IV)                |
| 904 | 5956347855414236288 | 1530232079 | 18.64 | no signal in individual pixels                   |
| 905 | 5956651561152105600 | 1530819494 | 18.76 | signal in all pixels                             |
| 906 | 5956733131200489856 | 23924768   | 15.77 | TIC 23931953                                     |
| 907 | 5956734673075307904 | 1530980617 | 18.66 | signal in all pixels                             |



|     |                     |            |       |                                |
|-----|---------------------|------------|-------|--------------------------------|
| 908 | 5956791886327668480 | 1531096951 | 18.66 | TIC 23490938                   |
| 909 | 5956805149187734272 | 1531126009 | 17.88 | signal in all pixels           |
| 910 | 5989131714442067712 | 1163012595 | 18.48 | TIC 254564998                  |
| 911 | 5989362994167861760 | 1163252638 | 18.38 | no signal in individual pixels |
| 912 | 5992245879309568896 | 224126354  | 16.70 | TIC 224121346                  |
| 913 | 6001062794303920000 | 1166550495 | 16.89 | no signal in individual pixels |
| 914 | 6001278436023666048 | 289769967  | 15.71 | no signal in individual pixels |
| 915 | 6004382146876150528 | 1168341733 | 18.06 | TYC 7826-2283-1                |
| 916 | 6009287789802192128 | 1170139593 | 18.31 | no signal in individual pixels |
| 917 | 6016275362286886144 | 1172010185 | 18.13 | no signal in individual pixels |
| 918 | 6029741802804505984 | 1393478067 | 18.52 | no signal in individual pixels |
| 919 | 6030044890000961664 | 1394813348 | 18.18 | no signal in individual pixels |
| 920 | 6030709957111851904 | 1254214539 | 18.44 | no signal in individual pixels |
| 921 | 6030836710199020416 | 466488694  | 15.41 | none                           |
| 922 | 6032738242517337088 | 1397936567 | 17.95 | no signal in individual pixels |
| 923 | 6040415204502288128 | 1256930522 | 18.11 | no signal in individual pixels |
| 924 | 6055329633055113600 | 435222860  | 16.12 | no signal in individual pixels |
| 925 | 6057427810480028416 | 379344824  | 15.05 | [CKS91] 12017-6220 (V)         |
| 926 | 6058884427202541696 | 67409472   | 12.00 | no signal in individual pixels |
| 927 | 6061705430420025856 | 406054890  | 15.83 | TIC 406054872                  |
| 928 | 6063408127268069248 | 420279755  | 14.89 | TIC 420279808                  |
| 929 | 6067605787774877568 | 987501762  | 17.84 | no signal in individual pixels |
| 930 | 6068966188577379584 | 1046930949 | 18.49 | no signal in individual pixels |
| 931 | 6069936099575837696 | 1047317325 | 17.96 | signal in all pixels           |
| 932 | 6069966198707004416 | 1047328157 | 17.95 | no signal in individual pixels |
| 933 | 6072291047318085248 | 989277782  | 18.91 | signal in all pixels           |
| 934 | 6072952163063423360 | 989787049  | 17.38 | TIC 288022372                  |
| 935 | 6075379949139944192 | 398767751  | 10.37 | none                           |
| 936 | 6075454681577448320 | 991180027  | 18.28 | no signal in individual pixels |
| 937 | 6075795049139380352 | 991432590  | 18.30 | -                              |
| 938 | 6076340033266006656 | 991772681  | 18.26 | no signal in individual pixels |
| 939 | 6077028155742966528 | 992162933  | 17.69 | TIC 334215363                  |
| 940 | 6077115910515076608 | 429199321  | 15.83 | no signal in individual pixels |
| 941 | 6077194147621393152 | 992245885  | 18.65 | signal in all pixels           |
| 942 | 6077730331356709248 | 992478825  | 16.52 | no signal in individual pixels |
| 943 | 6077744418849436800 | 992485167  | 17.47 | TIC 403957442                  |
| 944 | 6080641254022107008 | 993452137  | 18.46 | no signal in individual pixels |
| 945 | 6082286668870223232 | 438836467  | 16.18 | signal in all pixels           |
| 946 | 6083108661191997568 | 1047943103 | 16.98 | CRTS J133816.4-474540 (EB)     |
| 947 | 6083486824483106944 | 1048026748 | 17.00 | none                           |
| 948 | 6083505447446326400 | 1048040030 | 18.65 | signal in all pixels           |
| 949 | 6083507612124915072 | 438622872  | 14.98 | signal in all pixels           |
| 950 | 6083508333664344832 | 1048045403 | 18.28 | no signal in individual pixels |
| 951 | 6083512044518010368 | 1048057161 | 18.20 | Cl* NGC 5139 B V39 (RR Lyr)    |
| 952 | 6083513384548113920 | 1048059374 | 18.68 | Cl* NGC 5139 B V79 (RR Lyr)    |
| 953 | 6083514277899316480 | 1048061197 | 18.20 | no signal in individual pixels |



|     |                     |            |       |                                |
|-----|---------------------|------------|-------|--------------------------------|
| 954 | 6083514380992694656 | 1048061758 | 17.29 | no signal in individual pixels |
| 955 | 6083514685923924992 | 1048062979 | 17.11 | CI* NGC 5139 SAW V150 (RR Lyr) |
| 956 | 6083516060313791232 | 438625280  | 14.18 | signal in all pixels           |
| 957 | 6083516236407187328 | 1048069704 | 18.49 | signal in all pixels           |
| 958 | 6083518328056785024 | 1048076255 | 18.78 | CI* NGC 5139 WSB V26 (EB)      |
| 959 | 6083675425070169216 | 1048098822 | 18.35 | CI* NGC 5139 LEID 69005        |
| 960 | 6083675803027407872 | 1048099460 | 16.89 | no signal in individual pixels |
| 961 | 6083681781656374272 | 363877893  | 13.04 | none                           |
| 962 | 6083685423788857216 | 1048103525 | 17.47 | signal in all pixels           |
| 963 | 6083689650001261440 | 1048107752 | 18.83 | signal in all pixels           |
| 964 | 6083690131073461120 | 438597464  | 16.15 | CI* NGC 5139 B V95 (RR Lyr)    |
| 965 | 6083695525530821760 | 1048116318 | 17.28 | signal in all pixels           |
| 966 | 6083699339456205824 | 1048127523 | 18.54 | signal in all pixels           |
| 967 | 6083709613047607808 | 1048160619 | 18.45 | no signal in individual pixels |
| 968 | 6083712671051864832 | 1048167132 | 18.42 | CI* NGC 5139 B V33 (RR Lyr)    |
| 969 | 6083718271691367040 | 1048189244 | 18.21 | CI* NGC 5139 SAW V163 (RR Lyr) |
| 970 | 6083718890166800128 | 1048190978 | 17.98 | CI* NGC 5139 B V68 (RR Lyr)    |
| 971 | 6083721604591054464 | 1048198838 | 18.20 | CI* NGC 5139 B V74 (RR Lyr)    |
| 972 | 6083721634628791680 | 1048198949 | 18.72 | CI* NGC 5139 B V36 (RR Lyr)    |
| 973 | 6083722390543138816 | 1048200959 | 16.75 | no signal in individual pixels |
| 974 | 6083742048642853248 | 1048211869 | 16.66 | no signal in individual pixels |
| 975 | 6083769669543511936 | 1048223139 | 18.35 | CI* NGC 5139 SAW V134 (RR Lyr) |
| 976 | 6083933531129596288 | 243192184  | 14.91 | none                           |
| 977 | 6084986730131301248 | 245008002  | 16.20 | none                           |
| 978 | 6085530644789992320 | 169158381  | 16.46 | TYC 8254-1635-1                |
| 979 | 6086922725287875456 | 994405885  | 17.18 | TIC 453773405                  |
| 980 | 6086950831553282816 | 453838097  | 15.51 | none                           |
| 981 | 6089461982977420544 | 329693923  | 13.82 | none                           |
| 982 | 6090382819662877952 | 1049272547 | 18.32 | signal in all pixels           |
| 983 | 6090850150765589376 | 312718333  | 16.20 | none                           |
| 984 | 6090943364436650880 | 1049488793 | 17.75 | signal in all pixels           |
| 985 | 6091467556604347520 | 1049703870 | 18.31 | no signal in individual pixels |
| 986 | 6092523916695056128 | 1050109577 | 18.04 | TIC 242494645                  |
| 987 | 6093997395420556544 | 1050605008 | 17.32 | V673 Cen (EB)                  |
| 988 | 6094602955750495488 | 1050795505 | 17.42 | TIC 241571032                  |
| 989 | 6094786501173315200 | 1050849495 | 16.45 | no signal in individual pixels |
| 990 | 6095905322973891328 | 1051129623 | 18.39 | TIC 242255440                  |
| 991 | 6097877675030930048 | 457859082  | 15.95 | no signal in individual pixels |
| 992 | 6099238148875711616 | 1051842160 | 18.40 | no signal in individual pixels |
| 993 | 6101089799475171072 | 1173099740 | 18.97 | Gaia EDR3 6101090521023906304  |
| 994 | 6107829251696990208 | 1052865952 | 18.93 | signal in all pixels           |
| 995 | 6108516210245811712 | 1052986381 | 17.96 | no signal in individual pixels |
| 996 | 6109378193000785920 | 242186776  | 12.66 | none                           |
| 997 | 6113264588643011712 | 1053661547 | 18.89 | -                              |
| 998 | 6124920953791085440 | 994500979  | 18.39 | signal in all pixels           |
| 999 | 6126099698979026944 | 994932221  | 18.56 | TIC 332650183                  |



|      |                     |            |       |                                                  |
|------|---------------------|------------|-------|--------------------------------------------------|
| 1000 | 6127970414931370112 | 995416624  | 18.77 | Gaia EDR3 6127970178714136960 (RR Lyr candidate) |
| 1001 | 6128930739560386560 | 73086539   | 15.62 | no signal in individual pixels                   |
| 1002 | 6128957260979473152 | 995613567  | 18.53 | -                                                |
| 1003 | 6129139165732657280 | 73087120   | 15.09 | TIC 73087129                                     |
| 1004 | 6129485271386704640 | 995707478  | 18.06 | -                                                |
| 1005 | 6130406627760739456 | 22562147   | 15.59 | TIC 22562145                                     |
| 1006 | 6130872717612496768 | 333201290  | 15.97 | no signal in individual pixels                   |
| 1007 | 6131726350945883264 | 996145031  | 18.39 | -                                                |
| 1008 | 6132026341527645312 | 72177745   | 17.26 | none                                             |
| 1009 | 6133998972766965120 | 996458859  | 17.49 | signal in all pixels                             |
| 1010 | 6135072748952161536 | 248111983  | 15.78 | none                                             |
| 1011 | 6135377137573842560 | 996684230  | 18.40 | signal in all pixels                             |
| 1012 | 6135761416887274112 | 996737915  | 17.81 | TIC 258516818                                    |
| 1013 | 6142378896336639360 | 30073382   | 11.66 | no signal in individual pixels                   |
| 1014 | 6142640550041393024 | 102314646  | 12.65 | no signal in individual pixels                   |
| 1015 | 6143097637642898688 | 22034812   | 14.44 | none                                             |
| 1016 | 6143488028696637568 | 997443582  | 18.58 | TIC 22216722                                     |
| 1017 | 6144582974769700992 | 997589943  | 17.90 | none                                             |
| 1018 | 6148325471834589184 | 134871451  | 11.95 | none                                             |
| 1019 | 6148596943829355136 | 380135300  | 12.31 | none                                             |
| 1020 | 6149617943456408320 | 134652401  | 12.60 | CRTS J120901.6-392517 (EB)                       |
| 1021 | 6155660726218745216 | 131312677  | 14.46 | none                                             |
| 1022 | 6158218941883819648 | 130945039  | 12.29 | none                                             |
| 1023 | 6158701528704596096 | 131237300  | 17.01 | none                                             |
| 1024 | 6161776759649387904 | 461264720  | 15.08 | none                                             |
| 1025 | 6166128832829891456 | 124780676  | 14.15 | none                                             |
| 1026 | 6177529630243170432 | 1055802439 | 18.33 | none                                             |
| 1027 | 6184268987981207552 | 229254851  | 16.34 | none                                             |
| 1028 | 6353389608797074176 | 293508490  | 16.71 | none                                             |
| 1029 | 6358470726907119232 | 352567167  | 16.88 | none                                             |
| 1030 | 6359461872217496704 | 1688142108 | 16.75 | none                                             |
| 1031 | 6365804611201098368 | 1815611169 | 17.84 | TIC 387132119                                    |
| 1032 | 6394778460578198016 | 237313549  | 13.77 | none                                             |
| 1033 | 6396691709593682304 | 2026251825 | 18.56 | no signal in individual pixels                   |
| 1034 | 6396953943117793664 | 2026260666 | 18.12 | UCAC4 109-123687                                 |
| 1035 | 6414030050188708480 | 345202106  | 13.73 | none                                             |
| 1036 | 6417709050455854336 | 292700038  | 15.12 | none                                             |
| 1037 | 6417943757530532992 | 1688406084 | 18.54 | no signal in individual pixels                   |
| 1038 | 6418217845164002944 | 344047599  | 16.61 | CRTS J183429.3-732636 (RR Lyr)                   |
| 1039 | 6421452956269493504 | 1815920535 | 15.93 | CRTS J190338.0-690139 (EB)                       |
| 1040 | 6423584664497694720 | 1922404553 | 18.21 | TIC 396168734                                    |
| 1041 | 6431593889451314560 | 1688602703 | 16.89 | TIC 295647609                                    |
| 1042 | 6431828600823764864 | 292293387  | 15.04 | signal in all pixels                             |
| 1043 | 6432487723686022784 | 1688686294 | 16.45 | TIC 295600534                                    |
| 1044 | 6436684142952570368 | 1816207373 | 17.14 | TIC 464315597                                    |



|      |                     |            |       |                                |
|------|---------------------|------------|-------|--------------------------------|
| 1045 | 6437128487387858688 | 1688997197 | 18.65 | no signal in individual pixels |
| 1046 | 6437199642106880256 | 1689010785 | 18.52 | CPD-66 3273                    |
| 1047 | 6437222456973856896 | 365604859  | 11.79 | none                           |
| 1048 | 6446358917564362752 | 409800401  | 15.65 | none                           |
| 1049 | 6448177342293519488 | 320660280  | 14.94 | none                           |
| 1050 | 6473212668007045632 | 1989478615 | 18.68 | TYC 8776-1214-1 (RR Lyr)       |
| 1051 | 6477149714203716864 | 79052662   | 14.28 | none                           |
| 1052 | 6489277945932225152 | 316881546  | 15.22 | none                           |
| 1053 | 6491685395361112832 | 220490049  | 14.25 | none                           |
| 1054 | 6505017626683426816 | 403208724  | 15.32 | no signal in individual pixels |
| 1055 | 6538511637082089856 | 2055734684 | 16.76 | none                           |
| 1056 | 6554413598876731520 | 206688456  | 15.64 | none                           |
| 1057 | 6566932088515730432 | 92219756   | 12.79 | no signal in individual pixels |
| 1058 | 6585413706451189376 | 2027767905 | 18.20 | no signal in individual pixels |
| 1059 | 6597995353583873536 | 278770293  | 15.46 | none                           |
| 1060 | 6624328240456787840 | 89435287   | 11.73 | none                           |
| 1061 | 6629776531031124352 | 365606909  | 13.12 | none                           |
| 1062 | 6630894150242812800 | 365659999  | 15.11 | none                           |
| 1063 | 6631310109232589568 | 365954183  | 15.33 | none                           |
| 1064 | 6632939997781472512 | 1816699805 | 17.63 | no signal in individual pixels |
| 1065 | 6633454981538710784 | 201600733  | 16.21 | CRTS J190101.7-590832 (EB)     |
| 1066 | 6633753876903084928 | 379574382  | 13.14 | none                           |
| 1067 | 6634058579067913472 | 365599503  | 15.98 | signal in all pixels           |
| 1068 | 6635167535321691776 | 1689787422 | 18.40 | TIC 365361132                  |
| 1069 | 6635756976635061504 | 1689913863 | 18.44 | CRTS J183024.3-583432 (EB)     |
| 1070 | 6635876376726404480 | 1689938989 | 18.81 | signal in all pixels           |
| 1071 | 6635977845327577600 | 1689959978 | 17.40 | no signal in individual pixels |
| 1072 | 6636169465294119936 | 1816810915 | 16.58 | CRTS J184213.7-592125 (RR Lyr) |
| 1073 | 6637613433296678400 | 1816971181 | 18.04 | signal in all pixels           |
| 1074 | 6638185183642097280 | 1817056562 | 17.01 | TIC 379406265                  |
| 1075 | 6640663306754718592 | 1923195859 | 16.89 | CRTS J194017.5-563749 (RotV*)  |
| 1076 | 6642096623240124288 | 1923309581 | 18.48 | no signal in individual pixels |
| 1077 | 6643054886280759040 | 421943847  | 16.47 | none                           |
| 1078 | 6643922950710710400 | 424849040  | 15.98 | no signal in individual pixels |
| 1079 | 6644151816632543872 | 1817309085 | 18.33 | signal in all pixels           |
| 1080 | 6644600765269455360 | 158398021  | 13.91 | no signal in individual pixels |
| 1081 | 6646232367509032704 | 424911726  | 15.22 | -                              |
| 1082 | 6647886136076867840 | 1690199809 | 18.90 | signal in all pixels           |
| 1083 | 6648027251520800640 | 1690231362 | 17.53 | no signal in individual pixels |
| 1084 | 6648706852790218240 | 1690398649 | 18.16 | no signal in individual pixels |
| 1085 | 6648740216095672576 | 1690408334 | 18.96 | no signal in individual pixels |
| 1086 | 6648822645105429760 | 1690433433 | 18.29 | TIC 76764448                   |
| 1087 | 6649267264417888640 | 119498482  | 16.29 | none                           |
| 1088 | 6649687582799963776 | 1690650787 | 16.53 | no signal in individual pixels |
| 1089 | 6650818537885355136 | 1690712439 | 17.32 | none                           |
| 1090 | 6651630385485595904 | 304706131  | 14.61 | none                           |



|      |                     |            |       |                                |
|------|---------------------|------------|-------|--------------------------------|
| 1091 | 6652855550676088320 | 324205791  | 16.27 | CRTS J182617.8-533946 (EB)     |
| 1092 | 6655273724642756096 | 1691613456 | 18.34 | GSC 08371-01874                |
| 1093 | 6655586604421043584 | 1691691172 | 17.68 | no signal in individual pixels |
| 1094 | 6660045502026676992 | 1923789560 | 18.77 | TIC 424724379                  |
| 1095 | 6665927472620003456 | 101694231  | 16.48 | no signal in individual pixels |
| 1096 | 6671273985350039168 | 1924199152 | 18.13 | BPS CS 30302-0101 (RR Lyr)     |
| 1097 | 6689454826729586048 | 114726596  | 16.05 | CD-41 13594 (EB)               |
| 1098 | 6690141845400532864 | 1924745547 | 17.03 | TIC 300405889                  |
| 1099 | 6703965970739289728 | 1692784184 | 18.93 | signal in all pixels           |
| 1100 | 6705082254219260544 | 1692984056 | 17.62 | no signal in individual pixels |
| 1101 | 6705536352519862144 | 390722433  | 14.45 | none                           |
| 1102 | 6705696052284928000 | 1818993504 | 17.56 | TIC 340113714                  |
| 1103 | 6706041333293445376 | 1693193276 | 17.49 | no signal in individual pixels |
| 1104 | 6706319406655905920 | 1693345170 | 18.47 | no signal in individual pixels |
| 1105 | 6706423619742155904 | 1693402829 | 18.91 | signal in all pixels           |
| 1106 | 6706897234380484096 | 1693633684 | 18.45 | TIC 90166569                   |
| 1107 | 6707158093510797056 | 1693781729 | 18.07 | no signal in individual pixels |
| 1108 | 6707179018594464896 | 1693793979 | 17.44 | TIC 87547631                   |
| 1109 | 6707223548812728192 | 1693820572 | 17.86 | none                           |
| 1110 | 6707258703133111040 | 87261650   | 15.36 | TYC 8361-113-1                 |
| 1111 | 6707575220734781568 | 1694048003 | 17.42 | no signal in individual pixels |
| 1112 | 6707581787750693120 | 1694051670 | 17.01 | TIC 88147424                   |
| 1113 | 6707713694774167424 | 1694125610 | 16.64 | signal in all pixels           |
| 1114 | 6707846112910655616 | 88229657   | 16.46 | signal in all pixels           |
| 1115 | 6707932802543692928 | 1694248987 | 18.90 | no signal in individual pixels |
| 1116 | 6708002655878479360 | 1694290995 | 18.66 | signal in all pixels           |
| 1117 | 6708177585610356480 | 1694381423 | 18.51 | no signal in individual pixels |
| 1118 | 6708601997098513280 | 390558833  | 16.38 | TIC 390558851                  |
| 1119 | 6708976891901433472 | 1694629913 | 18.04 | signal in all pixels           |
| 1120 | 6709029084344623104 | 1694640903 | 16.63 | TIC 405926734                  |
| 1121 | 6709455694858627968 | 1694765629 | 17.49 | no signal in individual pixels |
| 1122 | 6709554449042864896 | 1694815278 | 18.77 | signal in all pixels           |
| 1123 | 6710114237895552256 | 1695009776 | 18.37 | TIC 405862714                  |
| 1124 | 6710237481986505600 | 340206880  | 16.54 | no signal in individual pixels |
| 1125 | 6711255732828439040 | 1819495294 | 18.62 | no signal in individual pixels |
| 1126 | 6715637698985225088 | 1820305571 | 18.11 | CRTS J190559.1-413536 (RR Lyr) |
| 1127 | 6715668657109025408 | 1820313183 | 17.98 | TIC 254081333                  |
| 1128 | 6715697450570540416 | 1820319769 | 18.98 | no signal in individual pixels |
| 1129 | 6716109256332401280 | 397320542  | 15.72 | signal in all pixels           |
| 1130 | 6716317059728391424 | 1820509562 | 17.01 | no signal in individual pixels |
| 1131 | 6716831115778811904 | 1820682528 | 18.28 | no signal in individual pixels |
| 1132 | 6718466123926428800 | 1821082819 | 18.31 | no signal in individual pixels |
| 1133 | 6719492762847939840 | 1695141135 | 18.55 | signal in all pixels           |
| 1134 | 6719767228453543040 | 85580401   | 14.64 | none                           |
| 1135 | 6719832060966158720 | 1695397141 | 17.93 | signal in all pixels           |
| 1136 | 6720012964988176000 | 1695528638 | 18.00 | no signal in individual pixels |



|      |                     |            |       |                                                  |
|------|---------------------|------------|-------|--------------------------------------------------|
| 1137 | 6720291897344431232 | 87616982   | 16.78 | TIC 87617001                                     |
| 1138 | 6720948378799468544 | 1696279617 | 18.00 | no signal in individual pixels                   |
| 1139 | 6721010810456502144 | 1696341282 | 18.40 | no signal in individual pixels                   |
| 1140 | 6721011463293001216 | 1696341981 | 18.56 | no signal in individual pixels                   |
| 1141 | 6721012146178998656 | 1696342755 | 17.36 | signal in all pixels                             |
| 1142 | 6721186590570973952 | 1696490624 | 18.05 | TIC 88357018                                     |
| 1143 | 6721297851716806144 | 1696574308 | 18.65 | TIC 89046387                                     |
| 1144 | 6721535964705982336 | 1696776702 | 16.51 | no signal in individual pixels                   |
| 1145 | 6721917804462049024 | 1697022408 | 18.16 | Gaia EDR3 6721914849533726592 (RR Lyr candidate) |
| 1146 | 6721972878824710528 | 1697056414 | 17.70 | no signal in individual pixels                   |
| 1147 | 6721972913184416512 | 1697056436 | 17.11 | no signal in individual pixels                   |
| 1148 | 6722163918967853824 | 1697175423 | 17.83 | TYC 7910-2632-1                                  |
| 1149 | 6722165362076920576 | 1697176194 | 17.82 | TYC 7910-2632-1                                  |
| 1150 | 6722568509193661824 | 314200124  | 13.29 | no signal in individual pixels                   |
| 1151 | 6722872794732952320 | 90322028   | 16.04 | signal in all pixels                             |
| 1152 | 6722877605099385216 | 1697477215 | 18.43 | no signal in individual pixels                   |
| 1153 | 6722915714351340928 | 91002569   | 15.92 | no signal in individual pixels                   |
| 1154 | 6723109224093457920 | 1697636174 | 17.55 | no signal in individual pixels                   |
| 1155 | 6723641422078567040 | 1698005658 | 18.50 | no signal in individual pixels                   |
| 1156 | 6723700623909615744 | 1698051047 | 17.68 | signal in all pixels                             |
| 1157 | 6723793463924346624 | 1698119003 | 18.63 | TIC 314323408                                    |
| 1158 | 6723877164246876672 | 1698184543 | 17.05 | TIC 62722069                                     |
| 1159 | 6723895100042162432 | 1698205845 | 17.90 | TIC 62882921                                     |
| 1160 | 6723910875468556672 | 1698225312 | 17.54 | no signal in individual pixels                   |
| 1161 | 6724029210381298816 | 1698368794 | 16.64 | TIC 86334926                                     |
| 1162 | 6724043126080066048 | 1698392979 | 16.85 | no signal in individual pixels                   |
| 1163 | 6724043327941534976 | 1698393543 | 17.36 | signal in all pixels                             |
| 1164 | 6724098651426879360 | 1698453868 | 18.44 | TIC 86414230                                     |
| 1165 | 6724163110285607680 | 1698530325 | 18.92 | TIC 62717688                                     |
| 1166 | 6724172387412131456 | 1698542618 | 18.43 | TIC 63085065                                     |
| 1167 | 6724253678275863168 | 1698655497 | 18.31 | no signal in individual pixels                   |
| 1168 | 6724305011706657536 | 1698726721 | 16.83 | no signal in individual pixels                   |
| 1169 | 6724349030832282240 | 1698781611 | 18.51 | TIC 87068904                                     |
| 1170 | 6724452552423350784 | 1698912110 | 18.66 | no signal in individual pixels                   |
| 1171 | 6724605521994057856 | 1699066765 | 18.99 | no signal in individual pixels                   |
| 1172 | 6724624424133155456 | 1699084392 | 18.17 | TIC 89572664                                     |
| 1173 | 6724659226259008384 | 1699118430 | 18.09 | no signal in individual pixels                   |
| 1174 | 6724668920014115456 | 57424692   | 16.46 | TIC 57424707                                     |
| 1175 | 6724781100242508416 | 1699249686 | 17.44 | signal in all pixels                             |
| 1176 | 6724789758906008320 | 1699259820 | 18.11 | TIC 87411648                                     |
| 1177 | 6724821369874307200 | 1699299390 | 18.46 | TIC 368646953                                    |
| 1178 | 6725085222601520640 | 1699649874 | 18.33 | V468 CrA (RR Lyr)                                |
| 1179 | 6725204897558032640 | 1699831657 | 18.24 | Gaia EDR3 6725205035020986112 (RR Lyr candidate) |
| 1180 | 6725286257113064192 | 1699959160 | 18.10 | none                                             |
| 1181 | 6725379268928381184 | 1700128422 | 17.95 | TIC 326129890                                    |



|      |                     |            |       |                                                  |
|------|---------------------|------------|-------|--------------------------------------------------|
| 1182 | 6725487403330496512 | 1700318597 | 18.66 | no signal in individual pixels                   |
| 1183 | 6725550625269597184 | 1700439042 | 18.23 | no signal in individual pixels                   |
| 1184 | 6725625941819460224 | 1700556684 | 18.87 | no signal in individual pixels                   |
| 1185 | 6725772932757664640 | 1700781813 | 18.37 | no signal in individual pixels                   |
| 1186 | 6725813129361447296 | 1700847280 | 18.40 | V675 CrA (RR Lyr)                                |
| 1187 | 6725863363303970816 | 1700932204 | 18.49 | no signal in individual pixels                   |
| 1188 | 6725900269949627776 | 1701001075 | 18.06 | no signal in individual pixels                   |
| 1189 | 6726004757944446848 | 331770091  | 14.91 | no signal in individual pixels                   |
| 1190 | 6726050726936450688 | 1701302063 | 18.27 | no signal in individual pixels                   |
| 1191 | 6726064990569369344 | 331768098  | 13.65 | none                                             |
| 1192 | 6726116491478181632 | 1701443892 | 17.99 | TIC 331426373                                    |
| 1193 | 6726123157285045504 | 1701458783 | 18.17 | no signal in individual pixels                   |
| 1194 | 6726547087729655680 | 1701901283 | 18.86 | signal in all pixels                             |
| 1195 | 6726719711040368512 | 1702092609 | 18.99 | -                                                |
| 1196 | 6726741426395303296 | 1702111750 | 18.73 | no signal in individual pixels                   |
| 1197 | 6726945420160781952 | 1702302060 | 18.82 | signal in all pixels                             |
| 1198 | 6727137834713073408 | 1702515637 | 18.89 | TIC 113150377                                    |
| 1199 | 6727173126446951424 | 1702553779 | 18.62 | no signal in individual pixels                   |
| 1200 | 6727177661933096320 | 1702558592 | 18.52 | no signal in individual pixels                   |
| 1201 | 6727226040464809856 | 1702614378 | 17.98 | no signal in individual pixels                   |
| 1202 | 6727298092818076160 | 1702711856 | 18.67 | -                                                |
| 1203 | 6727360279662489344 | 1702807558 | 18.61 | -                                                |
| 1204 | 6727394884195234816 | 1702862011 | 18.43 | V552 CrA (RR Lyr)                                |
| 1205 | 6727455146881494784 | 1702944293 | 17.12 | Gaia EDR3 6727455116847116544 (RR Lyr candidate) |
| 1206 | 6727481986146425728 | 1702983499 | 18.88 | signal in all pixels                             |
| 1207 | 6727683093676920576 | 1703357456 | 18.44 | signal in all pixels                             |
| 1208 | 6727683501706551808 | 1703358098 | 17.75 | signal in all pixels                             |
| 1209 | 6727697868407252224 | 1703384590 | 18.50 | no signal in individual pixels                   |
| 1210 | 6727707970132293120 | 1703404139 | 18.13 | no signal in individual pixels                   |
| 1211 | 6727758302872315520 | 1703497083 | 17.72 | TIC 1703497021                                   |
| 1212 | 6727773631611364224 | 1703528658 | 18.67 | no signal in individual pixels                   |
| 1213 | 6727808163159282432 | 1703600185 | 18.09 | no signal in individual pixels                   |
| 1214 | 6727998894039826304 | 1703871394 | 18.41 | Gaia EDR3 6727998894063546112 (RR Lyr candidate) |
| 1215 | 6728016761127835776 | 1703895899 | 18.80 | no signal in individual pixels                   |
| 1216 | 6728063696533517696 | 1703965520 | 18.97 | -                                                |
| 1217 | 6728221132867132160 | 1704248050 | 18.85 | signal in all pixels                             |
| 1218 | 6728306997848553856 | 59787418   | 15.24 | -                                                |
| 1219 | 6728799304141901696 | 1821570679 | 17.89 | TIC 316476530                                    |
| 1220 | 6729767046174280832 | 1821981722 | 18.68 | no signal in individual pixels                   |
| 1221 | 6729795148139731584 | 1704610980 | 16.52 | TIC 315091286                                    |
| 1222 | 6730412493868745472 | 1822220968 | 16.68 | signal in all pixels                             |
| 1223 | 6731115833412903424 | 1822569202 | 18.58 | no signal in individual pixels                   |
| 1224 | 6732702531774074368 | 1823353470 | 18.53 | -                                                |
| 1225 | 6732881103632134784 | 1823461657 | 17.37 | CD-32 14688                                      |
| 1226 | 6733050836430023552 | 315197972  | 14.99 | none                                             |



|      |                     |            |       |                                                 |
|------|---------------------|------------|-------|-------------------------------------------------|
| 1227 | 6733105713248415488 | 314936845  | 14.15 | none                                            |
| 1228 | 6733112825701400832 | 1704983834 | 18.33 | no signal in individual pixels                  |
| 1229 | 6733184461456593536 | 1705051107 | 18.18 | no signal in individual pixels                  |
| 1230 | 6733744495125532544 | 1705433855 | 18.89 | TIC 314816327                                   |
| 1231 | 6733747273970769920 | 1705436112 | 18.15 | no signal in individual pixels                  |
| 1232 | 6734104550838587776 | 1705798039 | 17.65 | signal in all pixels                            |
| 1233 | 6734135229798787328 | 1705847616 | 18.25 | TIC 60745776                                    |
| 1234 | 6734553387812132480 | 1706540932 | 17.73 | signal in all pixels                            |
| 1235 | 6734579024474758912 | 272768608  | 16.10 | signal in all pixels                            |
| 1236 | 6734773809812771328 | 1706829311 | 17.61 | TIC 338224118                                   |
| 1237 | 6734811360704758656 | 1706879440 | 18.02 | no signal in individual pixels                  |
| 1238 | 6735043808640836352 | 1707242716 | 18.92 | signal in all pixels                            |
| 1239 | 6735050268269491072 | 1707253717 | 18.41 | no signal in individual pixels                  |
| 1240 | 6735077648694196096 | 1707298185 | 18.84 | signal in all pixels                            |
| 1241 | 6736318314434186624 | 1707439295 | 17.42 | no signal in individual pixels                  |
| 1242 | 6736325903611726464 | 211034499  | 16.44 | signal in all pixels                            |
| 1243 | 6736530279650889088 | 1824825972 | 18.69 | no signal in individual pixels                  |
| 1244 | 6736598891768151424 | 1707624341 | 17.81 | V4150 Sgr (RR Lyr)                              |
| 1245 | 6736648305373453440 | 1707709176 | 17.79 | no signal in individual pixels                  |
| 1246 | 6736795021439662080 | 1707887439 | 18.79 | signal in all pixels                            |
| 1247 | 6736808348706428288 | 1707900671 | 18.15 | signal in all pixels                            |
| 1248 | 6737444725412355840 | 1925102663 | 18.57 | no signal in individual pixels                  |
| 1249 | 6747819785853653760 | 1926445618 | 18.76 | CRTS J194338.8-331113 (RR Lyr)                  |
| 1250 | 6756064989189602304 | 1826208435 | 18.54 | no signal in individual pixels                  |
| 1251 | 6757508789694160128 | 1826962366 | 18.88 | signal in all pixels                            |
| 1252 | 6757834279492026496 | 1927250484 | 18.82 | TIC 112245959                                   |
| 1253 | 6760252655324244224 | 1827858861 | 18.46 | Gaia EDR3 6760254128495971200 (Candidate RRLyr) |
| 1254 | 6760253239457454592 | 277479500  | 13.07 | none                                            |
| 1255 | 6760614596505860480 | 1828184615 | 18.93 | OGLE BLG-RRLYR-38224 (RR Lyr)                   |
| 1256 | 6760700912479537536 | 30339103   | 13.73 | TIC 108438382                                   |
| 1257 | 6761296916509146752 | 1828780950 | 18.66 | signal in all pixels                            |
| 1258 | 6761392745830038400 | 275201189  | 14.73 | signal in all pixels                            |
| 1259 | 6761395868240404864 | 1828903447 | 17.11 | HD 173502 (PulsV*bCep)                          |
| 1260 | 6761404767428025728 | 1828917119 | 18.91 | no signal in individual pixels                  |
| 1261 | 6804398115891931648 | 1992921035 | 14.51 | none                                            |
| 1262 | 6812649744499242368 | 53978379   | 15.47 | no signal in individual pixels                  |
