# Supplementary material for: A search for variable subdwarf B stars in TESS Full Frame Images III. An update on variable targets in both ecliptic hemispheres -- contamination analysis and new sdB pulsators
Source: arXiv:2301.01082 ancillary file (2023-01-03)
Supplement: Supplementary file 2 [file 12-north_no_spec_FTs.pdf]

| <b>Table 12. NEH - 228 spectroscopically unclassified variables with amplitude spectra</b> |                     |            |              |                                |
|--------------------------------------------------------------------------------------------|---------------------|------------|--------------|--------------------------------|
| <b>No.</b>                                                                                 | <b>Gaia DR2</b>     | <b>TIC</b> | <b>G</b>     | <b>Variable contaminator</b>   |
|                                                                                            |                     |            | <b>[mag]</b> |                                |
| 1                                                                                          | 1082306439760979840 | 743148169  | 18.81        | TIC 284473271                  |
| 2                                                                                          | 1107705772542003200 | 705157619  | 18.09        | no signal in individual pixels |
| 3                                                                                          | 1108642968765677696 | 743476657  | 18.74        | V486 Cam (RR Lyr)              |
| 4                                                                                          | 1112770367915047424 | 705166070  | 17.41        | none                           |
| 5                                                                                          | 1113516073020001152 | 705175423  | 18.32        | TIC 468921975                  |
| 6                                                                                          | 124179878329719936  | 137965683  | 14.38        | -                              |
| 7                                                                                          | 1299121920781686912 | 345646956  | 16.45        | 2MASS J16280505+2332141 (EB)   |
| 8                                                                                          | 1316367176548009088 | 1200490403 | 18.93        | signal in all pixels           |
| 9                                                                                          | 1328058588631578752 | 57188215   | 15.37        | NGC 6205 918 (RR Lyr)          |
| 10                                                                                         | 1360404507027046144 | 334900478  | 16.26        | CI* NGC 6341 SAW V5 (RR Lyr)   |
| 11                                                                                         | 1360404644463437184 | 1270830822 | 16.36        | CI* NGC 6341 HAC 12 (RR Lyr)   |
| 12                                                                                         | 1360404713182626176 | 1270831583 | 15.84        | CI* NGC 6341 SAW V5 (RR Lyr)   |
| 13                                                                                         | 1360405366019600128 | 1270835502 | 16.63        | CI* NGC 6341 BUON 252          |
| 14                                                                                         | 1360405572181496576 | 334899867  | 16.21        | CI* NGC 6341 HAC 2 (RR Lyr)    |
| 15                                                                                         | 1360405606536917888 | 1270837848 | 16.36        | CI* NGC 6341 HAC 2 (RR Lyr)    |
| 16                                                                                         | 1360405640896788608 | 334899799  | 16.43        | no signal in individual pixels |
| 17                                                                                         | 1360408252238042752 | 1270841916 | 16.48        | no signal in individual pixels |
| 18                                                                                         | 1360408561479212416 | 1270843280 | 16.53        | none                           |
| 19                                                                                         | 1360408694620012416 | 334899806  | 16.15        | signal in all pixels           |
| 20                                                                                         | 1360408698917922304 | 1270843742 | 15.99        | CI* NGC 6341 BUON 66           |
| 21                                                                                         | 1360408870716557568 | 334899706  | 16.16        | CI* NGC 6341 HAC 3 (RR Lyr)    |
| 22                                                                                         | 1360409386112764800 | 334855274  | 15.63        | no signal in individual pixels |
| 23                                                                                         | 1366750338385213184 | 188823525  | 15.41        | none                           |
| 24                                                                                         | 1408611838431462272 | 1270929100 | 18.81        | CI* NGC 6229 SAW V21 (RR Lyr)  |
| 25                                                                                         | 141362010961304960  | 433413657  | 11.98        | no signal in individual pixels |
| 26                                                                                         | 1454780812716838400 | 1000656229 | 18.02        | NGC 5272 378 (RR Lyr)          |
| 27                                                                                         | 1454781259395191168 | 1000658319 | 17.23        | NGC 5272 948 (RR Lyr)          |
| 28                                                                                         | 1454784557930979072 | 1000667332 | 17.79        | NGC 5272 361 (RR Lyr)          |
| 29                                                                                         | 1454785275190719616 | 416607024  | 16.72        | none                           |
| 30                                                                                         | 1454875301999567104 | 199498039  | 16.32        | NGC 5272 1357 (RR Lyr)         |
| 31                                                                                         | 1454875400782264192 | 1000678734 | 17.03        | NGC 5272 1353 (RR Lyr)         |
| 32                                                                                         | 1638908908259733888 | 1401027720 | 18.15        | TIC 233234760                  |
| 33                                                                                         | 1641988266667804416 | 199550188  | 15.54        | no signal in individual pixels |
| 34                                                                                         | 1651395688155045888 | 1401049068 | 16.19        | TIC 422828506                  |
| 35                                                                                         | 1661867677415309440 | 1001372446 | 18.99        | no signal in individual pixels |
| 36                                                                                         | 1674177667865952000 | 1001488696 | 18.55        | TIC 154181415                  |
| 37                                                                                         | 1792346408750425728 | 2001228745 | 18.47        | -                              |
| 38                                                                                         | 1800636593282297856 | 298659379  | 16.30        | ATO J324.3427+27.1433 (V)      |
| 39                                                                                         | 1810293977574625536 | 1941781336 | 17.45        | no signal in individual pixels |
| 40                                                                                         | 1815926298906033280 | 1942976796 | 16.52        | no signal in individual pixels |

|    |                     |            |       |                                         |
|----|---------------------|------------|-------|-----------------------------------------|
| 41 | 1816177434235193216 | 1943061704 | 18.15 | no signal in individual pixels          |
| 42 | 1816244500139424128 | 1943089437 | 18.11 | no signal in individual pixels          |
| 43 | 1816360464255460608 | 1943134495 | 17.40 | TIC 305026640                           |
| 44 | 1818494070870971904 | 1943792185 | 17.63 | [SHM2017] J308.59748+21.80372 (RR Lyr)  |
| 45 | 1818722769293285888 | 1943865981 | 16.85 | signal in all pixels                    |
| 46 | 1820808405423071616 | 1842059775 | 17.65 | UW Sge (V)                              |
| 47 | 1823649504799178624 | 1945335720 | 18.85 | ATO J301.6421+20.9989 (V)               |
| 48 | 1824783277431088512 | 392156280  | 15.96 | none                                    |
| 49 | 1838024657256337280 | 1950832039 | 17.22 | TIC 289365711                           |
| 50 | 1838679897466100352 | 1950905363 | 18.75 | ATO J313.3559+21.4050 (V)               |
| 51 | 1840251511899151360 | 1951113422 | 17.30 | TIC 298564459                           |
| 52 | 1840546765129724928 | 2001826392 | 16.82 | TIC 13487952                            |
| 53 | 1844179929505618560 | 1951817789 | 18.00 | signal in all pixels                    |
| 54 | 1846296802929256832 | 1952256069 | 17.66 | signal in all pixels                    |
| 55 | 1851085549721748608 | 298652703  | 13.28 | none                                    |
| 56 | 1855647423465451520 | 1953033063 | 18.42 | signal in all pixels                    |
| 57 | 1858179465616300672 | 1954064238 | 17.31 | TIC 282642055                           |
| 58 | 1866242253097646592 | 1957839690 | 17.49 | TIC 428637082                           |
| 59 | 1866281247095593600 | 1957854845 | 17.34 | no signal in individual pixels          |
| 60 | 1866461223403421952 | 1957921006 | 17.49 | no signal in individual pixels          |
| 61 | 1898657883100188544 | 162180176  | 13.29 | no signal in individual pixels          |
| 62 | 1901046606471675904 | 100594664  | 13.40 | none                                    |
| 63 | 1905951734001545856 | 2003638995 | 17.33 | signal in all pixels                    |
| 64 | 1906486401592241024 | 2003680569 | 17.84 | no signal in individual pixels          |
| 65 | 1917952899121466368 | 374138533  | 12.18 | none                                    |
| 66 | 193414231450777216  | 700897252  | 18.87 | ATO J087.9162+43.2076 (V)               |
| 67 | 1935580888012230784 | 2041819494 | 18.83 | HD 216766 (Double or multiple star, A2) |
| 68 | 1935962732084366592 | 154818961  | 14.25 | none                                    |
| 69 | 1939760166070592000 | 431631481  | 14.24 | signal in all pixels                    |
| 70 | 1943858286426802304 | 2042696692 | 16.47 | none                                    |
| 71 | 1945729968750061440 | 287598689  | 15.43 | none                                    |
| 72 | 1946614560216587008 | 287860863  | 14.63 | none                                    |
| 73 | 1947213759696113920 | 426980323  | 15.84 | TYC 2721-1981-1                         |
| 74 | 1948774379006908288 | 2004376628 | 18.05 | signal in all pixels                    |
| 75 | 1949931924236412032 | 256780950  | 13.06 | none                                    |
| 76 | 1953745271081325440 | 304964655  | 16.23 | TIC 304964668                           |
| 77 | 1956067989393212032 | 2005522236 | 17.65 | TIC 256787183                           |
| 78 | 1957707666169667456 | 2005732051 | 18.86 | TYC 3208-2231-1                         |
| 79 | 1964567764034901120 | 418537177  | 15.98 | no signal in individual pixels          |
| 80 | 196726961201325568  | 440388793  | 12.91 | none                                    |
| 81 | 1972683877836057600 | 419714501  | 15.64 | none                                    |
| 82 | 1979429038083843328 | 2011754031 | 15.25 | no signal in individual pixels          |
| 83 | 1983619032071794944 | 2012994650 | 18.43 | ATO J339.5969+46.7493 (EB candidate)    |
| 84 | 1985567439691237376 | 252527122  | 16.01 | TIC 252527111                           |

|     |                     |            |       |                                                                 |
|-----|---------------------|------------|-------|-----------------------------------------------------------------|
| 85  | 1985860695759886592 | 2043377471 | 17.56 | none                                                            |
| 86  | 1986759649594678528 | 2013148272 | 18.98 | ATO J338.8688+47.5751 (EB candidate)                            |
| 87  | 1987039337863810816 | 2013196679 | 18.94 | signal in all pixels                                            |
| 88  | 1987437812052513536 | 467529837  | 14.06 | none                                                            |
| 89  | 1992525217991908480 | 2044370599 | 14.41 | signal in all pixels                                            |
| 90  | 1995466995705902592 | 2045012618 | 18.54 | no signal in individual pixels                                  |
| 91  | 2001188476275895936 | 2014205738 | 18.91 | no signal in individual pixels                                  |
| 92  | 2001383841438971136 | 2014292802 | 16.96 | TIC 197498139                                                   |
| 93  | 2001659926247735040 | 431145331  | 15.27 | no signal in individual pixels                                  |
| 94  | 2032857194333300352 | 1867908327 | 17.08 | ATO J295.9120+30.6140 (V)                                       |
| 95  | 2034597824311822848 | 57507655   | 14.39 | signal in all pixels                                            |
| 96  | 2037262318906365312 | 1712166670 | 18.38 | no signal in individual pixels                                  |
| 97  | 2037415700780608128 | 1712233248 | 15.65 | none                                                            |
| 98  | 2037478025041657472 | 1712262553 | 17.18 | none                                                            |
| 99  | 2039324521683150080 | 403248740  | 13.90 | none                                                            |
| 100 | 2039459241912570880 | 1712945849 | 18.36 | TIC 29714517                                                    |
| 101 | 2040412174897885184 | 1713259626 | 18.18 | TIC 358598846                                                   |
| 102 | 2041930329878249984 | 20439718   | 15.33 | ATO J283.9630+30.8489 (EB candidate)                            |
| 103 | 2042199985105098496 | 28858086   | 14.71 | TYC 2638-2020-1                                                 |
| 104 | 2045244429726676608 | 1873354652 | 18.15 | TIC 1873354675                                                  |
| 105 | 2077210973653321600 | 1880746153 | 18.89 | 2MASS J19462002+4245541 (EB)                                    |
| 106 | 2079330419753334144 | 1881387607 | 17.81 | ATO J297.3604+44.6639 (EB candidate)                            |
| 107 | 2080459759936046464 | 271547244  | 14.77 | signal in all pixels                                            |
| 108 | 2080623857747831424 | 271659828  | 16.21 | no signal in individual pixels                                  |
| 109 | 2080657500231447808 | 1881707922 | 18.36 | 2MASS J19434470+4758368 (RotV*)                                 |
| 110 | 2083565811572191360 | 193863012  | 16.51 | TIC 193863015                                                   |
| 111 | 2086397839981036032 | 1881890367 | 18.10 | signal in all pixels                                            |
| 112 | 2087153483644941568 | 1882061796 | 16.87 | ATO J297.7812+49.3798 (EB)                                      |
| 113 | 2088226705776949888 | 1973057768 | 18.20 | TIC 295210915                                                   |
| 114 | 2088337756446382464 | 1973089618 | 17.82 | 15.63 $\mu$ Hz: TIC 405934050;<br>65.63 $\mu$ Hz: TIC 405934076 |
| 115 | 2090760637700298112 | 1714998110 | 17.83 | ATO J282.3403+33.8336 (EB candidate)                            |
| 116 | 2091025070244210944 | 68265412   | 13.36 | no signal in individual pixels                                  |
| 117 | 2092946501174006528 | 1715312730 | 16.91 | TYC 2652-1462-1                                                 |
| 118 | 2093324767535333888 | 237183273  | 14.58 | none                                                            |
| 119 | 2098226081131178880 | 336132473  | 13.12 | none                                                            |
| 120 | 2098353109083521664 | 336263242  | 16.26 | no signal in individual pixels                                  |
| 121 | 2099796218097223552 | 1715938427 | 17.52 | ATO J288.2562+39.9599 (V)                                       |
| 122 | 2100070954267036672 | 1715980555 | 17.77 | none                                                            |
| 123 | 2101160913887221888 | 1882248573 | 17.56 | signal in all pixels                                            |
| 124 | 2103059117632458368 | 1716331834 | 18.78 | no signal in individual pixels                                  |
| 125 | 2105585421693855744 | 158424730  | 17.28 | TIC 158424784                                                   |
| 126 | 2111853428244955264 | 1550574605 | 16.19 | none                                                            |
| 127 | 2113739326907805696 | 1550678705 | 18.65 | none                                                            |

|     |                     |            |       |                                      |
|-----|---------------------|------------|-------|--------------------------------------|
| 128 | 2115076131184395520 | 7804997    | 15.24 | none                                 |
| 129 | 2126207243307096192 | 1882483337 | 18.93 | TIC 159649131                        |
| 130 | 2127444125171341312 | 1882631458 | 16.73 | 2MASS J19232717+4546553 (RotV*)      |
| 131 | 2127850772675551232 | 1882665005 | 17.06 | V839 Cyg (RR Lyr)                    |
| 132 | 2128309711401769344 | 1882735968 | 18.90 | Gaia DR2 2128309715701366016         |
| 133 | 2128316411551020160 | 1882737149 | 18.89 | signal in all pixels                 |
| 134 | 2129409566628271232 | 290035516  | 16.02 | no signal in individual pixels       |
| 135 | 2129683074442759040 | 1882937348 | 16.78 | no signal in individual pixels       |
| 136 | 213308657404832768  | 664834496  | 16.72 | none                                 |
| 137 | 2137421299839603328 | 27998017   | 14.92 | signal in all pixels                 |
| 138 | 2137489984956949632 | 1883388858 | 17.77 | no signal in individual pixels       |
| 139 | 2138054511159522432 | 1883465325 | 18.48 | no signal in individual pixels       |
| 140 | 2138263800623825024 | 1883489297 | 17.55 | ATO J295.9989+54.1882 (V)            |
| 141 | 2141313261762604032 | 377197425  | 16.64 | none                                 |
| 142 | 2159159709869671168 | 233120549  | 15.64 | no signal in individual pixels       |
| 143 | 2161688071217417728 | 233064123  | 9.52  | no signal in individual pixels       |
| 144 | 2166781146535333888 | 366849840  | 15.89 | no signal in individual pixels       |
| 145 | 2171574772400722048 | 2016922661 | 16.34 | ATO J324.7678+51.8769 (EB)           |
| 146 | 2218305807587114624 | 411576480  | 16.00 | TIC 411577735                        |
| 147 | 2219210568217622912 | 412363512  | 16.86 | no signal in individual pixels       |
| 148 | 2231467614602883456 | 367090060  | 15.27 | none                                 |
| 149 | 2233797475444252288 | 1980585525 | 18.99 | signal in all pixels                 |
| 150 | 2233846442371207168 | 233266154  | 16.00 | ATO J299.8393+55.2170 (EB candidate) |
| 151 | 2234034351481581568 | 1980600166 | 18.75 | HD 190291 (solar like, F0)           |
| 152 | 2234114173452564096 | 1883770385 | 17.73 | no signal in individual pixels       |
| 153 | 2234624553006762624 | 1980637218 | 16.86 | no signal in individual pixels       |
| 154 | 2236210461089760000 | 1980673962 | 16.53 | GSC 03948-02316 (EB candidate)       |
| 155 | 2237409719037840384 | 256622207  | 17.00 | none                                 |
| 156 | 2237551517380084736 | 1883954695 | 16.22 | none                                 |
| 157 | 2238098803590426368 | 256384536  | 14.18 | signal in all pixels                 |
| 158 | 2239900383454607232 | 1884092103 | 17.38 | TIC 229974469                        |
| 159 | 2244819843293381376 | 236888904  | 15.68 | none                                 |
| 160 | 2254710740659370496 | 229962636  | 14.39 | no signal in individual pixels       |
| 161 | 2260984927665960704 | 1884416085 | 18.87 | TIC 259266402                        |
| 162 | 2261060214149311872 | 259170065  | 16.00 | TIC 259170046                        |
| 163 | 2271591989352943488 | 1981426661 | 18.62 | no signal in individual pixels       |
| 164 | 2287403962995179264 | 2051677111 | 16.91 | none                                 |
| 165 | 265031711598697728  | 321831910  | 14.97 | none                                 |
| 166 | 270172340774799488  | 306211983  | 15.75 | none                                 |
| 167 | 2863196315306344832 | 419547639  | 15.39 | no signal in individual pixels       |
| 168 | 316139833851242240  | 61337611   | 11.08 | none                                 |
| 169 | 318144999462982912  | 620805781  | 18.31 | CRTS J014521.8+345118 (EB)           |
| 170 | 336682765508713728  | 381730939  | 12.10 | none                                 |
| 171 | 341218594570556032  | 621422778  | 17.22 | signal in all pixels                 |

|     |                     |            |       |                                        |
|-----|---------------------|------------|-------|----------------------------------------|
| 172 | 343903292727125504  | 28690361   | 16.01 | ATO J026.6356+39.4140 (EB candidate)   |
| 173 | 3444031646422921344 | 309113421  | 16.26 | none                                   |
| 174 | 347293568112654720  | 189598026  | 16.57 | no signal in individual pixels         |
| 175 | 355680848969498368  | 301100606  | 15.35 | none                                   |
| 176 | 359675851453158656  | 622557069  | 18.39 | ATO J028.4788+52.0630 (EB candidate)   |
| 177 | 359799649588750464  | 250453464  | 15.11 | none                                   |
| 178 | 375930000563894784  | 191663789  | 11.52 | none                                   |
| 179 | 390486812962336256  | 601419369  | 18.71 | no signal in individual pixels         |
| 180 | 3938022150401267072 | 953956379  | 17.64 | CI* NGC 5024 SAW V33 (RR Lyr)          |
| 181 | 398116839542946944  | 196946103  | 14.43 | none                                   |
| 182 | 408964281963069696  | 403400154  | 16.13 | signal in all pixels                   |
| 183 | 412544287524575744  | 623638028  | 17.78 | TYC 3678-1252-1                        |
| 184 | 417769377238431744  | 240716329  | 16.22 | no signal in individual pixels         |
| 185 | 420571242106123776  | 603886634  | 15.35 | no signal in individual pixels         |
| 186 | 424739456329229824  | 604803910  | 18.58 | no signal in individual pixels         |
| 187 | 431525298501730816  | 359039906  | 16.72 | none                                   |
| 188 | 4497574170517871616 | 1681600851 | 17.43 | ATO J274.7168+14.2897 (EB candidate)   |
| 189 | 4498708419837302400 | 1681874891 | 18.41 | [SHM2017] J273.45866+15.64893 (RR Lyr) |
| 190 | 4500054462584536576 | 1505807101 | 16.95 | none                                   |
| 191 | 4502102302993010688 | 1682046125 | 17.29 | TIC 150398632                          |
| 192 | 4510156191310953984 | 462811965  | 16.03 | signal in all pixels                   |
| 193 | 4511999243375875584 | 1683377714 | 18.08 | signal in all pixels                   |
| 194 | 4519583124826317568 | 1811394469 | 17.03 | ATO J287.4350+20.6769 (EB)             |
| 195 | 4523127954613606912 | 1683842358 | 18.00 | no signal in individual pixels         |
| 196 | 4524788625192532864 | 1684271267 | 18.96 | signal in all pixels                   |
| 197 | 4527057879749609984 | 1684833800 | 18.83 | ATO J272.9633+19.5496 (EB candidate)   |
| 198 | 4528076581574683008 | 1685008842 | 17.68 | signal in all pixels                   |
| 199 | 4528846617674457472 | 342320091  | 14.53 | none                                   |
| 200 | 4530859303765646336 | 1813173164 | 18.96 | signal in all pixels                   |
| 201 | 4535895994733729024 | 1814885171 | 18.98 | ATO J280.7792+24.7897 (EB candidate)   |
| 202 | 4537278012127640576 | 1686111363 | 17.92 | no signal in individual pixels         |
| 203 | 453810165809216512  | 249953635  | 15.10 | none                                   |
| 204 | 4545156047299735936 | 1308564438 | 18.39 | TIC 400110989                          |
| 205 | 4548857999871987712 | 1506415981 | 18.16 | signal in all pixels                   |
| 206 | 4553345622222014720 | 1506923479 | 17.09 | CRTS J173053.2+182335 (EB)             |
| 207 | 4577858379269509248 | 1507563495 | 17.53 | TIC 275486706                          |
| 208 | 4587673444692894848 | 1815401960 | 17.22 | ATO J280.7781+29.9169 (V)              |
| 209 | 4589093944995879936 | 377682650  | 16.35 | TIC 377682645                          |
| 210 | 4589221793281682048 | 313898581  | 15.78 | ATO J273.0371+27.8948 (EB candidate)   |
| 211 | 4607166377101142272 | 76039505   | 15.79 | none                                   |
| 212 | 479934630799062656  | 82969837   | 16.99 | none                                   |
| 213 | 533041484802576512  | 379086469  | 16.22 | signal in all pixels                   |
| 214 | 550070931346054784  | 103511037  | 15.19 | none                                   |
| 215 | 559799478948924800  | 289267299  | 15.66 | TIC 289267282                          |

|     |                    |           |       |                                |
|-----|--------------------|-----------|-------|--------------------------------|
| 216 | 562049900075843072 | 629777697 | 17.29 | TIC 399797801                  |
| 217 | 573943493448464384 | 461601415 | 16.27 | no signal in individual pixels |
| 218 | 796315837515758720 | 4839754   | 13.62 | none                           |
| 219 | 897707263615279872 | 741428427 | 17.96 | signal in all pixels           |
| 220 | 898706032489528064 | 423081986 | 15.38 | -                              |
| 221 | 940404431153925632 | 741916679 | 17.49 | no signal in individual pixels |
| 222 | 945273721477246208 | 15924748  | 15.48 | TYC 2941-27-1                  |
| 223 | 951138134245928704 | 197181683 | 16.52 | no signal in individual pixels |
| 224 | 951495028848519424 | 742278003 | 18.20 | ATO J102.7425+41.2720 (V)      |
| 225 | 994967386444824064 | 11595640  | 13.07 | none                           |
| 226 | 995053663747140352 | 444902249 | 10.84 | none                           |
| 227 | 995329916043197952 | 258620986 | 15.84 | none                           |
| 228 | 999919342001035648 | 743017950 | 16.96 | none                           |
