# Supplementary material for: A search for variable subdwarf B stars in TESS Full Frame Images III. An update on variable targets in both ecliptic hemispheres -- contamination analysis and new sdB pulsators
Source: arXiv:2301.01082 ancillary file (2023-01-03)
Supplement: Supplementary file 3 [file 13-south_known_spec.pdf]

**Table 13. SEH - 76 non-sdB classified variables**

| No.                | Gaia DR2            | TIC        | G     | spT        | Period  | Variable contaminator          |
|--------------------|---------------------|------------|-------|------------|---------|--------------------------------|
|                    |                     |            | [mag] |            | [d]     |                                |
| Pulsators          |                     |            |       |            |         |                                |
| 1                  | 2969201399574096128 | 708596809  | 11.30 | A0IV/V     | -       | no signal in individual pixels |
| 2                  | 3109409266919646976 | 168595004  | 10.70 | A5         | -       | none                           |
| 3                  | 3115125211261708032 | 293137161  | 11.01 | A0         | -       | none                           |
| 4                  | 3344114626761364224 | 437889214  | 10.02 | B5         | -       | none                           |
| 5                  | 3396397877830881792 | 247513086  | 8.17  | A0         | -       | none                           |
| 6                  | 4817132519153233792 | 77436693   | 13.70 | BHe        | -       | none                           |
| 7                  | 5090382015016433920 | 686449995  | 6.63  | A5mA5-F2   | -       | none                           |
| 8                  | 5326745919424790656 | 126486580  | 9.16  | A0V        | -       | none                           |
| 9                  | 5429254969036524416 | 4595563    | 10.08 | A2/3(IV)   | -       | none                           |
| 10                 | 5524551806479093376 | 29796977   | 9.98  | A0         | -       | none                           |
| 11                 | 5796399012705196800 | 401975322  | 10.21 | B1III      | -       | none                           |
| 12                 | 6534581776366266752 | 224284872  | 13.55 | A0         | -       | none                           |
| 13                 | 65422239006166656   | 740003685  | 15.93 | DAO/sdOB   | -       | TIC 18997902                   |
| 14                 | 6702965728696663424 | 349351160  | 10.61 | A7         | -       | none                           |
| Phased lightcurves |                     |            |       |            |         |                                |
| 1                  | 2382531303846872448 | 12970429   | 13.85 | A0         | 0.059   | none                           |
| 2                  | 3484255561335762560 | 270373840  | 10.40 | B2V        | 0.6759  | none                           |
| 3                  | 4038633133701623168 | 1559025737 | 8.74  | B8V        | 2.026   | none                           |
| 4                  | 4686168482281917824 | 184134822  | 15.93 | B0-5(III)e | 0.8253  | none                           |
| 5                  | 4822681238943011840 | 78015136   | 13.16 | B          | 2.0625  | none                           |
| 6                  | 5362804330246457344 | 120596335  | 12.18 | sdO        | 0.3574  | none                           |
| 7                  | 5641012078094779904 | 829062665  | 8.10  | A0IV       | 1.6344  | none                           |
| 8                  | 5810017903018854784 | 293896689  | 10.60 | OB-        | 3.873   | none                           |
| 9                  | 6066705249078471296 | 253275342  | 8.10  | B8V        | 0.4812  | none                           |
| 10                 | 6204768798167836032 | 75647221   | 11.58 | OB-        | 0.5561  | -                              |
| 11                 | 6369440112037710592 | 327727051  | 11.36 | B4e        | 0.9279  | none                           |
| 12                 | 6375470177401596416 | 419571251  | 11.86 | B3         | 2.463   | none                           |
| 13                 | 6720095737595795200 | 88985610   | 8.85  | A1V        | 2.6584  | none                           |
| 14                 | 6799118570294811264 | 212299724  | 10.44 | B5III      | 1.8268  | none                           |
| 15                 | 6818355106040261376 | 25202305   | 12.09 | B6         | 2.7991  | none                           |
| Eclipsing binaries |                     |            |       |            |         |                                |
| 1                  | 2975118421398967424 | 146472758  | 13.27 | A          | 3.8133  | none                           |
| 2                  | 3834352875505630080 | 842028390  | 18.78 | DA         | 14.7223 | no signal in individual pixels |
| 3                  | 4040428807982926336 | 257415989  | 8.17  | B9II/III   | 2.1238  | none                           |
| 4                  | 4054618662690377856 | 1422846269 | 10.09 | B9V        | 1.7862  | signal in all pixels           |
| 5                  | 5351887970784238592 | 457418232  | 9.46  | B8III      | 2.1626  | none                           |
| 6                  | 5544723515521376000 | 145338612  | 8.95  | B9IV       | 4.8953  | none                           |
| 7                  | 5590218008142683520 | 22641187   | 15.75 | B0V        | 0.1018  | none                           |
| 8                  | 5759325125577015424 | 919588     | 9.32  | B9V        | 4.7913  | none                           |
| 9                  | 584063737770574976  | 800147867  | 18.93 | DA         | 3.1586  | TIC 323568463                  |
| 10                 | 5864602303103277568 | 320863824  | 9.94  | B1/2(III)  | 0.4452  | none                           |
| 11                 | 5902486663443800448 | 125080859  | 9.50  | A0III      | 5.5032  | none                           |

| Amplitude spectra |                     |            |       |         |   |                                                                 |
|-------------------|---------------------|------------|-------|---------|---|-----------------------------------------------------------------|
| 1                 | 2912264869258467200 | 37770142   | 9.03  | A0V     | - | no signal in individual pixels                                  |
| 2                 | 2948419495935518848 | 148295706  | 11.29 | OB      | - | none                                                            |
| 3                 | 3052873581621063936 | 125200530  | 8.25  | A0V     | - | none                                                            |
| 4                 | 3305764520174154752 | 284729168  | 16.40 | B       | - | none                                                            |
| 5                 | 3344334627867111168 | 151473446  | 12.19 | B:      | - | none                                                            |
| 6                 | 3469365322037142016 | 170494530  | 13.01 | B2      | - | none                                                            |
| 7                 | 3477724290468772736 | 57793227   | 15.89 | B       | - | CRTS J113909.0-323319 (EB)                                      |
| 8                 | 3480524609146540672 | 322809249  | 12.51 | B       | - | none                                                            |
| 9                 | 3490536212271814400 | 397419834  | 10.48 | B5      | - | none                                                            |
| 10                | 3491614283423744512 | 901474003  | 13.33 | B6      | - | none                                                            |
| 11                | 3555477217298285312 | 391824371  | 13.34 | B7      | - | none                                                            |
| 12                | 3753639444897348096 | 307936918  | 13.63 | A1      | - | none                                                            |
| 13                | 4786097841386890496 | 161635091  | 14.37 | B       | - | no signal in individual pixels                                  |
| 14                | 4870606614334908928 | 686060362  | 16.78 | sdO     | - | none                                                            |
| 15                | 4882954645311111424 | 686241564  | 16.63 | sdOHe   | - | TYC 7037-89-1 (EB)                                              |
| 16                | 4895712416167202176 | 44895938   | 14.55 | B3      | - | no signal in individual pixels                                  |
| 17                | 5329579463984075520 | 815576241  | 10.19 | A0      | - | 74.07 $\mu$ Hz: TIC 28796337;<br>193.75 $\mu$ Hz: TYC 8155-83-1 |
| 18                | 5453052901782552704 | 49044042   | 11.12 | B6      | - | none                                                            |
| 19                | 5700782320455378176 | 176304380  | 9.63  | B9IV/V  | - | none                                                            |
| 20                | 578539413395848704  | 800042858  | 18.30 | DA+M    | - | none                                                            |
| 21                | 5820064282494545280 | 1108525154 | 13.75 | B9III   | - | none                                                            |
| 22                | 5825954366325225728 | 423426730  | 8.12  | B9V     | - | none                                                            |
| 23                | 5864647692301841792 | 380846698  | 9.88  | A5/8    | - | none                                                            |
| 24                | 5877234901498723840 | 404098422  | 6.37  | B3IV    | - | none                                                            |
| 25                | 5884832114451618688 | 75708367   | 8.19  | B3/5V   | - | HD 140926 (Be star, B2/3Vnne)                                   |
| 26                | 5926114786038289280 | 213207249  | 8.81  | B9/9.5V | - | none                                                            |
| 27                | 6106849625493901824 | 159197255  | 12.53 | OB+     | - | none                                                            |
| 28                | 6137173602134028416 | 30989907   | 11.88 | OB+     | - | -                                                               |
| 29                | 6155114264643246336 | 103778583  | 11.64 | B       | - | none                                                            |
| 30                | 6409230097816994432 | 403284330  | 13.19 | B       | - | none                                                            |
| 31                | 6434081912466526080 | 382366857  | 11.43 | OB      | - | none                                                            |
| 32                | 6442023272633436672 | 1922709746 | 16.25 | B       | - | TIC 339659122                                                   |
| 33                | 6485148764374844800 | 126658450  | 11.52 | B2He?   | - | none                                                            |
| 34                | 6590537602435136768 | 89433335   | 13.40 | B3      | - | none                                                            |
| 35                | 6630629472878877056 | 365660822  | 12.30 | OB+     | - | none                                                            |
| 36                | 6706089368210943104 | 364952416  | 7.95  | A1/2V   | - | none                                                            |
