# Supplementary material for: A search for variable subdwarf B stars in TESS Full Frame Images III. An update on variable targets in both ecliptic hemispheres -- contamination analysis and new sdB pulsators
Source: arXiv:2301.01082 ancillary file (2023-01-03)
Supplement: Supplementary file 4 [file 14-north_known_spec.pdf]

**Table 14. NEH - 46 non-sdB classified variables**

| No.                | Gaia DR2            | TIC        | G     | spT   | Period | Variable contaminator                                           |
|--------------------|---------------------|------------|-------|-------|--------|-----------------------------------------------------------------|
|                    |                     |            | [mag] |       | [d]    |                                                                 |
| Pulsators          |                     |            |       |       |        |                                                                 |
| 1                  | 1625627602365544832 | 198209459  | 13.53 | B2    | -      | none                                                            |
| 2                  | 1713032695100155904 | 298091568  | 15.00 | B4.1  | -      | none                                                            |
| 3                  | 1861191062326013696 | 1955410399 | 10.31 | A0    | -      | none                                                            |
| 4                  | 2077737678383889408 | 270610177  | 11.77 | Be    | -      | 11 μHz+harmonics: none;<br>46 - 70 μHz: UCAC4 663-077912 (PulV) |
| 5                  | 2132171608553758336 | 279919275  | 13.46 | B3V   | -      | none                                                            |
| 6                  | 2276592430799302912 | 315774160  | 14.57 | B     | -      | TYC 4468-121-1                                                  |
| 7                  | 565004017238715264  | 609754520  | 6.64  | A7IV  | -      | none                                                            |
| Eclipsing binaries |                     |            |       |       |        |                                                                 |
| 1                  | 1821225425253990400 | 209942349  | 10.47 | A3    | 1.1762 | none                                                            |
| 2                  | 431584053656962816  | 283020391  | 16.27 | DAB   | 6.3199 | TIC 283020417                                                   |
| 3                  | 4322472232203849856 | 68975924   | 9.01  | A2    | 3.4703 | none                                                            |
| Phased lightcurves |                     |            |       |       |        |                                                                 |
| 1                  | 1075871822836912128 | 371767486  | 15.78 | DA:   | 0.8906 | none                                                            |
| 2                  | 1152688378078955264 | 459905076  | 15.29 | DA:   | 0.4294 | none                                                            |
| 3                  | 1459266575345109248 | 950014908  | 18.92 | DA    | 0.2015 | ATO J196.5813+25.4410 (V)                                       |
| 4                  | 1533367920984344320 | 18084735   | 11.57 | B4V   | 0.5465 | none                                                            |
| 5                  | 1542252151028439808 | 233640529  | 12.45 | A5    | 0.4131 | none                                                            |
| 6                  | 1605967612907047808 | 161002462  | 13.43 | B5.7  | 3.2063 | none                                                            |
| 7                  | 1659906934649659136 | 441686959  | 13.22 | B7.4  | 1.4122 | none                                                            |
| 8                  | 1828813777784480128 | 395530534  | 7.43  | B8V   | 1.3056 | none                                                            |
| 9                  | 2100882501225439488 | 120819719  | 13.44 | B     | 1.9043 | none                                                            |
| 10                 | 733024134288133120  | 82263882   | 13.54 | B6    | 1.0151 | none                                                            |
| 11                 | 747335579498454144  | 173005060  | 14.21 | B     | 2.3108 | none                                                            |
| 12                 | 767386312198060160  | 10113134   | 12.96 | B     | 0.9451 | none                                                            |
| 13                 | 936051906999100800  | 334276196  | 15.79 | B7    | 2.8301 | none                                                            |
| Amplitude spectra  |                     |            |       |       |        |                                                                 |
| 1                  | 1000850426487401728 | 14196017   | 14.16 | B1    | -      | none                                                            |
| 2                  | 1006212675978250240 | 339539154  | 14.50 | B1    | -      | none                                                            |
| 3                  | 1328057763997734144 | 57158280   | 13.13 | B2p   | -      | NGC 6205 344 (RR Lyr)                                           |
| 4                  | 1357436478465245184 | 115351563  | 16.03 | B     | -      | none                                                            |
| 5                  | 1511544337452190592 | 332350597  | 11.56 | B9kp  | -      | none                                                            |
| 6                  | 1662011812222609280 | 1001373800 | 16.84 | B     | -      | none                                                            |
| 7                  | 1683580626882189312 | 142961094  | 14.98 | B9.6  | -      | none                                                            |
| 8                  | 1706963459634476928 | 160409651  | 14.77 | B8.7  | -      | none                                                            |
| 9                  | 1862531534485984256 | 427303386  | 9.77  | A0    | -      | none                                                            |
| 10                 | 1865673736869022848 | 236211659  | 12.20 | B     | -      | none                                                            |
| 11                 | 1909071392087590656 | 120598109  | 15.01 | DBA   | -      | no signal in individual pixels                                  |
| 12                 | 1988623257385378304 | 65989760   | 12.90 | B     | -      | none                                                            |
| 13                 | 2099876757323090304 | 399792855  | 11.21 | B3V:p | -      | none                                                            |
| 14                 | 2106552442170221312 | 279911599  | 16.59 | B     | -      | signal in all pixels                                            |
| 15                 | 2130935452546450944 | 299032735  | 13.04 | B     | -      | none                                                            |

|    |                     |           |       |        |   |                                |
|----|---------------------|-----------|-------|--------|---|--------------------------------|
| 16 | 2131117284281652992 | 399912033 | 14.79 | B      | - | none                           |
| 17 | 300118776907986560  | 5645757   | 11.67 | B      | - | none                           |
| 18 | 426510559099112832  | 605260809 | 10.17 | A2III: | - | none                           |
| 19 | 474298671637654400  | 392371303 | 10.44 | A0     | - | none                           |
| 20 | 693490266000488704  | 126318109 | 12.25 | B      | - | no signal in individual pixels |
| 21 | 709613951186153472  | 172933463 | 10.34 | B8     | - | none                           |
| 22 | 791009766199488128  | 11894192  | 14.68 | DA:    | - | none                           |
| 23 | 908509660415660416  | 99010997  | 10.14 | B8     | - | none                           |
