# Supplementary material for: A search for variable subdwarf B stars in TESS Full Frame Images III. An update on variable targets in both ecliptic hemispheres -- contamination analysis and new sdB pulsators
Source: arXiv:2301.01082 ancillary file (2023-01-03)
Supplement: Supplementary file 5 [file 16-new_variables.pdf]

**Table 16. New variable stars found during the contamination analysis**

| No. | Gaia DR2            | TIC        | Name                  | G     |
|-----|---------------------|------------|-----------------------|-------|
|     |                     |            |                       | [mag] |
| 1   | 1000847845211000960 | 14196021   | -                     | 16.65 |
| 2   | 1030011910101662336 | 467154863  | -                     | 12.56 |
| 3   | 1082306439760980224 | 284473271  | -                     | 16.95 |
| 4   | 1113516077316307328 | 468921975  | -                     | 17.32 |
| 5   | 1131845245388039296 | 459183003  | -                     | 14.38 |
| 6   | 1282064440985835520 | 284710916  | -                     | 16.95 |
| 7   | 1283952955284393600 | 156692387  | -                     | 15.02 |
| 8   | 130950323040219648  | 21129678   | TYC 1778-656-1        | 12.01 |
| 9   | 1328061822746706304 | 57189413   | Pul-3 1330158         | 13.31 |
| 10  | 1360408252238042752 | 1270841916 | CI* NGC 6341 BUON 252 | 16.48 |
| 11  | 1360408767637438080 | 334899753  | CI* NGC 6341 BUON 66  | 15.35 |
| 12  | 1434391228573931264 | 233683339  | TYC 4198-1477-1       | 11.28 |
| 13  | 1469334528442227840 | 321422994  | -                     | 7.69  |
| 14  | 1604817455025097344 | 441702643  | HD 234128             | 9.60  |
| 15  | 1638914513192572160 | 233234760  | -                     | 13.43 |
| 16  | 1651395756874523008 | 422828506  | -                     | 15.20 |
| 17  | 1674177633505987456 | 154181415  | -                     | 11.81 |
| 18  | 1702017371000775552 | 257024839  | -                     | 11.98 |
| 19  | 1705399782300977152 | 288381017  | -                     | 13.35 |
| 20  | 1816360468564136576 | 305026640  | -                     | 15.73 |
| 21  | 1816806080004760704 | 210175404  | HD 195052             | 7.82  |
| 22  | 1816862636135969280 | 1943342821 | -                     | 16.32 |
| 23  | 1838024764630531328 | 289365711  | -                     | 15.22 |
| 24  | 1840250103149876608 | 298564459  | -                     | 16.79 |
| 25  | 1840545974854882688 | 13487952   | -                     | 13.45 |
| 26  | 1840900567357062272 | 126684646  | -                     | 14.28 |
| 27  | 1844828954902210432 | 126816868  | TYC 2181-560-1        | 11.04 |
| 28  | 1856239892738299648 | 282366186  | -                     | 12.40 |
| 29  | 1858179152070142976 | 282642055  | -                     | 13.64 |
| 30  | 1866242184378162048 | 428637082  | -                     | 14.47 |
| 31  | 1902885642747681920 | 10596964   | -                     | 12.57 |
| 32  | 1905945029554316928 | 274959728  | -                     | 12.69 |
| 33  | 1907427072447704960 | 128344724  | HD 213872             | 8.04  |
| 34  | 1922534396571551616 | 177398591  | -                     | 12.63 |
| 35  | 1935962732084366464 | 154818955  | -                     | 14.50 |
| 36  | 1947213794055843968 | 426980319  | TYC 2721-1981-1       | 12.44 |
| 37  | 1949931718078029568 | 256780975  | -                     | 14.15 |
| 38  | 1952552850720372608 | 407657373  | -                     | 10.52 |
| 39  | 1953746748550072832 | 304964668  | -                     | 14.23 |
| 40  | 1956067920673737984 | 256787183  | -                     | 14.95 |
| 41  | 1957707460011110528 | 120350727  | TYC 3208-2231-1       | 10.45 |
| 42  | 1966389105045721728 | 372181882  | -                     | 14.75 |
| 43  | 1966708135217729536 | 372019870  | -                     | 13.21 |

|    |                     |            |                 |       |
|----|---------------------|------------|-----------------|-------|
| 44 | 1976684382179745408 | 326709788  | -               | 13.26 |
| 45 | 1976690257695008768 | 326709771  | -               | 12.90 |
| 46 | 1979662856104556160 | 384526802  | -               | 12.32 |
| 47 | 1979663676424477440 | 384371809  | -               | 16.91 |
| 48 | 1985566168380916352 | 252527111  | -               | 15.50 |
| 49 | 1988555431256785280 | 66784249   | -               | 9.65  |
| 50 | 1997600284486738048 | 345216390  | TYC 4004-623-1  | 12.19 |
| 51 | 2000070891422764032 | 197577843  | -               | 9.63  |
| 52 | 2001383845748574080 | 197498139  | -               | 13.77 |
| 53 | 2039165023782110976 | 403535217  | -               | 14.40 |
| 54 | 2039459211857522304 | 29714517   | -               | 15.91 |
| 55 | 2040412179197363712 | 358598846  | -               | 15.35 |
| 56 | 2042199980805751040 | 28858091   | TYC 2638-2020-1 | 11.47 |
| 57 | 2045244429748163840 | 1873354675 | -               | 16.94 |
| 58 | 2045509721277230976 | 40171580   | -               | 13.49 |
| 59 | 2071550520297992064 | 188973040  | -               | 12.75 |
| 60 | 2072904019124529152 | 239219717  | HD 187235       | 5.81  |
| 61 | 2079637668837248128 | 271667164  | -               | 13.87 |
| 62 | 2083565807263743232 | 193863015  | -               | 16.80 |
| 63 | 2086094344713343104 | 364760486  | -               | 12.64 |
| 64 | 2086094344713345152 | 364760507  | -               | 10.04 |
| 65 | 2088226606998576768 | 295210915  | -               | 16.00 |
| 66 | 2088337657672346880 | 405934076  | -               | 17.83 |
| 67 | 2088337760751570816 | 405934050  | -               | 15.25 |
| 68 | 2088590098668256512 | 351295092  | -               | 12.81 |
| 69 | 2089872743397880192 | 425914150  | -               | 11.92 |
| 70 | 2091168178555456128 | 27851503   | BD+32 3155      | 9.34  |
| 71 | 2091796510791838976 | 68673212   | -               | 15.58 |
| 72 | 2092946191936357504 | 120634210  | TYC 2652-1462-1 | 11.08 |
| 73 | 2105585387334115712 | 158424784  | -               | 15.80 |
| 74 | 2105585417396240128 | 158424726  | GSC 03128-00751 | 12.22 |
| 75 | 2109975423726130944 | 289531891  | BD+39 3466      | 9.19  |
| 76 | 2126055373267136896 | 159448824  | -               | 15.94 |
| 77 | 2126207239009923840 | 159649131  | -               | 12.36 |
| 78 | 2128309715701366016 | 1882735974 | -               | 20.11 |
| 79 | 2129989047910369408 | 417677656  | TYC 3551-2105-1 | 11.50 |
| 80 | 2167371859151737600 | 195728444  | -               | 13.36 |
| 81 | 2174334310379160704 | 341441182  | TYC 3967-834-1  | 11.71 |
| 82 | 2198794900730810752 | 330843238  | TYC 3990-344-1  | 12.23 |
| 83 | 2218305601428687488 | 411577735  | -               | 17.48 |
| 84 | 2221479096922886400 | 305721904  | TYC 4259-2305-1 | 9.88  |
| 85 | 2233741885685321856 | 417763980  | TYC 4606-830-1  | 11.75 |
| 86 | 2236210667244575616 | 233793054  | TYC 3948-543-1  | 10.04 |
| 87 | 2239899975434050304 | 229974469  | -               | 12.45 |
| 88 | 2243609177912239744 | 467268412  | -               | 12.74 |
| 89 | 2247928334463557248 | 269701741  | TYC 4244-667-1  | 11.45 |

|     |                     |           |                 |       |
|-----|---------------------|-----------|-----------------|-------|
| 90  | 2260987504646338944 | 259266402 | -               | 15.84 |
| 91  | 2261059939271215872 | 259170046 | -               | 12.94 |
| 92  | 2271591748837314304 | 387678271 | TYC 4464-728-1  | 10.76 |
| 93  | 2276592052842180352 | 336104507 | TYC 4468-121-1  | 10.44 |
| 94  | 2288995506076455296 | 237211570 | -               | 14.81 |
| 95  | 285301831226772608  | 66571077  | TYC 4079-738-1  | 11.24 |
| 96  | 2919889883618032000 | 172410940 | -               | 14.67 |
| 97  | 2921500668156916480 | 62973790  | TYC 6526-2198-1 | 11.47 |
| 98  | 2922129103469130624 | 172925309 | -               | 17.68 |
| 99  | 2922539500489285760 | 79689505  | -               | 13.04 |
| 100 | 2926097721968343040 | 78442502  | TYC 5962-2598-1 | 11.38 |
| 101 | 2926300689244267648 | 48404603  | -               | 14.87 |
| 102 | 2978112941316016640 | 121549920 | -               | 12.85 |
| 103 | 3006362899727839360 | 443326977 | -               | 13.15 |
| 104 | 3016508540192797312 | 388851561 | -               | 11.83 |
| 105 | 3026543507950724224 | 139785175 | -               | 13.32 |
| 106 | 3027974247455060096 | 385874363 | TYC 5966-1776-1 | 11.35 |
| 107 | 3047771534128902912 | 752215671 | TYC 5395-1656-1 | 11.56 |
| 108 | 3047774184129924992 | 187591950 | -               | 12.88 |
| 109 | 3051988818354158464 | 178430962 | TYC 4827-3532-1 | 12.41 |
| 110 | 3053792429743638016 | 403672868 | TYC 5396-3209-1 | 11.51 |
| 111 | 3055411117015344512 | 5773753   | -               | 14.30 |
| 112 | 3056100820041073280 | 65881563  | HD 61235        | 9.46  |
| 113 | 3056676929773971968 | 68060528  | -               | 11.67 |
| 114 | 3061211728044506880 | 65674883  | -               | 14.82 |
| 115 | 3062196821743114624 | 64670889  | TYC 4817-751-1  | 10.49 |
| 116 | 3070438211146027776 | 88792275  | -               | 12.61 |
| 117 | 3084066520334453376 | 73036564  | -               | 13.56 |
| 118 | 3100012703114696448 | 25699555  | -               | 15.68 |
| 119 | 3108411661982016256 | 5097023   | HD 293472       | 10.93 |
| 120 | 3108411700641725056 | 5096969   | -               | 16.50 |
| 121 | 3108438118980557824 | 5010732   | TYC 4819-2200-1 | 12.49 |
| 122 | 3109216813729774464 | 4999366   | -               | 13.82 |
| 123 | 3110017984051675776 | 51061955  | HD 293718       | 9.02  |
| 124 | 3111017714997000960 | 51066424  | -               | 13.62 |
| 125 | 3111784723136614272 | 284130265 | TYC 163-370-1   | 11.69 |
| 126 | 3116446416218903424 | 291962592 | -               | 14.74 |
| 127 | 3127189194580973184 | 234117193 | -               | 14.84 |
| 128 | 3136176838843608064 | 318054832 | TYC 169-1547-1  | 12.01 |
| 129 | 3137171179610535680 | 280225751 | -               | 13.39 |
| 130 | 3142055966173525376 | 234479702 | -               | 16.11 |
| 131 | 3142606168664447872 | 425203302 | HD 58406        | 9.62  |
| 132 | 3155186677630598144 | 264415524 | -               | 16.42 |
| 133 | 3157513897070802688 | 235515258 | -               | 13.79 |
| 134 | 3159937426855164800 | 262753655 | -               | 10.52 |
| 135 | 3163191397157535872 | 14562651  | TYC 772-1061-1  | 10.46 |

|     |                     |            |                 |       |
|-----|---------------------|------------|-----------------|-------|
| 136 | 3167805527768856192 | 440828323  | -               | 12.74 |
| 137 | 3239171735149435392 | 455040026  | -               | 12.39 |
| 138 | 3463190464736303232 | 107116441  | HD 106098       | 7.19  |
| 139 | 3480090370771578112 | 293110371  | -               | 13.98 |
| 140 | 3573965677119301888 | 335499532  | -               | 14.17 |
| 141 | 380338531092181888  | 288292934  | -               | 13.05 |
| 142 | 4035494856994650368 | 326268416  | -               | 15.66 |
| 143 | 4035812783290341760 | 328311189  | HD 164821       | 9.81  |
| 144 | 4035962321234280448 | 330361794  | -               | 14.68 |
| 145 | 4035966341325506432 | 331426373  | -               | 16.44 |
| 146 | 4035985307902284416 | 331123166  | -               | 16.39 |
| 147 | 4036508297507715968 | 112582374  | -               | 15.77 |
| 148 | 4037072656228219264 | 326580683  | -               | 14.10 |
| 149 | 4037933603783337088 | 332183980  | -               | 13.33 |
| 150 | 4037950203918200192 | 368989688  | HD 321512       | 9.61  |
| 151 | 4037952609100471680 | 368875977  | -               | 16.20 |
| 152 | 4037958622055212800 | 332192081  | -               | 16.34 |
| 153 | 4038034896294274176 | 58111564   | TYC 7404-5579-1 | 11.63 |
| 154 | 4038509271213133952 | 63620022   | HD 321646       | 10.09 |
| 155 | 4038805241630001152 | 56585584   | -               | 14.84 |
| 156 | 4039236873066049536 | 57381069   | HD 321392       | 10.54 |
| 157 | 4039334076674100736 | 1562101847 | -               | 16.52 |
| 158 | 4044583175232151040 | 64501119   | -               | 14.67 |
| 159 | 4045364756241734272 | 61555986   | -               | 14.40 |
| 160 | 4045508590453650304 | 1572480613 | -               | 17.87 |
| 161 | 4045542086809684224 | 64238011   | -               | 14.68 |
| 162 | 4046523985053304320 | 405191861  | -               | 14.00 |
| 163 | 4046542681094780160 | 273001069  | -               | 12.96 |
| 164 | 4046775159100879232 | 28512009   | -               | 15.16 |
| 165 | 4046872568966494208 | 197159291  | HD 170460       | 9.78  |
| 166 | 4047904598101613952 | 1579368307 | -               | 16.01 |
| 167 | 408300245661632640  | 370996738  | -               | 16.07 |
| 168 | 408510011862975360  | 71982139   | TYC 3671-919-1  | 11.39 |
| 169 | 412545116464742144  | 333068770  | TYC 3678-1252-1 | 11.09 |
| 170 | 423505288886486144  | 604540729  | -               | 16.52 |
| 171 | 431402909113148672  | 359433277  | -               | 12.07 |
| 172 | 431584053656972160  | 283020417  | -               | 12.86 |
| 173 | 438583819545499520  | 428055283  | -               | 8.62  |
| 174 | 4502102302993009408 | 150398632  | -               | 16.15 |
| 175 | 4510985463605954176 | 298514766  | -               | 12.73 |
| 176 | 4527438345131259392 | 256115545  | TYC 1575-286-1  | 11.77 |
| 177 | 4532553414971302144 | 314483554  | -               | 12.71 |
| 178 | 4545156017236737408 | 400110989  | -               | 13.50 |
| 179 | 4567834269195235840 | 150599880  | -               | 16.32 |
| 180 | 4577858379269507840 | 275486706  | -               | 16.80 |
| 181 | 4589093940696193024 | 377682645  | -               | 16.94 |

|     |                     |           |                 |       |
|-----|---------------------|-----------|-----------------|-------|
| 182 | 4592018955162562048 | 24261146  | -               | 8.74  |
| 183 | 4692539984661757952 | 52153898  | -               | 12.87 |
| 184 | 4702811313050760064 | 39017347  | -               | 15.17 |
| 185 | 4762428822077310336 | 220461517 | HD 32475        | 8.75  |
| 186 | 480943295278953600  | 321105654 | -               | 8.91  |
| 187 | 4825484168959858560 | 1527210   | -               | 16.14 |
| 188 | 4909378967742430976 | 206564278 | -               | 13.82 |
| 189 | 5190966816196033280 | 383260696 | -               | 13.39 |
| 190 | 5194902586786637312 | 389013472 | -               | 12.46 |
| 191 | 5199247577564534784 | 394563932 | HD 90982        | 10.11 |
| 192 | 5201664579001450880 | 394238292 | -               | 15.41 |
| 193 | 5206159077597140736 | 453363852 | -               | 13.99 |
| 194 | 5210030045718111232 | 272472682 | -               | 14.42 |
| 195 | 5217109010817884160 | 288067102 | -               | 14.12 |
| 196 | 5217848020071003136 | 452591808 | -               | 14.03 |
| 197 | 5218949490203154944 | 452385022 | -               | 15.65 |
| 198 | 5220930947593836544 | 287430039 | -               | 14.41 |
| 199 | 5224132377558954368 | 302525126 | -               | 13.26 |
| 200 | 5228454218476267264 | 401597729 | TYC 9229-1045-1 | 11.72 |
| 201 | 5230268172140395264 | 453888710 | TYC 9218-2243-1 | 11.87 |
| 202 | 5232514783638765696 | 397264934 | HD 91441        | 7.91  |
| 203 | 5233348350893189120 | 296945692 | TYC 9230-1986-1 | 12.01 |
| 204 | 5233397313514281088 | 410982255 | TYC 9230-650-1  | 11.50 |
| 205 | 5235188383612093952 | 295283974 | HD 99086        | 9.50  |
| 206 | 5235188452331574272 | 295386839 | -               | 15.34 |
| 207 | 5235795898154393344 | 392616391 | -               | 16.99 |
| 208 | 5237830888006515840 | 400839754 | -               | 16.77 |
| 209 | 5239154115889810304 | 397786565 | -               | 14.18 |
| 210 | 5239571307519022336 | 465456405 | -               | 12.30 |
| 211 | 5244004783224269056 | 371323853 | -               | 13.19 |
| 212 | 5244874496924635008 | 373034540 | -               | 14.13 |
| 213 | 5246146150844814336 | 845838161 | -               | 13.94 |
| 214 | 5249563295545865600 | 269540771 | -               | 13.49 |
| 215 | 5249644075292765440 | 363534697 | -               | 16.29 |
| 216 | 5249773989468645120 | 269544397 | -               | 13.48 |
| 217 | 5249774058188121472 | 269544423 | -               | 15.52 |
| 218 | 5249774058188133248 | 269544452 | TYC 8946-869-1  | 12.37 |
| 219 | 5249895691657856000 | 362592863 | -               | 13.25 |
| 220 | 5250398580780583936 | 360387688 | HD 309665       | 9.69  |
| 221 | 5250674210296043264 | 362097981 | -               | 13.48 |
| 222 | 5250674558204518912 | 362098098 | -               | 13.36 |
| 223 | 5251560936384991360 | 378037013 | -               | 15.61 |
| 224 | 5252355913334145280 | 376414794 | -               | 12.45 |
| 225 | 5252903165213946112 | 378027065 | -               | 15.09 |
| 226 | 5252999956602261888 | 377576240 | -               | 16.79 |
| 227 | 5253245727475264512 | 375746688 | -               | 12.86 |

|     |                     |           |                 |       |
|-----|---------------------|-----------|-----------------|-------|
| 228 | 5253647049219382656 | 390094806 | -               | 12.26 |
| 229 | 5253918907816065920 | 460863280 | -               | 12.66 |
| 230 | 5254015424324222464 | 390685381 | -               | 13.67 |
| 231 | 5254701687028855936 | 378325663 | -               | 13.08 |
| 232 | 5255832332903758720 | 270086297 | -               | 16.50 |
| 233 | 5256736608175848064 | 462454808 | -               | 12.51 |
| 234 | 5256736715584377216 | 462454742 | -               | 12.84 |
| 235 | 5257667516570866304 | 469248153 | -               | 12.19 |
| 236 | 5257714559351263104 | 444544916 | HD 302393       | 10.52 |
| 237 | 5258319600000641920 | 462170260 | -               | 13.03 |
| 238 | 5269596088153228032 | 306472729 | -               | 15.93 |
| 239 | 5279289657541807488 | 176932559 | -               | 13.96 |
| 240 | 5280371954942137856 | 176935274 | -               | 16.52 |
| 241 | 5285464377404209792 | 167811160 | -               | 16.34 |
| 242 | 5290692589556889984 | 410449364 | -               | 16.90 |
| 243 | 5291112018881767168 | 341330235 | -               | 16.15 |
| 244 | 5293139587041400960 | 349192518 | -               | 14.68 |
| 245 | 5296549550559148416 | 356207241 | -               | 13.90 |
| 246 | 5298070106425032192 | 357117415 | -               | 15.56 |
| 247 | 5298070243863883008 | 357117414 | TYC 8931-1063-1 | 12.05 |
| 248 | 5298391232540840064 | 357120271 | -               | 16.14 |
| 249 | 5299425426314526976 | 358985523 | -               | 15.96 |
| 250 | 5300038988157555456 | 357384071 | CD-59 2246      | 9.29  |
| 251 | 5300161652426240768 | 384718194 | TYC 8595-1266-1 | 11.76 |
| 252 | 5303780351357356416 | 385004580 | -               | 13.26 |
| 253 | 5304687654602821760 | 383733821 | HD 77525        | 8.52  |
| 254 | 5304725037999367808 | 384032429 | -               | 17.16 |
| 255 | 5305259503734864640 | 361064918 | -               | 16.73 |
| 256 | 5311211435055179264 | 384357648 | HD 78270        | 9.62  |
| 257 | 5314453413792262784 | 118083764 | TYC 8580-714-1  | 11.10 |
| 258 | 5317639592333952768 | 118542507 | -               | 12.85 |
| 259 | 5319790408875602688 | 139830552 | -               | 14.32 |
| 260 | 5322521149082732800 | 388622617 | -               | 14.27 |
| 261 | 5322521939356695680 | 388622573 | -               | 12.90 |
| 262 | 5329579463992281728 | 28796337  | -               | 13.58 |
| 263 | 5329579567071497216 | 28796280  | TYC 8155-83-1   | 12.74 |
| 264 | 5329580254266248704 | 28796311  | TYC 8155-1797-1 | 11.52 |
| 265 | 5336022185498555008 | 315841896 | HD 99416        | 8.82  |
| 266 | 5340301248569279744 | 307871938 | -               | 17.08 |
| 267 | 5341595820423958528 | 300685428 | -               | 13.05 |
| 268 | 5342223332326015616 | 268256646 | -               | 14.98 |
| 269 | 5344290826485249920 | 376272735 | -               | 16.58 |
| 270 | 5347227244092635776 | 306746627 | -               | 12.73 |
| 271 | 5347816273079223808 | 80851607  | -               | 12.64 |
| 272 | 5347816444877964032 | 81013420  | -               | 16.51 |
| 273 | 5348815969664011008 | 91909726  | HD 99641        | 8.80  |

|     |                     |           |                 |       |
|-----|---------------------|-----------|-----------------|-------|
| 274 | 5355588961316766080 | 464339039 | -               | 13.61 |
| 275 | 5355945993339266560 | 862309155 | -               | 17.34 |
| 276 | 5355946096418485120 | 463006054 | -               | 15.18 |
| 277 | 5355946298267024384 | 463006006 | -               | 13.39 |
| 278 | 5357218162655743616 | 448119771 | -               | 16.88 |
| 279 | 5361576454936896768 | 80682970  | -               | 13.30 |
| 280 | 5363099347257022976 | 147188371 | -               | 15.92 |
| 281 | 5365037511384979840 | 446463051 | TYC 8188-4047-1 | 12.17 |
| 282 | 5365504906900658560 | 103455699 | -               | 14.58 |
| 283 | 5365569400131030784 | 103184931 | -               | 14.71 |
| 284 | 5365758133870284160 | 103064288 | -               | 16.67 |
| 285 | 5366164442080271360 | 146721958 | -               | 14.99 |
| 286 | 5368624599351986944 | 389092347 | -               | 12.83 |
| 287 | 5369134287408073088 | 400864696 | -               | 16.00 |
| 288 | 5369143671916118912 | 389094756 | -               | 14.59 |
| 289 | 537697439806050944  | 407425104 | -               | 12.43 |
| 290 | 5377737862811124480 | 61986506  | -               | 12.41 |
| 291 | 5383924166203787904 | 152484511 | HD 99627        | 7.30  |
| 292 | 5388173843068686336 | 941392385 | -               | 19.58 |
| 293 | 5388590253034578560 | 72063751  | -               | 14.26 |
| 294 | 5391470698617696768 | 147136087 | TYC 7731-706-1  | 10.77 |
| 295 | 5402896136260022144 | 57185763  | -               | 16.11 |
| 296 | 5407149042941626624 | 259660452 | -               | 17.48 |
| 297 | 5407636371416522240 | 375435567 | -               | 13.55 |
| 298 | 5407683822215685632 | 375369028 | TYC 8187-1501-1 | 10.70 |
| 299 | 5408609851521792896 | 36386815  | -               | 13.79 |
| 300 | 5416786472816800512 | 101915841 | -               | 13.46 |
| 301 | 5418855543243042688 | 286999395 | -               | 18.77 |
| 302 | 5430272154731627904 | 3589729   | -               | 12.39 |
| 303 | 5430326305680776064 | 3354992   | -               | 16.43 |
| 304 | 5430557645496482048 | 3120296   | -               | 13.92 |
| 305 | 5430605031878495360 | 3120227   | -               | 13.45 |
| 306 | 5432279862961052416 | 44692620  | -               | 15.30 |
| 307 | 5433007323043969152 | 44306559  | -               | 16.56 |
| 308 | 5439868692214398464 | 11932252  | -               | 12.38 |
| 309 | 5449580158729020928 | 48942631  | -               | 15.48 |
| 310 | 5456955480866179456 | 363348244 | -               | 13.82 |
| 311 | 546757754916703232  | 396013343 | -               | 11.85 |
| 312 | 5477102176019196032 | 372851666 | -               | 15.67 |
| 313 | 5478585722145655680 | 150441810 | HD 46698        | 9.94  |
| 314 | 5487126114292844544 | 339768609 | -               | 13.19 |
| 315 | 5493350788917805056 | 766897407 | -               | 18.76 |
| 316 | 5496278346002206848 | 260538568 | -               | 12.92 |
| 317 | 5506584721326844800 | 445388907 | -               | 13.65 |
| 318 | 5507683339601282048 | 60608976  | -               | 17.28 |
| 319 | 5510486235259342080 | 59757295  | CD-46 3075      | 9.85  |

|     |                     |           |                         |       |
|-----|---------------------|-----------|-------------------------|-------|
| 320 | 5511237098622640256 | 60500408  | -                       | 15.08 |
| 321 | 5518789399175413376 | 79853526  | HD 66815                | 9.55  |
| 322 | 5520448497807830016 | 80804861  | -                       | 15.14 |
| 323 | 5520454373323099136 | 80804874  | -                       | 14.17 |
| 324 | 5521176133980907136 | 81427818  | 2MASS J08123971-4331202 | 10.57 |
| 325 | 5531436913935633408 | 143732705 | -                       | 12.68 |
| 326 | 5532057038490253824 | 123566367 | CD-44 3650              | 10.18 |
| 327 | 5532742098656703744 | 79798831  | -                       | 14.53 |
| 328 | 5543711105839749120 | 55513750  | -                       | 15.83 |
| 329 | 5551496060467574912 | 237974015 | -                       | 16.55 |
| 330 | 5562578209963553280 | 130571889 | -                       | 15.47 |
| 331 | 5578307823311195008 | 157307309 | -                       | 17.19 |
| 332 | 5594201298258640896 | 152683130 | -                       | 13.02 |
| 333 | 5594391307611575680 | 151005187 | TYC 7123-1718-1         | 10.83 |
| 334 | 5596703408773397248 | 154072038 | -                       | 13.49 |
| 335 | 559796485354538368  | 289267282 | -                       | 17.56 |
| 336 | 5601882928863475200 | 127257401 | TYC 6548-2955-1         | 10.85 |
| 337 | 5602460932697430400 | 128336946 | TYC 6557-3270-1         | 12.52 |
| 338 | 5603319548182261120 | 98487738  | TYC 7107-177-1          | 11.22 |
| 339 | 5607595858139420416 | 97198226  | -                       | 15.04 |
| 340 | 5610444074293395840 | 63475004  | HD 52618                | 8.93  |
| 341 | 5610727198532209536 | 63195379  | -                       | 13.83 |
| 342 | 5611300662572691584 | 63884938  | -                       | 16.51 |
| 343 | 5611676523755321984 | 109931495 | -                       | 14.49 |
| 344 | 5615672595688333440 | 140535818 | -                       | 13.60 |
| 345 | 562049865716101376  | 399797801 | -                       | 15.77 |
| 346 | 5624566648316617216 | 18658764  | -                       | 14.21 |
| 347 | 5629302588495037696 | 186976949 | -                       | 13.39 |
| 348 | 5637827617537477504 | 70506669  | -                       | 17.62 |
| 349 | 5639067729223791488 | 47791970  | -                       | 13.69 |
| 350 | 5644257561549251712 | 147520378 | -                       | 12.24 |
| 351 | 5653584783097189376 | 941297    | -                       | 15.32 |
| 352 | 5674641358481222528 | 189106923 | TYC 6588-537-1          | 12.62 |
| 353 | 5693570585029021184 | 196318935 | -                       | 15.00 |
| 354 | 5695944469291999488 | 271381183 | TYC 6560-3528-1         | 11.39 |
| 355 | 5696368777700914048 | 156466107 | TYC 6556-175-1          | 11.11 |
| 356 | 5698291445592304640 | 129923311 | -                       | 13.59 |
| 357 | 5698379406514785792 | 153030345 | TYC 6558-1725-1         | 9.87  |
| 358 | 5709005597974727424 | 1103460   | UCAC4 364-048648        | 11.76 |
| 359 | 5709873902923076480 | 386435525 | TYC 6011-1986-1         | 11.87 |
| 360 | 5713928459432507776 | 11070498  | -                       | 15.04 |
| 361 | 5715415651991150592 | 415273187 | TYC 5992-124-1          | 10.11 |
| 362 | 5719128874546370048 | 54221871  | -                       | 13.92 |
| 363 | 5723694661005331968 | 386315293 | HD 72009                | 10.42 |
| 364 | 5725554072607426944 | 54391224  | -                       | 13.31 |
| 365 | 5767544937068977792 | 451530226 | -                       | 17.18 |



|     |                     |            |                 |       |
|-----|---------------------|------------|-----------------|-------|
| 366 | 5775032439453787008 | 384294161  | -               | 11.31 |
| 367 | 5777941369263751808 | 310102139  | CD-76 839       | 10.73 |
| 368 | 5778066851029502720 | 310270073  | -               | 12.75 |
| 369 | 5778256211845370880 | 407221993  | -               | 13.98 |
| 370 | 5784814317670524672 | 269981015  | -               | 17.33 |
| 371 | 5788454766310233856 | 357784273  | -               | 13.50 |
| 372 | 5788543345715149440 | 357208790  | -               | 14.48 |
| 373 | 5790689111380619136 | 395329193  | HD 119034       | 9.81  |
| 374 | 5792895968654169216 | 402513601  | -               | 15.68 |
| 375 | 5793593540067556992 | 403078542  | TYC 9270-1649-1 | 11.03 |
| 376 | 5794445936453527936 | 426061785  | -               | 16.64 |
| 377 | 5795863756701627008 | 263349964  | -               | 14.57 |
| 378 | 5796024388480978688 | 263670290  | -               | 12.49 |
| 379 | 5796414234067241344 | 396648272  | -               | 16.14 |
| 380 | 5796639359075316096 | 401617111  | -               | 11.41 |
| 381 | 5797130909493417856 | 258489335  | -               | 15.51 |
| 382 | 5799205928463730176 | 263090069  | TYC 9259-3165-1 | 12.15 |
| 383 | 5799206061588435712 | 263090180  | -               | 14.66 |
| 384 | 5799206237701417984 | 263024559  | -               | 13.78 |
| 385 | 5799225234318798592 | 262833444  | -               | 16.62 |
| 386 | 5799930055632056576 | 257478985  | TYC 9257-1957-1 | 12.34 |
| 387 | 5800138898442465408 | 260829757  | -               | 15.16 |
| 388 | 5800337944401826176 | 1107800063 | -               | 17.86 |
| 389 | 5800601140011484800 | 260335322  | TYC 9032-826-1  | 12.07 |
| 390 | 5802848747907559680 | 310799640  | -               | 16.90 |
| 391 | 5803207085617950080 | 343296059  | HD 159537       | 9.36  |
| 392 | 5804243753285260032 | 311529705  | -               | 14.24 |
| 393 | 5804719773101604480 | 293578567  | -               | 15.02 |
| 394 | 5805333128790293248 | 310507162  | HD 150995       | 6.72  |
| 395 | 5807013732317147520 | 363454805  | TYC 9278-2110-1 | 10.06 |
| 396 | 5808932345752452992 | 362325680  | -               | 17.97 |
| 397 | 5809843291127745920 | 294886947  | -               | 16.44 |
| 398 | 5811904664972614016 | 295167241  | TYC 9289-2657-1 | 11.48 |
| 399 | 5814141969281504256 | 304663375  | -               | 14.89 |
| 400 | 5816413319790133632 | 301747913  | -               | 15.43 |
| 401 | 5817506612303659136 | 290814065  | -               | 16.55 |
| 402 | 5818570527244766720 | 447471894  | -               | 14.72 |
| 403 | 5818655223992687872 | 426236341  | -               | 14.53 |
| 404 | 5820176741939755008 | 447006364  | -               | 15.07 |
| 405 | 5820202992777101696 | 263606058  | HD 138774       | 9.75  |
| 406 | 5820219756023237248 | 263303021  | -               | 16.36 |
| 407 | 5821726915896666624 | 362475056  | -               | 16.46 |
| 408 | 5822579862054689536 | 340169117  | -               | 15.81 |
| 409 | 5822944178356346112 | 341225454  | -               | 12.45 |
| 410 | 5824276442865076864 | 271315403  | -               | 15.05 |
| 411 | 5824303174727833344 | 261694578  | TYC 9258-200-1  | 12.32 |

|     |                     |            |                  |       |
|-----|---------------------|------------|------------------|-------|
| 412 | 5824483047942228224 | 262927909  | -                | 14.81 |
| 413 | 5824483803880454016 | 262920132  | -                | 15.03 |
| 414 | 5825168456035683712 | 455603263  | -                | 16.23 |
| 415 | 5825443677527219072 | 426908146  | TYC 9035-1908-1  | 11.31 |
| 416 | 5825554762564785536 | 424717153  | -                | 16.22 |
| 417 | 5825857742410471296 | 423768896  | CD-63 1109       | 9.99  |
| 418 | 5826738558638797568 | 423016159  | -                | 16.86 |
| 419 | 5827889712932154240 | 350847864  | -                | 15.64 |
| 420 | 5828087350145667584 | 350181335  | -                | 16.34 |
| 421 | 5828087414548565248 | 350181374  | -                | 18.08 |
| 422 | 5828964446873245568 | 1209068824 | -                | 19.68 |
| 423 | 5829429029220366080 | 299981629  | TYC 9041-1147-1  | 11.04 |
| 424 | 5829521422558317824 | 300763561  | -                | 16.66 |
| 425 | 5830401031864509568 | 402700560  | -                | 14.92 |
| 426 | 5831076441242048128 | 350362794  | -                | 13.00 |
| 427 | 5831076475601780736 | 350362747  | -                | 16.13 |
| 428 | 5831694469872120192 | 220771986  | -                | 16.40 |
| 429 | 5831767175069679232 | 221301041  | HD 148274        | 9.91  |
| 430 | 5831770198726668672 | 221301000  | -                | 17.00 |
| 431 | 5831867093193021440 | 221047381  | -                | 16.40 |
| 432 | 5832178181917965312 | 342360998  | TYC 9040-3548-1  | 11.70 |
| 433 | 5832312223592928896 | 343364326  | -                | 15.49 |
| 434 | 5833922900716496512 | 79909417   | -                | 15.90 |
| 435 | 5839006119071807488 | 393976075  | -                | 13.34 |
| 436 | 584063742066442752  | 323568463  | -                | 14.96 |
| 437 | 5841069417058281472 | 1006325065 | -                | 19.05 |
| 438 | 5841981878580983552 | 361390488  | TYC 9249-2331-1  | 10.14 |
| 439 | 5841982084739411200 | 361390493  | -                | 13.53 |
| 440 | 5843275282210787840 | 328023891  | -                | 14.13 |
| 441 | 5843566515357941632 | 338135641  | -                | 16.04 |
| 442 | 5843658526423693056 | 338140307  | -                | 12.78 |
| 443 | 5843724192198636416 | 334999132  | UCAC4 094-038759 | 15.48 |
| 444 | 5844979628330042624 | 957834257  | -                | 18.42 |
| 445 | 5846837081417998464 | 448256778  | -                | 17.41 |
| 446 | 5848704052181083136 | 259019132  | -                | 12.30 |
| 447 | 5848820119348047104 | 258611491  | HD 129795        | 7.18  |
| 448 | 5852288734995264640 | 324848407  | -                | 17.16 |
| 449 | 5853426798239031680 | 391290143  | TYC 9010-2235-1  | 11.62 |
| 450 | 5855029233312493184 | 312804529  | -                | 15.64 |
| 451 | 5856141011373319808 | 311842027  | -                | 12.98 |
| 452 | 5857083499007737984 | 336944517  | TYC 9241-1058-1  | 11.84 |
| 453 | 5859739261936071424 | 448017139  | -                | 17.64 |
| 454 | 5859931371593518592 | 328842239  | -                | 14.79 |
| 455 | 5860660313399084160 | 312576659  | HD 311107        | 10.55 |
| 456 | 5864236165807073920 | 318720437  | -                | 12.43 |
| 457 | 5872653958042032896 | 208837337  | -                | 14.74 |

|     |                     |            |                 |       |
|-----|---------------------|------------|-----------------|-------|
| 458 | 5876767054916225792 | 44278854   | -               | 12.71 |
| 459 | 5878437350517780224 | 392646027  | TYC 9006-4210-1 | 12.60 |
| 460 | 5884832080091884416 | 75708361   | HD 140926       | 7.90  |
| 461 | 5886387236217138688 | 46197921   | -               | 11.91 |
| 462 | 5888891167833559552 | 145812196  | -               | 13.09 |
| 463 | 5898674652300978048 | 332556988  | TYC 8289-810-1  | 11.77 |
| 464 | 5899324914661007104 | 446364434  | -               | 15.23 |
| 465 | 5901546271760380288 | 370091739  | -               | 15.19 |
| 466 | 5905131298129266944 | 455319850  | -               | 13.44 |
| 467 | 5905744237191442304 | 128542916  | TYC 8283-3278-1 | 10.73 |
| 468 | 5907618255985223168 | 455389016  | -               | 13.93 |
| 469 | 5909624795984270848 | 306882685  | -               | 16.35 |
| 470 | 5910623186905123584 | 305947198  | -               | 14.00 |
| 471 | 5911440845598524288 | 307232499  | -               | 12.70 |
| 472 | 5911947819235946880 | 306638921  | -               | 16.41 |
| 473 | 5912491875638757632 | 305186122  | -               | 15.91 |
| 474 | 5912875055441832448 | 74183935   | -               | 15.02 |
| 475 | 5913634508733603072 | 290811927  | -               | 17.98 |
| 476 | 5914825550400111104 | 170972841  | -               | 12.16 |
| 477 | 5914963234185748864 | 172886984  | -               | 10.14 |
| 478 | 5915376994141999744 | 171550067  | -               | 14.23 |
| 479 | 5915495603966205568 | 304833926  | -               | 16.06 |
| 480 | 5916147511288645504 | 367746024  | -               | 17.58 |
| 481 | 5916827834113326336 | 172636779  | -               | 15.42 |
| 482 | 5916864972674231552 | 172638589  | -               | 14.98 |
| 483 | 5916995406564505472 | 171213459  | -               | 15.78 |
| 484 | 5917095938833131392 | 171738431  | -               | 16.85 |
| 485 | 5917095977519585920 | 171738397  | -               | 14.58 |
| 486 | 5917446442523385344 | 172808758  | -               | 14.89 |
| 487 | 5917447649435725568 | 1315624260 | -               | 14.43 |
| 488 | 5918720364183373184 | 75668886   | -               | 14.65 |
| 489 | 5918752902855582336 | 337190401  | -               | 12.94 |
| 490 | 5920848507604365952 | 75528597   | -               | 13.66 |
| 491 | 5920911901323727744 | 75305674   | -               | 16.30 |
| 492 | 5921479829134109824 | 73703617   | -               | 16.17 |
| 493 | 5921537901401324928 | 360564991  | -               | 15.10 |
| 494 | 5921549652415516416 | 1513801289 | -               | 15.48 |
| 495 | 5922071198905100544 | 388832000  | HD 158766       | 9.82  |
| 496 | 5922154826191552512 | 323890455  | -               | 13.23 |
| 497 | 5922518597061216384 | 367328654  | -               | 15.30 |
| 498 | 5922784781956302464 | 174123557  | -               | 15.95 |
| 499 | 5923149682376208640 | 366954637  | -               | 13.13 |
| 500 | 5923573028716206592 | 173502035  | -               | 14.80 |
| 501 | 5923721119205695616 | 172147254  | -               | 14.02 |
| 502 | 5924163569544956672 | 213474487  | -               | 16.34 |
| 503 | 5924696454716860544 | 412539248  | -               | 15.00 |

|     |                     |            |                 |       |
|-----|---------------------|------------|-----------------|-------|
| 504 | 5924696828359390336 | 412539380  | -               | 12.09 |
| 505 | 5924999645053714432 | 372665442  | -               | 12.78 |
| 506 | 5924999743808737920 | 372665467  | -               | 12.77 |
| 507 | 5925476592585261696 | 214357475  | -               | 13.46 |
| 508 | 5928428227229284224 | 221969261  | TYC 8720-1555-1 | 11.06 |
| 509 | 5929155902094031872 | 170432176  | -               | 14.25 |
| 510 | 5929340070299722368 | 420831735  | TYC 8717-1756-1 | 10.81 |
| 511 | 5929340139019209344 | 420702904  | -               | 12.45 |
| 512 | 5929422430593544320 | 421060287  | -               | 14.59 |
| 513 | 5929734004701977728 | 171126382  | -               | 15.78 |
| 514 | 5929873088586737536 | 170151063  | -               | 16.71 |
| 515 | 5930376630548681728 | 222186458  | -               | 17.23 |
| 516 | 5945577997280030976 | 255718013  | TYC 8356-449-1  | 11.70 |
| 517 | 5945662114226248704 | 396910578  | -               | 13.07 |
| 518 | 5946192525515577216 | 323887849  | -               | 13.71 |
| 519 | 5946436028662287872 | 388821174  | -               | 13.06 |
| 520 | 5946889718970768512 | 96099359   | -               | 14.87 |
| 521 | 5947682084574955520 | 390088830  | -               | 11.95 |
| 522 | 5947917964185206528 | 21665741   | TYC 8348-2426-1 | 11.75 |
| 523 | 5949608600747742720 | 214249847  | -               | 13.02 |
| 524 | 5949903549070928000 | 1521545773 | -               | 15.70 |
| 525 | 5950530884842606336 | 214020620  | -               | 15.24 |
| 526 | 5951804875224112256 | 218140405  | -               | 15.19 |
| 527 | 5952080822624156928 | 16141385   | -               | 13.61 |
| 528 | 5953858247547530880 | 22889795   | -               | 17.44 |
| 529 | 5954488924867751168 | 24023325   | TYC 8344-261-1  | 12.51 |
| 530 | 5954488959227126528 | 24023230   | TYC 8344-540-1  | 10.62 |
| 531 | 5954623271445151872 | 21998764   | -               | 15.28 |
| 532 | 5956733470452811904 | 23931953   | -               | 14.35 |
| 533 | 5956791851997997568 | 23490938   | -               | 16.10 |
| 534 | 5989131546959071488 | 254564998  | -               | 16.76 |
| 535 | 5989252527604597376 | 254707388  | -               | 15.10 |
| 536 | 5992245844949838208 | 224121346  | -               | 16.74 |
| 537 | 6001063550218208384 | 289875288  | TYC 7848-1485-1 | 10.80 |
| 538 | 6003468452715574528 | 141960970  | TYC 7834-1214-1 | 11.77 |
| 539 | 6004382765347273856 | 307529083  | TYC 7826-2283-1 | 12.44 |
| 540 | 6005939265801701888 | 148264694  | -               | 13.88 |
| 541 | 6008695054261417600 | 295901890  | TYC 7837-1755-1 | 10.57 |
| 542 | 6035804372448412800 | 94927513   | -               | 13.01 |
| 543 | 6052876249006129536 | 380445207  | -               | 12.27 |
| 544 | 6061706151974528384 | 406054872  | -               | 14.39 |
| 545 | 6063408329102740480 | 420279819  | -               | 18.19 |
| 546 | 6063408333426505600 | 420279808  | -               | 16.11 |
| 547 | 6065759325475845376 | 241401813  | -               | 10.35 |
| 548 | 6066422713277072512 | 253380938  | HD 113554       | 9.70  |
| 549 | 6069641941552953600 | 241533827  | -               | 12.64 |

|     |                     |            |                         |       |
|-----|---------------------|------------|-------------------------|-------|
| 550 | 6072952197423163520 | 288022372  | -                       | 14.87 |
| 551 | 6074817209652126976 | 419779192  | -                       | 13.07 |
| 552 | 6075378922666333184 | 398767644  | TYC 8640-3151-1         | 11.53 |
| 553 | 6077029427053289344 | 334215363  | -                       | 14.89 |
| 554 | 6077744521928647040 | 403957442  | -                       | 16.53 |
| 555 | 6083471774916181376 | 425433597  | -                       | 14.79 |
| 556 | 6083675218946850560 | 438598618  | CI* NGC 5139 LEID 69005 | 14.25 |
| 557 | 6083725521608359808 | 438618519  | NGC 5139 6781           | 14.88 |
| 558 | 6085532156618486912 | 169786140  | TYC 8254-1635-1         | 10.71 |
| 559 | 6086922729589821568 | 453773405  | -                       | 16.72 |
| 560 | 6090850112104591616 | 312718329  | -                       | 17.41 |
| 561 | 6092524638257617920 | 242494645  | -                       | 12.38 |
| 562 | 6092765358279494144 | 242410561  | TYC 8268-1377-1         | 11.46 |
| 563 | 6094602951447392768 | 241571032  | -                       | 13.84 |
| 564 | 6095905636508330368 | 242255440  | -                       | 15.07 |
| 565 | 6096794488580041600 | 242275285  | TYC 8264-2468-1         | 11.53 |
| 566 | 6101090521023906304 | 1173099918 | -                       | 18.84 |
| 567 | 6104664208695831424 | 159154997  | -                       | 17.02 |
| 568 | 6126099909446162816 | 332650183  | -                       | 15.71 |
| 569 | 6129139367589740416 | 73087129   | -                       | 16.67 |
| 570 | 6130406627760739584 | 22562145   | -                       | 17.33 |
| 571 | 6134198362329481600 | 248079846  | -                       | 17.13 |
| 572 | 6135749665856729472 | 258516818  | -                       | 16.19 |
| 573 | 6143487964270445696 | 22216722   | -                       | 15.13 |
| 574 | 6148958309495177472 | 165531881  | UCAC4 244-054022        | 12.89 |
| 575 | 6198287928739684736 | 121101104  | -                       | 14.77 |
| 576 | 6365804439402410368 | 387132119  | -                       | 13.70 |
| 577 | 6396977483833892608 | 327667956  | UCAC4 109-123687        | 13.62 |
| 578 | 6421452848890053504 | 1815920520 | -                       | 19.15 |
| 579 | 6423584978033391360 | 396168734  | -                       | 17.48 |
| 580 | 6431145666663098752 | 292621879  | -                       | 12.52 |
| 581 | 6431593889451313152 | 295647609  | -                       | 15.71 |
| 582 | 6432487723686020352 | 295600534  | -                       | 16.17 |
| 583 | 6436684147250254336 | 464315597  | -                       | 15.57 |
| 584 | 6437199371523105920 | 295541199  | CPD-66 3273             | 10.54 |
| 585 | 6442023341352913536 | 339659122  | -                       | 15.01 |
| 586 | 654228110224930688  | 18997902   | -                       | 13.08 |
| 587 | 654228320679849600  | 18997890   | TYC 792-1009-1          | 10.18 |
| 588 | 6558038242037943936 | 231240145  | HD 209142               | 7.71  |
| 589 | 6562425190353962624 | 139896280  | -                       | 13.88 |
| 590 | 6631310315391008896 | 365954182  | -                       | 14.54 |
| 591 | 6635167780139846528 | 365361132  | -                       | 14.56 |
| 592 | 6635283778619600256 | 380918914  | UCAC4 147-218248        | 13.14 |
| 593 | 6636109026511833472 | 120249063  | -                       | 12.75 |
| 594 | 6638185252361580672 | 379406265  | -                       | 15.83 |
| 595 | 6643508847143691648 | 230975443  | HD 180934               | 8.16  |

|     |                     |            |                 |       |
|-----|---------------------|------------|-----------------|-------|
| 596 | 6648008220526387712 | 119220200  | -               | 13.84 |
| 597 | 6648824058154351488 | 76764448   | -               | 15.73 |
| 598 | 6655103025461363328 | 6353630    | -               | 12.79 |
| 599 | 6655226617441445888 | 389576837  | GSC 08371-01874 | 14.22 |
| 600 | 6655267711688555904 | 389576843  | HD 169999       | 10.48 |
| 601 | 6656795002058334080 | 158237379  | TYC 8387-854-1  | 11.96 |
| 602 | 6660045536386406144 | 424724379  | -               | 14.99 |
| 603 | 6690141884056924800 | 300405889  | -               | 16.00 |
| 604 | 6705696159663336320 | 340113714  | -               | 14.71 |
| 605 | 6706393937236340480 | 292019405  | -               | 15.26 |
| 606 | 6706897273042577024 | 90166569   | -               | 13.89 |
| 607 | 6707179022898207104 | 87547631   | -               | 14.82 |
| 608 | 6707258703133113216 | 87261652   | TYC 8361-113-1  | 12.62 |
| 609 | 6707425176065191936 | 86888953   | -               | 16.30 |
| 610 | 6707575121961384704 | 87892948   | -               | 15.95 |
| 611 | 6707581753390963712 | 88147424   | -               | 14.63 |
| 612 | 6708601928379030272 | 390558851  | -               | 16.34 |
| 613 | 6709029088645784704 | 405926734  | -               | 16.81 |
| 614 | 6709739093984603008 | 91151828   | -               | 15.33 |
| 615 | 6710128492894054656 | 397167012  | -               | 15.36 |
| 616 | 6710161169002313600 | 405862714  | -               | 13.24 |
| 617 | 6710746280990311552 | 268883654  | HD 174136       | 8.56  |
| 618 | 6712934107266220160 | 61568533   | HD 179235       | 9.36  |
| 619 | 6715668863267444352 | 254081333  | -               | 18.01 |
| 620 | 6716837266172193792 | 254002630  | -               | 15.78 |
| 621 | 6718384485185881088 | 254050616  | -               | 12.37 |
| 622 | 6719609173653801856 | 1695223044 | HD 165456       | 9.60  |
| 623 | 6719946723720769408 | 88232354   | CD-46 12230     | 10.41 |
| 624 | 6720217306662519808 | 87614856   | HD 166488       | 8.17  |
| 625 | 6720291970375487744 | 87617001   | -               | 16.58 |
| 626 | 6721011974380262656 | 86021350   | -               | 14.87 |
| 627 | 6721077090397112960 | 87535726   | -               | 15.01 |
| 628 | 6721186521851832064 | 88357018   | -               | 16.70 |
| 629 | 6721297645558364928 | 89046387   | -               | 14.85 |
| 630 | 6722166770833464192 | 91408747   | TYC 7910-2632-1 | 11.70 |
| 631 | 6723793463921722624 | 314323408  | -               | 16.78 |
| 632 | 6723877134204087296 | 62722069   | -               | 15.70 |
| 633 | 6723894829469751168 | 62882921   | -               | 15.40 |
| 634 | 6724029141687845632 | 86334926   | -               | 13.92 |
| 635 | 6724098818919340800 | 86414230   | -               | 15.94 |
| 636 | 6724163282108915712 | 62717688   | -               | 15.33 |
| 637 | 6724171627200295552 | 63085065   | -               | 16.70 |
| 638 | 6724206777217467392 | 85645459   | -               | 15.97 |
| 639 | 6724239453357123072 | 62888554   | -               | 16.60 |
| 640 | 6724360781883873152 | 87068904   | -               | 13.98 |
| 641 | 6724526120940614912 | 87414786   | TYC 7908-867-1  | 10.77 |

|     |                     |            |                 |       |
|-----|---------------------|------------|-----------------|-------|
| 642 | 6724624183633572736 | 89572664   | -               | 15.41 |
| 643 | 6724652770937042816 | 88611851   | -               | 14.70 |
| 644 | 6724668748215406464 | 57424707   | -               | 15.83 |
| 645 | 6724789831938042880 | 87411648   | -               | 16.07 |
| 646 | 6724821335497612544 | 368646953  | -               | 15.49 |
| 647 | 6725378895306643200 | 326129890  | -               | 16.94 |
| 648 | 6726064951865022464 | 1701331126 | -               | 19.58 |
| 649 | 6727137770292462336 | 113150377  | -               | 15.10 |
| 650 | 6727643713127429888 | 55922148   | -               | 15.12 |
| 651 | 6727758272805974144 | 1703497021 | -               | 14.88 |
| 652 | 6728221510824260736 | 57541132   | -               | 15.82 |
| 653 | 6728562531190495744 | 253741477  | -               | 13.98 |
| 654 | 6728799299847564160 | 316476530  | -               | 16.61 |
| 655 | 6729565522013567488 | 316214562  | TYC 7919-615-1  | 12.13 |
| 656 | 6729794396537366784 | 315091286  | -               | 15.46 |
| 657 | 6729954375477881472 | 315874222  | -               | 14.40 |
| 658 | 6732540392460834688 | 151945334  | HD 175760       | 8.93  |
| 659 | 6732881103632136832 | 277709796  | CD-32 14688     | 9.43  |
| 660 | 6733034004471840512 | 315277523  | -               | 15.26 |
| 661 | 6733112649599093760 | 314332665  | TYC 7406-672-1  | 11.75 |
| 662 | 6733112756994412544 | 314332717  | -               | 15.56 |
| 663 | 6733697044346441472 | 211221851  | -               | 13.77 |
| 664 | 6733744460785562880 | 314816327  | -               | 13.90 |
| 665 | 6734105512930090752 | 60456931   | -               | 15.42 |
| 666 | 6734135990019367808 | 60745776   | -               | 15.31 |
| 667 | 6734417911683319424 | 66396641   | -               | 14.50 |
| 668 | 6734554933980241664 | 27367933   | -               | 16.60 |
| 669 | 6734773741115797376 | 338224118  | -               | 16.26 |
| 670 | 6735459595847095808 | 391315814  | -               | 14.28 |
| 671 | 6736786500236754688 | 338208675  | HD 171773       | 9.95  |
| 672 | 6743398202922859008 | 391059353  | -               | 17.54 |
| 673 | 6744573752649904640 | 113126598  | TYC 7433-185-1  | 11.66 |
| 674 | 6755766613523795456 | 30608209   | -               | 15.07 |
| 675 | 6757835409067212672 | 112245959  | -               | 15.82 |
| 676 | 6760001691808665856 | 277476291  | -               | 14.58 |
| 677 | 6760700912479534336 | 108438382  | -               | 13.86 |
| 678 | 6761302718989508224 | 90532647   | -               | 16.47 |
| 679 | 6819845322255920384 | 2028782096 | HD 209385       | 9.85  |
| 680 | 945273614100334848  | 15924771   | TYC 2941-27-1   | 10.83 |
| 681 | -                   | 42711755   | TYC 2640-239-1  | -     |
| 682 | -                   | 128974867  | TYC 8279-1168-1 | -     |
