# Supplementary material for: A search for variable subdwarf B stars in TESS Full Frame Images III. An update on variable targets in both ecliptic hemispheres -- contamination analysis and new sdB pulsators
Source: arXiv:2301.01082 ancillary file (2023-01-03)
Supplement: Supplementary file 6 [file 4-south_pulsators.pdf]

**Table 4. SEH - 83 pulsator candidates**

| No. | Gaia DR2            | TIC       | G     | Variable contaminator                                                |
|-----|---------------------|-----------|-------|----------------------------------------------------------------------|
|     |                     |           | [mag] |                                                                      |
| 1   | 2921500461998485248 | 744231977 | 18.31 | TYC 6526-2198-1                                                      |
| 2   | 2927637764107094272 | 744958933 | 18.67 | ATO J106.3086-23.5750                                                |
| 3   | 3062196993541803904 | 754827446 | 17.45 | TYC 4817-751-1                                                       |
| 4   | 3087146252404755584 | 257068255 | 15.08 | none                                                                 |
| 5   | 3111790534231122944 | 284329074 | 15.26 | TYC 163-370-1                                                        |
| 6   | 3135760162593729792 | 318043125 | 15.14 | none                                                                 |
| 7   | 3167805630845394432 | 762068195 | 18.61 | TIC 440828323                                                        |
| 8   | 3229067399384875776 | 457225725 | 14.31 | none                                                                 |
| 9   | 3343211511104992512 | 247871256 | 12.07 | none                                                                 |
| 10  | 4923853724788504192 | 201251043 | 11.95 | none                                                                 |
| 11  | 5195370596485039360 | 309437982 | 11.64 | none                                                                 |
| 12  | 5196271513123121152 | 323174439 | 13.32 | none                                                                 |
| 13  | 5200393440479943808 | 356730219 | 12.02 | none                                                                 |
| 14  | 5224191377530306688 | 454961165 | 16.19 | none                                                                 |
| 15  | 5233348350879239680 | 906337576 | 18.98 | TYC 9230-1986-1                                                      |
| 16  | 5233397274851278720 | 906364997 | 18.00 | TYC 9230-650-1                                                       |
| 17  | 5237830853646781440 | 910533311 | 17.97 | TIC 400839754                                                        |
| 18  | 5249563295545862400 | 846723312 | 17.98 | TIC 269540771                                                        |
| 19  | 5249647030230264960 | 846766924 | 18.08 | TIC 363534697                                                        |
| 20  | 5250674622612902912 | 362098036 | 11.50 | none                                                                 |
| 21  | 5257667310412799104 | 854453711 | 15.63 | Eclipses: 163 Car (B2V);<br>183.91 and 205.9 $\mu$ Hz: TIC 469248153 |
| 22  | 5257747299878049152 | 442128473 | 10.77 | none                                                                 |
| 23  | 5266133451162548864 | 141684783 | 14.55 | none                                                                 |
| 24  | 5291746162211858688 | 349477778 | 15.41 | none                                                                 |
| 25  | 5298504894555743488 | 359056669 | 13.43 | none                                                                 |
| 26  | 5311214355632943744 | 810530414 | 17.31 | HD 78270 (F2/3IV/V)                                                  |
| 27  | 5314453718731068288 | 811223439 | 18.16 | TYC 8580-714-1                                                       |
| 28  | 5315487775054631040 | 811466418 | 17.62 | none                                                                 |
| 29  | 5333948923192853376 | 281555312 | 16.13 | none                                                                 |
| 30  | 5342621080656522880 | 265631178 | 14.45 | none                                                                 |
| 31  | 5347816273079220096 | 933707513 | 16.89 | TIC 80851607                                                         |
| 32  | 5362558250096941056 | 178621334 | 13.34 | none                                                                 |
| 33  | 5365175740610237568 | 864799220 | 18.62 | HD 90611 (Double or multiple star, F0IV/V)                           |
| 34  | 5366164442080271232 | 146721954 | 16.22 | TIC 146721958                                                        |
| 35  | 5391470732981138816 | 147136095 | 15.12 | TYC 7731-706-1                                                       |
| 36  | 5430557649797803264 | 3120302   | 16.48 | TIC 3120296                                                          |
| 37  | 5439887654492064256 | 25836205  | 13.16 | none                                                                 |
| 38  | 5478585589003785088 | 737275640 | 18.48 | HD 46698 (A9IV/V)                                                    |
| 39  | 5511191365810066176 | 123027362 | 15.96 | none                                                                 |
| 40  | 5518789334757310208 | 818321152 | 18.20 | HD 66815 (A9V)                                                       |
| 41  | 5525342630213336448 | 181142865 | 11.10 | none                                                                 |
| 42  | 5532057244648680704 | 768899830 | 18.91 | CD-44 3650 (A2)                                                      |

|    |                     |            |       |                                                                                              |
|----|---------------------|------------|-------|----------------------------------------------------------------------------------------------|
| 43 | 5603319543880484864 | 98487756   | 14.23 | TYC 7107-177-1                                                                               |
| 44 | 5618197551112972288 | 100472259  | 11.52 | none                                                                                         |
| 45 | 5622554881336253824 | 190720627  | 11.02 | none                                                                                         |
| 46 | 5644257664628455296 | 147520373  | 16.31 | TIC 147520378                                                                                |
| 47 | 5709005567912127744 | 834530823  | 16.50 | UCAC4 364-048648                                                                             |
| 48 | 5711817878148717184 | 140753138  | 12.85 | none                                                                                         |
| 49 | 5715409776475889792 | 415273200  | 13.92 | TYC 5992-124-1                                                                               |
| 50 | 5775032959148516224 | 1205151714 | 18.53 | 41.67 $\mu$ Hz + harmonics: TIC 384294161;<br>66.55 $\mu$ Hz: no signal in individual pixels |
| 51 | 5777941304844208384 | 310102142  | 15.91 | CD-76 839 (F0)                                                                               |
| 52 | 5820203061496596608 | 1108611714 | 17.57 | HD 138774 (A6/8)                                                                             |
| 53 | 5822943972181461504 | 1109489759 | 18.21 | TIC 341225454                                                                                |
| 54 | 5823403087017696384 | 446919722  | 12.98 | none                                                                                         |
| 55 | 5824303174727830784 | 1110689652 | 17.19 | TYC 9258-200-1                                                                               |
| 56 | 5848704155260300032 | 1121956723 | 17.74 | TIC 259019132                                                                                |
| 57 | 5849749515965664896 | 398597669  | 16.00 | none                                                                                         |
| 58 | 5853428275707783936 | 1019266145 | 16.30 | TYC 9010-2235-1                                                                              |
| 59 | 5867706872948520064 | 1028442563 | 18.50 | signal in all pixels                                                                         |
| 60 | 5872410931625754624 | 1035773311 | 17.50 | none                                                                                         |
| 61 | 5888715417783989760 | 461920379  | 13.94 | none                                                                                         |
| 62 | 5888889690364814464 | 144582845  | 15.42 | TIC 145812196                                                                                |
| 63 | 5912581241014136192 | 360220395  | 13.88 | GSC 08740-00359 (pul delta scuti)                                                            |
| 64 | 5915159531372950656 | 1314011445 | 18.75 | signal in all pixels                                                                         |
| 65 | 5922070855307705472 | 388832080  | 12.59 | none                                                                                         |
| 66 | 5922154826207612416 | 1514267365 | 18.96 | TIC 323890455                                                                                |
| 67 | 5929340031606260480 | 1321621063 | 18.70 | 174.77 and 266.2 $\mu$ Hz: TIC 420702904;<br>58 - 174 $\mu$ Hz: TYC 8717-1756-1              |
| 68 | 5989255482542099840 | 1163132002 | 17.95 | TIC 254707388                                                                                |
| 69 | 6008695187392779392 | 1169856895 | 18.95 | TYC 7837-1755-1                                                                              |
| 70 | 6052876249006118784 | 973849292  | 17.10 | TIC 380445207                                                                                |
| 71 | 6065759261068308608 | 1046158353 | 17.08 | TIC 241401813                                                                                |
| 72 | 6075713513480403200 | 991374485  | 18.51 | none                                                                                         |
| 73 | 6096794282417069696 | 1051339091 | 17.97 | TYC 8264-2468-1                                                                              |
| 74 | 6143764182206682112 | 22217594   | 15.18 | none                                                                                         |
| 75 | 6557944439951092224 | 2027194271 | 18.63 | HD 209142(A8V)                                                                               |
| 76 | 6643505922271000704 | 230975415  | 15.61 | HD 180934 (A7/8V)                                                                            |
| 77 | 6703551527875050624 | 1692650109 | 17.97 | no signal in individual pixels                                                               |
| 78 | 6710746285282878080 | 1819391406 | 18.29 | HD 174136 (A8V)                                                                              |
| 79 | 6719949708709640832 | 1695487554 | 18.31 | CD-46 12230 (A5)                                                                             |
| 80 | 6720217547165164160 | 1695657786 | 17.17 | HD 166488 (A8/F0+G/KIII)                                                                     |
| 81 | 6721697695986630784 | 89907858   | 14.79 | none                                                                                         |
| 82 | 6725906450391258240 | 1701013661 | 18.31 | signal in all pixels                                                                         |
| 83 | 6736786465858585088 | 1707873842 | 17.09 | HD 171773 (A9V)                                                                              |
