# Supplementary material for: A search for variable subdwarf B stars in TESS Full Frame Images III. An update on variable targets in both ecliptic hemispheres -- contamination analysis and new sdB pulsators
Source: arXiv:2301.01082 ancillary file (2023-01-03)
Supplement: Supplementary file 7 [file 6-south_eclipsing_binaries.pdf]

| Table 6. SEH - 83 eclipsing binaries                                |                     |            |       |        |                                                  |
|---------------------------------------------------------------------|---------------------|------------|-------|--------|--------------------------------------------------|
| No.                                                                 | Gaia DR2            | TIC        | G     | Period | Variable contaminator                            |
|                                                                     |                     |            | [mag] | [d]    |                                                  |
| 32 eclipsing binaries that show both primary and secondary eclipses |                     |            |       |        |                                                  |
| 1                                                                   | 2938186341221700480 | 60523137   | 16.23 | 1.2532 | none                                             |
| 2                                                                   | 3056677303432024960 | 753916356  | 17.97 | 2.4282 | TIC 68060528                                     |
| 3                                                                   | 4037952609036313728 | 1556986400 | 18.86 | 4.2844 | TIC 368875977                                    |
| 4                                                                   | 4038037855601783296 | 1557298522 | 17.18 | 2.9735 | TYC 7404-5579-1                                  |
| 5                                                                   | 4044609357370901632 | 1569961982 | 16.46 | 2.415  | RS Sgr (B3/4IV/V, EB)                            |
| 6                                                                   | 4046871808683609344 | 1577179385 | 17.94 | 2.6564 | HD 170460 (B8II)                                 |
| 7                                                                   | 4771354077652344704 | 685209944  | 17.02 | 0.8619 | X Pic (EB, A2)                                   |
| 8                                                                   | 5244004710201233664 | 371323868  | 16.77 | 5.9367 | TIC 371323853                                    |
| 9                                                                   | 5250397786202723840 | 847157315  | 17.33 | 6.1989 | none                                             |
| 10                                                                  | 5256736612505157888 | 462454783  | 13.02 | 4.6739 | TIC 462454808                                    |
| 11                                                                  | 5280371920582429696 | 176935277  | 15.90 | 1.0922 | TIC 176935274 and OGLE LMC755.20.000027 (RR Lyr) |
| 12                                                                  | 5335651516987122304 | 321175529  | 12.18 | 1.8844 | none                                             |
| 13                                                                  | 5368186306521653248 | 146317976  | 14.39 | 1.0496 | CRTS J103314.0-425702 (EB)                       |
| 14                                                                  | 5456955476569904384 | 942871718  | 18.01 | 3.3063 | TIC 363348244                                    |
| 15                                                                  | 5607596064297848960 | 778203221  | 17.23 | 1.1652 | TIC 97198226                                     |
| 16                                                                  | 5630930140581073664 | 827970537  | 17.09 | 2.5561 | none                                             |
| 17                                                                  | 5781106489583729792 | 309959661  | 16.16 | 2.4251 | OT Aps (B9.5IV, EB)                              |
| 18                                                                  | 5803207085617951360 | 1509000006 | 16.69 | 1.3974 | HD 159537 (A1V)                                  |
| 19                                                                  | 5907618251680775936 | 1155805356 | 18.05 | 2.7874 | TIC 455389016                                    |
| 20                                                                  | 6054299772960830208 | 976146222  | 16.72 | 1.8626 | ZZ Cru (B3V, EB)                                 |
| 21                                                                  | 6054936561988117120 | 450420664  | 10.64 | 2.9541 | none                                             |
| 22                                                                  | 6074860842215236864 | 990883707  | 18.07 | 1.3087 | signal in all pixels                             |
| 23                                                                  | 6134198327969742336 | 996495522  | 17.93 | 0.6491 | TIC 248079846                                    |
| 24                                                                  | 6144569024718252544 | 258379678  | 15.36 | 0.1739 | none                                             |
| 25                                                                  | 6148958309493216896 | 998016645  | 18.03 | 3.2584 | UCAC4 244-054022                                 |
| 26                                                                  | 6635283671237373696 | 1689813971 | 18.98 | 3.2146 | UCAC4 147-218248                                 |
| 27                                                                  | 6652952415078798208 | 76760933   | 13.85 | 0.3613 | none                                             |
| 28                                                                  | 6655102952444592256 | 1817787859 | 16.52 | 0.9444 | TIC 6353630                                      |
| 29                                                                  | 6704092350154675072 | 1692824895 | 16.74 | 2.8881 | CRTS J183755.6-484955 (EB)                       |
| 30                                                                  | 6726045641698117888 | 1701292115 | 9.18  | 1.8459 | none                                             |
| 31                                                                  | 6785257198999941248 | 270535918  | 13.42 | 1.3423 | none                                             |
| 32                                                                  | 6819845494052294784 | 2028782100 | 18.26 | 2.9797 | HD 209385 (A2mA6-F3) and [TGC2005] 333 (RR Lyr)  |
| 42 eclipsing binaries that show primary eclipses only               |                     |            |       |        |                                                  |
| 1                                                                   | 2337436792938619392 | 33984762   | 15.47 | 0.1445 | none                                             |
| 2                                                                   | 2912425780212327680 | 37737816   | 16.96 | 0.1488 | none                                             |
| 3                                                                   | 2926324156946337280 | 707111651  | 17.82 | 2.6908 | TIC 48404603                                     |
| 4                                                                   | 2943004023214007424 | 33743252   | 14.02 | 0.4886 | none                                             |
| 5                                                                   | 2983108331879225344 | 189012795  | 15.32 | 0.1889 | none                                             |
| 6                                                                   | 3108435168343024768 | 756875938  | 17.21 | 1.0354 | TIC 5096969                                      |
| 7                                                                   | 3117155669938231552 | 42566802   | 16.04 | 0.1986 | none                                             |
| 8                                                                   | 3133124560206025472 | 202273662  | 12.39 | 4.4319 | none                                             |
| 9                                                                   | 4648210184093228032 | 141280240  | 15.80 | 2.0908 | UX Men (F8V, EB)                                 |
| 10                                                                  | 5217847259856665088 | 843283217  | 17.95 | 1.9444 | TIC 452591808                                    |

|                                                   |                     |            |       |         |                                                                                          |
|---------------------------------------------------|---------------------|------------|-------|---------|------------------------------------------------------------------------------------------|
| 11                                                | 5251043302606589312 | 847473488  | 18.25 | 6.8704  | no signal in individual pixels                                                           |
| 12                                                | 5252903160911109632 | 849266771  | 18.86 | 0.5458  | TIC 378027065                                                                            |
| 13                                                | 5289914135324381696 | 308541002  | 16.56 | 0.2105  | none                                                                                     |
| 14                                                | 5305025578320680960 | 383375636  | 15.51 | 1.1821  | none                                                                                     |
| 15                                                | 5305259503712750848 | 856066667  | 18.48 | 0.8298  | TIC 361064918                                                                            |
| 16                                                | 5337514085339321856 | 280246753  | 12.21 | 0.5821  | none                                                                                     |
| 17                                                | 5499736649371768192 | 255594396  | 17.41 | 0.1585  | none                                                                                     |
| 18                                                | 5518740367833012224 | 818308005  | 17.48 | 0.2049  | 56.48 $\mu$ Hz + harmonics: none;<br>13.19 $\mu$ Hz + harmonics: V410 Pup                |
| 19                                                | 5611769771782124160 | 779128665  | 18.99 | 1.7065  | 2MASS J07274341-2908218 (EB)                                                             |
| 20                                                | 5713928455133099904 | 834924649  | 18.36 | 2.1812  | TIC 11070498                                                                             |
| 21                                                | 5755874037751559424 | 95785714   | 15.81 | 0.1559  | none                                                                                     |
| 22                                                | 5778067198920743040 | 1309769412 | 17.80 | 2.8099  | TIC 310270073                                                                            |
| 23                                                | 5796639427794797568 | 401617089  | 13.12 | 5.9992  | TIC 401617111                                                                            |
| 24                                                | 5799206233387125376 | 1106932458 | 18.19 | 1.5615  | TIC 263024559                                                                            |
| 25                                                | 5799225238637101952 | 1106947173 | 18.29 | 2.5142  | 18.17 $\mu$ Hz + harmonics: TIC 262833444;<br>4.63 $\mu$ Hz + harmonics: IX TrA (RR Lyr) |
| 26                                                | 5811904287015654656 | 1509561926 | 17.72 | 1.5239  | 102.89 $\mu$ Hz: none;<br>Eclipses: TYC 9289-2657-1                                      |
| 27                                                | 5824483803880454912 | 1110889969 | 17.74 | 2.1506  | Eclipses: TIC 262927909;<br>45.95 $\mu$ Hz: TIC 262920132                                |
| 28                                                | 5825554728205038080 | 424717152  | 15.09 | 2.0156  | TIC 424717153                                                                            |
| 29                                                | 5828964515592711936 | 1209068896 | 17.33 | 0.7066  | TIC 1209068824                                                                           |
| 30                                                | 5843724123479161344 | 957158511  | 17.24 | 1.673   | UCAC4 094-038759 (YSO candidate)                                                         |
| 31                                                | 5876767059272719232 | 1130777039 | 15.89 | 2.2711  | TIC 44278854                                                                             |
| 32                                                | 5921479897855061248 | 1513749999 | 18.38 | 0.9524  | TIC 73703617                                                                             |
| 33                                                | 5922518558382783616 | 1315988153 | 18.89 | 1.7541  | TIC 367328654                                                                            |
| 34                                                | 5923149678073282560 | 1316233834 | 18.40 | 0.698   | TIC 366954637                                                                            |
| 35                                                | 5928428227229275136 | 1219774587 | 18.90 | 2.8496  | TYC 8720-1555-1                                                                          |
| 36                                                | 6066425668214614784 | 986927321  | 17.30 | 0.6241  | HD 113554 (B3/5IV)                                                                       |
| 37                                                | 6097540197980557440 | 242402846  | 16.36 | 0.1274  | none                                                                                     |
| 38                                                | 6136619310835929984 | 996840740  | 18.31 | 0.9006  | CRTS J131829.0-424319 (EB)                                                               |
| 39                                                | 6207027744809208320 | 1174994870 | 17.78 | 1.5731  | TYC 7318-1177-1 (EB)                                                                     |
| 40                                                | 6401799112903799168 | 410442849  | 14.70 | 0.1117  | none                                                                                     |
| 41                                                | 6655972155043097600 | 456516418  | 13.56 | 0.2786  | none                                                                                     |
| 42                                                | 6720657317455798400 | 1695999069 | 16.26 | 0.3536  | none                                                                                     |
| <b>9 eclipsing binaries with eccentric orbits</b> |                     |            |       |         |                                                                                          |
| 1                                                 | 3047770537696481408 | 187657618  | 9.86  | -       | none                                                                                     |
| 2                                                 | 4038509271151105280 | 1558593400 | 18.79 | 2.8936  | HD 321646 (A3)                                                                           |
| 3                                                 | 5001375586674001024 | 616535392  | 18.78 | 11.0648 | CG Scl (G6V, EB)                                                                         |
| 4                                                 | 5249773989468659456 | 846855557  | 18.42 | 4.5177  | Eclipses: TIC 269544397;<br>69.91 $\mu$ Hz + harmonic: TIC 269544423                     |
| 5                                                 | 5332893048437332608 | 305898260  | 11.83 | 9.9141  | none                                                                                     |
| 6                                                 | 562023333557469952  | 139334900  | 13.00 | 2.9054  | none                                                                                     |
| 7                                                 | 5695384542987752064 | 832426099  | 9.86  | 3.0607  | AC Pyx (A0/1IV, EB)                                                                      |
| 8                                                 | 5809975095078956160 | 1509255862 | 18.98 | 4.2926  | PP Aps (A3mA5-A8, EB)                                                                    |
| 9                                                 | 6757323899938326272 | 1826847776 | 18.86 | 1.9224  | V526 Sgr (A0V, EB)                                                                       |
