# Supplementary material for: A search for variable subdwarf B stars in TESS Full Frame Images III. An update on variable targets in both ecliptic hemispheres -- contamination analysis and new sdB pulsators
Source: arXiv:2301.01082 ancillary file (2023-01-03)
Supplement: Supplementary file 8 [file 8-south_no_spec_phased_LC.pdf]

| Table 8. SEH - 273 spectroscopically unclassified variables with phased light curves |                     |            |       |        |                                      |
|--------------------------------------------------------------------------------------|---------------------|------------|-------|--------|--------------------------------------|
| No.                                                                                  | Gaia DR2            | TIC        | G     | Period | Variable contaminator                |
|                                                                                      |                     |            | [mag] | [d]    |                                      |
| One symmetric maximum                                                                |                     |            |       |        |                                      |
| 1                                                                                    | 2896588449084891136 | 49547169   | 13.28 | 0.3086 | IS CMa (F3V)                         |
| 2                                                                                    | 2905822663130146688 | 31353391   | 14.03 | 0.8929 | none                                 |
| 3                                                                                    | 2909497952544966272 | 37118148   | 14.28 | 0.2681 | none                                 |
| 4                                                                                    | 2911497105202950400 | 37004041   | 15.16 | 0.2833 | none                                 |
| 5                                                                                    | 2921050693020996864 | 63113578   | 11.45 | 0.4854 | none                                 |
| 6                                                                                    | 2924341084643425024 | 49774041   | 10.69 | 2.439  | none                                 |
| 7                                                                                    | 2936588029269162624 | 60348471   | 14.49 | 2.439  | none                                 |
| 8                                                                                    | 2957941296696980608 | 708356594  | 17.88 | 0.339  | NGC 1904 23 (RR Lyr)                 |
| 9                                                                                    | 2993468995592753920 | 34264736   | 15.93 | 0.1761 | none                                 |
| 10                                                                                   | 2995717462506292736 | 317804295  | 15.94 | 0.1706 | none                                 |
| 11                                                                                   | 3006362139517524608 | 709860036  | 18.69 | 2.1277 | TIC 443326977                        |
| 12                                                                                   | 3010515995663287424 | 332831934  | 16.41 | 1.0417 | none                                 |
| 13                                                                                   | 3026543267432558336 | 139785230  | 15.94 | 0.0937 | none                                 |
| 14                                                                                   | 3038538526969624192 | 170301183  | 12.29 | 3.0303 | none                                 |
| 15                                                                                   | 3040772322279673472 | 32302937   | 14.26 | 0.2618 | none                                 |
| 16                                                                                   | 3049609165952551680 | 125264225  | 11.12 | 1.1494 | none                                 |
| 17                                                                                   | 3052993703264602112 | 177514185  | 14.61 | 0.2564 | none                                 |
| 18                                                                                   | 3055532608748900864 | 64730323   | 14.74 | 0.6024 | none                                 |
| 19                                                                                   | 3061898441775753216 | 65145461   | 15.57 | 0.1163 | none                                 |
| 20                                                                                   | 3069130101545218560 | 803407565  | 10.98 | 2.5641 | none                                 |
| 21                                                                                   | 3083216116810048768 | 73238638   | 15.32 | 0.1376 | none                                 |
| 22                                                                                   | 3083335826137398400 | 803870626  | 16.25 | 0.2653 | none                                 |
| 23                                                                                   | 3136176770124825216 | 759533492  | 18.37 | 0.431  | TYC 169-1547-1                       |
| 24                                                                                   | 3150707232898463616 | 468928859  | 15.60 | 0.266  | none                                 |
| 25                                                                                   | 3151064780336438656 | 271207314  | 14.21 | 0.142  | none                                 |
| 26                                                                                   | 3151362095151274752 | 19026014   | 15.37 | 0.5525 | TYC 788-877-1 (Solar type)           |
| 27                                                                                   | 3217698036836906624 | 11197405   | 15.21 | 0.0755 | none                                 |
| 28                                                                                   | 3239171705085395072 | 672588015  | 17.43 | 3.125  | TIC 455040026                        |
| 29                                                                                   | 3341157696395192320 | 716209046  | 18.72 | 0.1745 | ATO J084.8000+12.6523 (EB candidate) |
| 30                                                                                   | 3468413690428028288 | 951159803  | 18.59 | 0.1414 | CRTS J122641.7-333204 (EB)           |
| 31                                                                                   | 3480090194676896384 | 901200174  | 18.66 | 0.5435 | TIC 293110371                        |
| 32                                                                                   | 3532585694447087232 | 20446816   | 12.91 | 1.0753 | none                                 |
| 33                                                                                   | 3573965638463072768 | 902378838  | 18.54 | 1.3889 | TIC 335499532                        |
| 34                                                                                   | 4035348484483331584 | 1401293420 | 18.44 | 0.1946 | -                                    |
| 35                                                                                   | 4038372381956935680 | 1558161606 | 18.94 | 0.5435 | signal in all pixels                 |
| 36                                                                                   | 4038805177242745600 | 1559754008 | 18.97 | 0.3745 | TIC 56585584                         |
| 37                                                                                   | 4045364760494465024 | 1571918587 | 18.95 | 2.439  | TIC 61555986                         |
| 38                                                                                   | 4046774712424275200 | 1576915471 | 17.48 | 0.2712 | TIC 28512009                         |
| 39                                                                                   | 4716642550852732672 | 237907939  | 14.20 | 0.1381 | none                                 |
| 40                                                                                   | 4752367504705559936 | 146687440  | 14.60 | 1.4925 | none                                 |
| 41                                                                                   | 4756267369383483904 | 149599018  | 14.59 | 5.8824 | none                                 |
| 42                                                                                   | 4762428207898487168 | 685137498  | 18.50 | 0.1346 | HD 32475 (F0IV)                      |
| 43                                                                                   | 4829447221183169024 | 206474978  | 15.96 | 0.2155 | none                                 |
| 44                                                                                   | 4909378967742431360 | 206564279  | 13.78 | 1.4286 | TIC 206564278                        |
| 45                                                                                   | 4927555166260455040 | 382416478  | 14.15 | 0.7519 | none                                 |
| 46                                                                                   | 5194902582490530560 | 804500973  | 18.07 | 3.7037 | TIC 389013472                        |
| 47                                                                                   | 5196065251613078912 | 804549027  | 17.95 | 0.1227 | none                                 |
| 48                                                                                   | 5199247646285490432 | 394563922  | 15.94 | 0.1151 | none                                 |
| 49                                                                                   | 5201664480218395136 | 842747184  | 18.16 | 1.3889 | TIC 394238292                        |

|     |                     |           |       |        |                                                                                                 |
|-----|---------------------|-----------|-------|--------|-------------------------------------------------------------------------------------------------|
| 50  | 5213207393804130816 | 271888015 | 13.03 | 0.8146 | none                                                                                            |
| 51  | 5214328517707616128 | 271642755 | 13.56 | 2.2222 | none                                                                                            |
| 52  | 5231883973199654400 | 398791871 | 11.82 | 1.1236 | none                                                                                            |
| 53  | 5232515157294643712 | 844059251 | 18.78 | 0.1845 | HD 91441 (B6/8V)                                                                                |
| 54  | 5239154184595202048 | 844338903 | 18.29 | 0.7407 | TIC 397786565                                                                                   |
| 55  | 5239571311849267200 | 465456367 | 14.46 | 1.8519 | TIC 465456405                                                                                   |
| 56  | 5242975056226807296 | 372815862 | 13.02 | 1.2346 | none                                                                                            |
| 57  | 5243482686998229376 | 371016851 | 14.37 | 0.2415 | none                                                                                            |
| 58  | 5244874526978221824 | 845251687 | 18.88 | 0.5348 | TIC 373034540                                                                                   |
| 59  | 5246146180897092608 | 845838164 | 17.64 | 0.3106 | TIC 845838161                                                                                   |
| 60  | 5249910741223769728 | 846930961 | 17.51 | 2.0833 | HD 84865 (ApSi, RotV*alf2CVn)                                                                   |
| 61  | 5251560902025244416 | 377658867 | 15.24 | 0.2132 | 54.28 µHz + harmonics: none;<br>76.27 µHz: TIC 378037013                                        |
| 62  | 5266468802206471296 | 167250176 | 14.26 | 0.1595 | none                                                                                            |
| 63  | 5269596049498087424 | 765017261 | 17.13 | 0.1247 | TIC 306472729                                                                                   |
| 64  | 5270373786471521024 | 306505851 | 16.03 | 0.1706 | none                                                                                            |
| 65  | 5291112774796009600 | 765677577 | 17.79 | 0.1605 | TIC 341330235                                                                                   |
| 66  | 5293139655760876544 | 765773357 | 17.66 | 3.4483 | TIC 349192518                                                                                   |
| 67  | 5296462581763471104 | 356837752 | 16.20 | 0.2639 | none                                                                                            |
| 68  | 5296549340102210688 | 806872820 | 18.01 | 3.8462 | TIC 356207241                                                                                   |
| 69  | 5298070003345815680 | 807215500 | 16.78 | 0.1873 | TIC 357117415                                                                                   |
| 70  | 5322521183433578752 | 388622589 | 10.90 | 0.8475 | 13.77 µHz: none;<br>161.92 µHz: TIC 388622573                                                   |
| 71  | 5341595751704487680 | 300685376 | 14.50 | 1.9608 | TIC 300685428                                                                                   |
| 72  | 5349904589251539456 | 82591181  | 13.10 | 2.3256 | none                                                                                            |
| 73  | 5355588720798713728 | 862023654 | 16.67 | 0.3663 | TIC 464339039                                                                                   |
| 74  | 5355946268217174656 | 463006021 | 14.27 | 1.2821 | 53.01 µHz + harmonics: none;<br>9.03 µHz: TIC 463006006;<br>6.71 µHz + harmonics: TIC 463006054 |
| 75  | 5361576454936897664 | 937597821 | 18.58 | 0.1724 | TIC 80682970                                                                                    |
| 76  | 5363099308598820096 | 937974717 | 18.95 | 0.2273 | TIC 147188371                                                                                   |
| 77  | 5369091410756158080 | 400919731 | 13.99 | 0.1447 | none                                                                                            |
| 78  | 5371061903087037696 | 94246301  | 11.95 | 4.1667 | none                                                                                            |
| 79  | 5371604000980277120 | 61762775  | 12.69 | 2.7027 | none                                                                                            |
| 80  | 5388590356113794816 | 941437058 | 18.07 | 0.2766 | TIC 72063751                                                                                    |
| 81  | 5390464817279368448 | 29917475  | 16.34 | 0.3135 | none                                                                                            |
| 82  | 5391620507080621824 | 158196468 | 12.94 | 3.5714 | none                                                                                            |
| 83  | 5393463597805768320 | 158223878 | 12.00 | 1.4493 | none                                                                                            |
| 84  | 5407683822210499072 | 867459631 | 18.98 | 1.087  | TYC 8187-1501-1                                                                                 |
| 85  | 5434346012808677632 | 70717873  | 13.66 | 1.2048 | none                                                                                            |
| 86  | 5434436383219257472 | 29723252  | 14.05 | 0.1502 | none                                                                                            |
| 87  | 5448344724273336064 | 71674519  | 14.42 | 1.5152 | none                                                                                            |
| 88  | 5457161703718981504 | 942878246 | 18.53 | 0.1479 | CRTS J110007.1-262459 (EB)                                                                      |
| 89  | 5477101965563632000 | 737151632 | 18.62 | 1.6949 | TIC 372851666                                                                                   |
| 90  | 5477508583007863936 | 149973540 | 13.50 | 1.1364 | none                                                                                            |
| 91  | 5497677749426668800 | 238069203 | 14.18 | 0.1555 | none                                                                                            |
| 92  | 5502168150617145216 | 238019887 | 15.24 | 0.7692 | none                                                                                            |
| 93  | 5520454369017441664 | 818833960 | 18.72 | 0.6369 | TIC 80804874                                                                                    |
| 94  | 5526271511387514880 | 83081722  | 16.41 | 0.1658 | none                                                                                            |
| 95  | 5546533513520296192 | 146117756 | 13.90 | 0.1048 | none                                                                                            |
| 96  | 5552604814865254400 | 170100070 | 15.34 | 0.3165 | none                                                                                            |
| 97  | 5560208483233550720 | 770973891 | 18.72 | 0.3484 | TYC 7638-357-1 (RRLyr)                                                                          |
| 98  | 5561999385810491264 | 170310610 | 15.32 | 0.813  | none                                                                                            |
| 99  | 5576826952945841408 | 148044670 | 15.55 | 0.3096 | none                                                                                            |
| 100 | 5584309675031744512 | 52388210  | 15.25 | 0.3831 | none                                                                                            |

|     |                     |            |       |        |                                                   |
|-----|---------------------|------------|-------|--------|---------------------------------------------------|
| 101 | 5591407473561155328 | 113929655  | 10.47 | 0.6788 | none                                              |
| 102 | 5599470673377393920 | 775878600  | 16.13 | 0.1767 | ATO J112.7262-30.0820 (EB)                        |
| 103 | 5611820525418596608 | 108121382  | 16.26 | 0.207  | none                                              |
| 104 | 5615708084989439488 | 415143942  | 15.17 | 0.1114 | none                                              |
| 105 | 5627260280004729472 | 17460375   | 13.44 | 0.1318 | none                                              |
| 106 | 5647085093133918720 | 196417751  | 11.86 | 1.6393 | none                                              |
| 107 | 5693570688108267648 | 831888569  | 18.42 | 2.3256 | TIC 196318935                                     |
| 108 | 5696368773398103296 | 832623391  | 18.30 | 0.4608 | TYC 6556-175-1                                    |
| 109 | 5697870946801360512 | 833025831  | 16.90 | 0.0985 | none                                              |
| 110 | 5698379200347454208 | 833137917  | 18.61 | 0.2597 | TYC 6558-1725-1                                   |
| 111 | 5709579959659083008 | 834573650  | 17.68 | 0.1631 | ATO J128.7529-17.4813 (EB candidate)              |
| 112 | 5709912046530451840 | 405300501  | 15.34 | 1.3699 | none                                              |
| 113 | 5715265255110912128 | 140674813  | 9.97  | 3.8462 | none                                              |
| 114 | 5716391812157166336 | 415224879  | 13.51 | 0.2151 | none                                              |
| 115 | 5753841281270433536 | 51431668   | 15.28 | 0.0889 | none                                              |
| 116 | 5768566765625082112 | 384295509  | 14.01 | 0.9009 | none                                              |
| 117 | 5785766490440028160 | 418757007  | 15.56 | 0.1376 | none                                              |
| 118 | 5790175845607430656 | 396256097  | 16.91 | 0.3717 | none                                              |
| 119 | 5796024319747525504 | 1106127339 | 18.23 | 2.6316 | TIC 263670290                                     |
| 120 | 5802848777968872832 | 1309947558 | 18.25 | 0.1422 | TIC 310799640                                     |
| 121 | 5804243753280956672 | 1309967972 | 18.83 | 4.3478 | TIC 311529705                                     |
| 122 | 5809162246755246720 | 1206329315 | 18.38 | 2.2727 | no signal in individual pixels                    |
| 123 | 5810573710448599680 | 294196248  | 12.96 | 1.2658 | none                                              |
| 124 | 5810658029245818240 | 1509377483 | 15.55 | 1.6667 | no signal in individual pixels                    |
| 125 | 5816413422869352448 | 1311566852 | 17.60 | 0.1905 | TIC 301747913                                     |
| 126 | 5832749206423000832 | 1212998545 | 18.06 | 0.4115 | signal in all pixels                              |
| 127 | 5856360741911875840 | 448006966  | 16.80 | 0.1175 | none                                              |
| 128 | 5878353036051735424 | 1036707862 | 15.06 | 0.3026 | none                                              |
| 129 | 5917085051098353152 | 1315252102 | 18.35 | 0.2688 | signal in all pixels                              |
| 130 | 5921549652415561856 | 1513801292 | 18.31 | 1.9608 | TIC 1513801289                                    |
| 131 | 5929155867700733056 | 170432227  | 15.24 | 0.2755 | TIC 170432176                                     |
| 132 | 5946889718944314880 | 1517742678 | 18.74 | 0.2985 | TIC 96099359                                      |
| 133 | 5947682054521782400 | 1518444947 | 18.98 | 0.8403 | TIC 390088830                                     |
| 134 | 5947917934120939264 | 1518643967 | 18.75 | 1.6667 | TYC 8348-2426-1                                   |
| 135 | 5949607883502930560 | 1521051042 | 17.57 | 0.3165 | TIC 214249847                                     |
| 136 | 5949903476020736640 | 1521545612 | 17.53 | 0.1629 | TIC 1521545773                                    |
| 137 | 5951695443759022976 | 1523004908 | 18.70 | 0.7874 | Gaia DR2 5951695336375324288<br>(Candidate RRLyr) |
| 138 | 5951799313240078080 | 1523231725 | 18.56 | 1.25   | HD 157832 (Variable Be star, B2ne)                |
| 139 | 6003468079048102400 | 1167947965 | 18.14 | 0.1681 | TYC 7834-1214-1                                   |
| 140 | 6005939265801702272 | 1168863300 | 17.83 | 0.1608 | TIC 148264694                                     |
| 141 | 6031156290142441344 | 191221080  | 12.83 | 0.2053 | none                                              |
| 142 | 6057220728665468416 | 253184319  | 15.39 | 0.4854 | none                                              |
| 143 | 6069641872841587200 | 1047202529 | 18.11 | 1.2346 | TIC 241533827                                     |
| 144 | 6074817239704924672 | 990861367  | 17.78 | 0.1887 | TIC 419779192                                     |
| 145 | 6085079806361861888 | 994074308  | 18.90 | 0.4348 | TYC 8251-437-1 (EB)                               |
| 146 | 6096267234097192320 | 242463073  | 12.12 | 1.9231 | none                                              |
| 147 | 6098441797519559552 | 1172688066 | 18.97 | 0.1852 | TYC 8279-1168-1                                   |
| 148 | 6104664243055570560 | 159259371  | 15.91 | 0.152  | TIC 159154997                                     |
| 149 | 6115504259470702592 | 166894438  | 15.84 | 0.1238 | none                                              |
| 150 | 6132361177176695680 | 996245434  | 17.05 | 0.1773 | CRTS J124318.8-453428 (EB)                        |
| 151 | 6148834236479971712 | 21641328   | 13.96 | 1.0989 | none                                              |
| 152 | 6155138767433459840 | 103831994  | 12.22 | 1.1765 | none                                              |
| 153 | 6157729113749149056 | 130924318  | 13.90 | 0.5236 | none                                              |

|                        |                     |            |       |        |                                                                                                                                    |
|------------------------|---------------------|------------|-------|--------|------------------------------------------------------------------------------------------------------------------------------------|
| 154                    | 6159105255630163456 | 131236578  | 15.14 | 0.2525 | none                                                                                                                               |
| 155                    | 6359368722966483840 | 276796039  | 14.08 | 4.7619 | none                                                                                                                               |
| 156                    | 6381776422045939584 | 2054761216 | 18.98 | 1.6393 | UCAC3 33-129092<br>(Eruptive variable Star, M2.3)                                                                                  |
| 157                    | 6431145460504666752 | 1688544000 | 17.76 | 5.5556 | TIC 292621879                                                                                                                      |
| 158                    | 6461831833600743936 | 316788032  | 14.78 | 1.0989 | none                                                                                                                               |
| 159                    | 6562425082977942272 | 2027302068 | 17.08 | 0.1645 | TIC 139896280                                                                                                                      |
| 160                    | 6576260585683860736 | 147146907  | 15.31 | 0.1441 | none                                                                                                                               |
| 161                    | 6629592225394313216 | 411918964  | 13.83 | 0.1832 | none                                                                                                                               |
| 162                    | 6636107617762820864 | 1816807538 | 17.91 | 0.2053 | TIC 120249063                                                                                                                      |
| 163                    | 6657826477106032256 | 6665844    | 13.84 | 1.4286 | none                                                                                                                               |
| 164                    | 6659367339573565312 | 1923720827 | 17.86 | 0.4202 | CRTS J193712.5-480921 (RR Lyr)                                                                                                     |
| 165                    | 6662709786201498240 | 1818609250 | 18.78 | 0.2174 | -                                                                                                                                  |
| 166                    | 6706393731068755840 | 1693385914 | 17.95 | 2.0408 | TIC 292019405                                                                                                                      |
| 167                    | 6707425171762916608 | 1693952468 | 18.91 | 0.1305 | TIC 86888953                                                                                                                       |
| 168                    | 6709739098282201472 | 1694913243 | 17.68 | 0.3521 | TIC 91151828                                                                                                                       |
| 169                    | 6712934171688784256 | 1819863744 | 18.87 | 0.8772 | HD 179235 (A9V)                                                                                                                    |
| 170                    | 6718384656985946112 | 1821060671 | 18.35 | 1.4493 | TIC 254050616                                                                                                                      |
| 171                    | 6719608933120159744 | 1695222843 | 18.06 | 1.0638 | HD 165456 (G5)                                                                                                                     |
| 172                    | 6721077154808040832 | 1696401635 | 18.67 | 0.1684 | TIC 87535726                                                                                                                       |
| 173                    | 6724206712797091456 | 1698589712 | 17.27 | 0.2849 | TIC 85645459                                                                                                                       |
| 174                    | 6724526120927993600 | 1698985611 | 18.45 | 0.4785 | TYC 7908-867-1                                                                                                                     |
| 175                    | 6727643648730503040 | 1703278418 | 18.20 | 0.1783 | TIC 55922148                                                                                                                       |
| 176                    | 6729391970973866752 | 1821836358 | 18.13 | 0.3745 | Gaia DR2 6729391975273949184<br>(RRLyr candidate)                                                                                  |
| 177                    | 6729565522015146240 | 1821904001 | 18.20 | 0.2268 | TYC 7919-615-1                                                                                                                     |
| 178                    | 6733034004471841664 | 1704918722 | 18.46 | 0.3356 | TIC 315277523                                                                                                                      |
| 179                    | 6734105474265563136 | 1705799658 | 18.88 | 0.3774 | TIC 60456931                                                                                                                       |
| 180                    | 6734417873003845888 | 1706301214 | 18.10 | 0.2165 | TIC 66396641                                                                                                                       |
| 181                    | 6742873224773448960 | 1925740295 | 18.35 | 3.7037 | HD 181321 (spectroscopic binary, G2V)                                                                                              |
| 182                    | 6743398202922849664 | 1825788527 | 18.53 | 0.1506 | TIC 391059353                                                                                                                      |
| 183                    | 6760001859308263808 | 1827654125 | 18.44 | 0.2309 | TIC 277476291                                                                                                                      |
| 184                    | 6761309114219270144 | 1828793177 | 18.26 | 0.274  | Gaia DR2 6761309114226077952<br>(Candidate_RRLyr)                                                                                  |
| 185                    | 6794666712135593344 | 1992439824 | 18.11 | 0.1484 | CRTS J205410.7-295417 (EB)                                                                                                         |
| One asymmetric maximum |                     |            |       |        |                                                                                                                                    |
| 1                      | 2922539741007440768 | 79689537   | 16.70 | 3.125  | 82.64 $\mu$ Hz + harmonics: none;<br>3.7 $\mu$ Hz + harmonic: TIC 79689505;<br>5.56 $\mu$ Hz + harmonic: ATO J104.6541-23.0081 (V) |
| 2                      | 2927154597462957056 | 48524451   | 14.50 | 0.2488 | none                                                                                                                               |
| 3                      | 2957940029686164352 | 708350288  | 18.10 | 0.7407 | NGC 1904 192 (RR Lyr)                                                                                                              |
| 4                      | 2957940029686166016 | 708350292  | 17.50 | 0.7353 | NGC 1904 192 (RR Lyr)                                                                                                              |
| 5                      | 3037520241761387264 | 750862698  | 19.00 | 0.3003 | ATO J117.2835-10.5983<br>(RRLyr candidate)                                                                                         |
| 6                      | 3047774184120137088 | 752216365  | 18.50 | 5.8824 | TIC 187591950                                                                                                                      |
| 7                      | 3786348167772858368 | 902790976  | 17.71 | 0.6849 | 2MASS J11311380-0403591 (RR Lyr)                                                                                                   |
| 8                      | 4702811313050785280 | 39017348   | 16.47 | 0.8065 | TIC 39017347                                                                                                                       |
| 9                      | 5304690746979284480 | 809316750  | 18.43 | 0.3788 | HD 77525 (B5Vn)                                                                                                                    |
| 10                     | 5383736493312165248 | 940928992  | 15.79 | 1.7857 | HD 99627(A0V)                                                                                                                      |
| 11                     | 5393973114069348096 | 941900430  | 17.47 | 0.5348 | CRTS J105621.7-382439 (RR Lyr)                                                                                                     |
| 12                     | 5439868103801897600 | 873480537  | 16.66 | 0.0873 | TIC 11932252                                                                                                                       |
| 13                     | 5461053601219563520 | 71338192   | 11.00 | 2.0408 | none                                                                                                                               |
| 14                     | 5496278341705187968 | 737473774  | 16.78 | 3.4483 | TIC 260538568                                                                                                                      |
| 15                     | 5579436712515286016 | 96520292   | 13.17 | 1.2987 | none                                                                                                                               |
| 16                     | 5689491195023189248 | 296724066  | 14.38 | 2.2727 | none                                                                                                                               |

|            |                     |            |       |        |                                      |
|------------|---------------------|------------|-------|--------|--------------------------------------|
| 17         | 5719124334768705920 | 54275411   | 12.03 | 1.5625 | none                                 |
| 18         | 5821920567383105664 | 1207491680 | 17.61 | 0.4065 | UCAC4 121-145252 (RR Lyr)            |
| 19         | 5824470506633796480 | 1110873767 | 17.34 | 3.4483 | R TrA (F7Ib/II, deltaCep)            |
| 20         | 5865963326711336832 | 325986533  | 13.12 | 1.087  | HD 121841 (B8II/III(pSi))            |
| 21         | 5914259512380607872 | 174187648  | 14.18 | 0.4717 | V503 Ara (RR Lyr)                    |
| 22         | 5917758433248059776 | 1511991718 | 18.77 | 0.6238 | WZ Pav (RRLyr)                       |
| 23         | 5945298691274098304 | 363483973  | 16.42 | 0.4505 | none                                 |
| 24         | 5947381578621154432 | 363706224  | 11.81 | 0.2247 | none                                 |
| 25         | 5951113321119542528 | 217365202  | 13.35 | 0.7929 | none                                 |
| 26         | 6039655274470700544 | 1172278318 | 17.11 | 0.4878 | CRTS J155556.9-312338 (RR Lyr)       |
| 27         | 6083769463385060736 | 1048223010 | 16.71 | 0.6536 | Cl* NGC 5139 SAW V134 (RR Lyr)       |
| 28         | 6087145380693985408 | 1048399825 | 18.88 | 0.3831 | CRTS J132310.3-453548 (RR Lyr)       |
| 29         | 6118854333959388672 | 1054281677 | 18.96 | 0.6897 | CRTS J143521.9-360617 (RR Lyr)       |
| 30         | 6662237855196197120 | 1818520053 | 18.88 | 0.6849 | CRTS J185258.8-484252 (RR Lyr)       |
| 31         | 6710128458534307968 | 1819242966 | 18.32 | 0.6098 | TIC 397167012                        |
| 32         | 6716837266172193152 | 1820684543 | 18.52 | 0.578  | TIC 254002630                        |
| 33         | 6724239453327875072 | 1698634750 | 17.37 | 0.5102 | TIC 62888554                         |
| 34         | 6733781534926708096 | 1705468240 | 18.20 | 0.4587 | V3678 Sgr (RR Lyr)                   |
| 35         | 6734982648321929216 | 1707147184 | 16.62 | 0.4405 | V3448 Sgr (RR Lyr)                   |
| 36         | 6735459595828246400 | 1823921368 | 18.99 | 0.525  | TIC 391315814                        |
| Two maxima |                     |            |       |        |                                      |
| 1          | 2909679852999761536 | 33166796   | 14.30 | 2.3256 | none                                 |
| 2          | 2978115793174302848 | 671282181  | 17.92 | 2.1277 | TIC 121549920                        |
| 3          | 3016508570255997184 | 710301636  | 17.07 | 1.2821 | TIC 388851561                        |
| 4          | 3047771538430246784 | 752215680  | 18.35 | 1.7544 | TYC 5395-1656-1                      |
| 5          | 3052741330986502912 | 125197892  | 12.72 | 1.2426 | none                                 |
| 6          | 3070438000690624384 | 803473779  | 17.61 | 0.4016 | TIC 88792275                         |
| 7          | 3109216818032728448 | 4999380    | 14.81 | 1.389  | TIC 4999366                          |
| 8          | 3111794588680353152 | 284124761  | 14.50 | 0.6452 | ATO J108.5124+01.1230 (EB candidate) |
| 9          | 3236488827993523584 | 713259786  | 16.53 | 0.2433 | CRTS J052935.4+040651 (EB)           |
| 10         | 4679135456154867200 | 293218310  | 15.98 | 0.4367 | none                                 |
| 11         | 4714790492235234176 | 231062312  | 13.07 | 1.6949 | none                                 |
| 12         | 4821689823052057728 | 192826669  | 15.71 | 1.4286 | none                                 |
| 13         | 4850445793032736384 | 301050418  | 10.72 | 1.8182 | none                                 |
| 14         | 5216785445160303744 | 287977499  | 12.58 | 0.0976 | none                                 |
| 15         | 5217109006519074176 | 804970406  | 18.74 | 0.3344 | TIC 288067102                        |
| 16         | 5219652387372513792 | 304299578  | 15.62 | 0.2008 | none                                 |
| 17         | 5334796165656329728 | 325158549  | 11.05 | 2.3256 | none                                 |
| 18         | 5365504803821448576 | 864903758  | 18.07 | 0.3058 | TIC 103455699                        |
| 19         | 5365570048662587520 | 864920508  | 18.65 | 0.3175 | TIC 103184931                        |
| 20         | 5366842561574019456 | 938222499  | 18.90 | 0.3484 | CRTS J104333.0-444559 (EB)           |
| 21         | 5429638694292915200 | 4264922    | 12.76 | 0.0742 | none                                 |
| 22         | 5496812536854546432 | 278861557  | 15.26 | 0.1318 | none                                 |
| 23         | 5507683266582438528 | 767550400  | 17.44 | 0.266  | TIC 60608976                         |
| 24         | 5532741999879105920 | 821330826  | 17.55 | 0.3077 | TIC 79798831                         |
| 25         | 5562578205666649088 | 771265934  | 17.36 | 0.6245 | TIC 130571889                        |
| 26         | 5645678401141009280 | 830270910  | 18.88 | 0.2713 | ATO J128.8091-28.1387 (V)            |
| 27         | 5775607999433058432 | 1205184125 | 16.72 | 0.2342 | none                                 |
| 28         | 5793581819094668544 | 1105179202 | 18.92 | 0.8929 | TYC 9270-1649-1                      |
| 29         | 5815712656008942592 | 1311306525 | 18.08 | 0.7519 | HD 149613 (RotV*, F3V)               |
| 30         | 5832312223592931072 | 1212826072 | 17.39 | 0.5181 | TIC 343364326                        |
| 31         | 5911440811230926592 | 1510915106 | 18.38 | 6.25   | TIC 307232499                        |
| 32         | 5915710764651751936 | 367140246  | 15.82 | 0.2519 | UNSW-V 305 (EB)                      |

|    |                     |            |       |        |                            |
|----|---------------------|------------|-------|--------|----------------------------|
| 33 | 5916995406555045760 | 1315155037 | 18.56 | 0.4505 | TIC 171213459              |
| 34 | 5946192624280057216 | 1516975280 | 18.19 | 0.6849 | TIC 323887849              |
| 35 | 5951804879518557952 | 1523243111 | 17.52 | 0.3058 | TIC 218140405              |
| 36 | 6035804338088673152 | 1255310693 | 18.88 | 0.3185 | TIC 94927513               |
| 37 | 6083471774916181888 | 1048022421 | 17.01 | 0.3774 | TIC 425433597              |
| 38 | 6092765087704842496 | 1050189754 | 16.94 | 0.3774 | TYC 8268-1377-1            |
| 39 | 6198287933039480192 | 1173764699 | 17.02 | 0.2857 | TIC 121101104              |
| 40 | 6224708304100799488 | 1176220959 | 17.16 | 0.3636 | ATO J227.1742-27.4436 (V)  |
| 41 | 6381526046928596992 | 260824263  | 16.78 | 0.5593 | none                       |
| 42 | 6621871759681427072 | 2028297898 | 18.84 | 0.2833 | CRTS J222347.4-264549 (EB) |
| 43 | 6648008014367949568 | 1690227091 | 17.00 | 0.4157 | TIC 119220200              |
| 44 | 6649398381180416128 | 119153557  | 16.36 | 0.4132 | QW Tel (F8/G0, EB)         |
| 45 | 6656795070777810688 | 158237390  | 16.32 | 2.7778 | TYC 8387-854-1             |
| 46 | 6724652770937040896 | 1699111897 | 17.15 | 0.7317 | TIC 88611851               |
| 47 | 6728562458170704128 | 1821458807 | 17.14 | 0.3584 | TIC 253741477              |
| 48 | 6729954371169136256 | 1704724045 | 18.66 | 0.3953 | TIC 315874222              |
| 49 | 6732540388160365696 | 151945339  | 15.21 | 1.2658 | HD 175760 (B9V)            |
| 50 | 6733697078706189696 | 1823584142 | 17.91 | 0.5435 | TIC 211221851              |
| 51 | 6744573756943257472 | 113059781  | 15.86 | 1.0424 | TYC 7433-185-1             |
| 52 | 6755766609220203520 | 1826089601 | 17.71 | 0.2933 | TIC 30608209               |
