# Supplementary material for: A search for variable subdwarf B stars in TESS Full Frame Images III. An update on variable targets in both ecliptic hemispheres -- contamination analysis and new sdB pulsators
Source: arXiv:2301.01082 ancillary file (2023-01-03)
Supplement: Supplementary file 9 [file 9-north_no_spec_phased_LC.pdf]

**Table 9. NEH - 93 spectroscopically unclassified variables with phased light curves**

| No.                   | Gaia DR2            | TIC        | G     | Period | Variable contaminator                                                                               |
|-----------------------|---------------------|------------|-------|--------|-----------------------------------------------------------------------------------------------------|
|                       |                     |            | [mag] | [d]    |                                                                                                     |
| One symmetric maximum |                     |            |       |        |                                                                                                     |
| 1                     | 1000519267329142144 | 444946935  | 15.92 | 1.6725 | none                                                                                                |
| 2                     | 1086341235118052096 | 85158691   | 12.85 | 0.3546 | none                                                                                                |
| 3                     | 1099487030500185344 | 743328948  | 16.90 | 0.3297 | none                                                                                                |
| 4                     | 1133795950814826240 | 841399917  | 17.31 | 1.5134 | none                                                                                                |
| 5                     | 1141625057721183616 | 138400883  | 16.24 | 0.0680 | none                                                                                                |
| 6                     | 1328061818442252032 | 1270377531 | 17.50 | 0.3913 | Pul -3 1330158                                                                                      |
| 7                     | 1336799091888985600 | 9569988    | 11.87 | 2.7441 | none                                                                                                |
| 8                     | 1344525738054881152 | 116262175  | 14.43 | 2.5163 | none                                                                                                |
| 9                     | 141494094091434880  | 67658009   | 13.04 | 0.8764 | none                                                                                                |
| 10                    | 156955941997427456  | 96951247   | 15.72 | 0.1592 | none                                                                                                |
| 11                    | 1708730890216076416 | 159438888  | 14.41 | 0.6370 | none                                                                                                |
| 12                    | 1816292363253864064 | 1943106787 | 18.86 | 0.8747 | no signal in individual pixels                                                                      |
| 13                    | 1816586516979325696 | 1943243403 | 18.42 | 0.2286 | ATO J304.9401+20.2202 (V)                                                                           |
| 14                    | 1817158988879945600 | 219640470  | 14.18 | 0.5359 | none                                                                                                |
| 15                    | 1831343410431617920 | 406417817  | 14.71 | 0.2010 | none                                                                                                |
| 16                    | 1844828920542477568 | 1951933220 | 16.55 | 0.1909 | TYC 2181-560-1                                                                                      |
| 17                    | 1856240648652853760 | 282366215  | 14.83 | 0.6220 | TIC 282366186                                                                                       |
| 18                    | 1893009515772824064 | 2002921529 | 17.30 | 0.2410 | ASAS J215731+2713.5 (EB)                                                                            |
| 19                    | 1896251498822626560 | 18000205   | 14.03 | 1.1013 | none                                                                                                |
| 20                    | 1902886016408161280 | 2040326958 | 17.64 | 1.4690 | 131.94 $\mu$ Hz: none;<br>7.87 $\mu$ Hz+harmonic: TIC 10596964                                      |
| 21                    | 1920489236226682496 | 125489130  | 16.78 | 0.1229 | none                                                                                                |
| 22                    | 1922534396571549184 | 2040945100 | 18.19 | 1.7462 | TIC 177398591                                                                                       |
| 23                    | 1973144057810900096 | 427916222  | 16.22 | 0.3723 | ATO J327.9786+43.5247 (EB candidate)                                                                |
| 24                    | 1997600078330802688 | 345216287  | 16.49 | 0.0935 | TYC 4004-623-1                                                                                      |
| 25                    | 2042814161128667136 | 1713892529 | 18.93 | 2.8649 | TYC 2640-239-1                                                                                      |
| 26                    | 2046397439474347904 | 1874192801 | 14.25 | 0.5796 | none                                                                                                |
| 27                    | 2050133678755873792 | 1876676459 | 18.51 | 0.7463 | V556 Lyr (A0, EB)                                                                                   |
| 28                    | 2050526964622031744 | 1714628258 | 17.22 | 0.5351 | none                                                                                                |
| 29                    | 2068952271239193344 | 193800883  | 15.10 | 0.2926 | none                                                                                                |
| 30                    | 2071550515996622592 | 188973075  | 16.36 | 1.0682 | TIC 188973040                                                                                       |
| 31                    | 2072903984764773248 | 1879342714 | 17.86 | 0.1761 | HD 187235 (B8Vn)                                                                                    |
| 32                    | 2080900114347408384 | 416641307  | 14.60 | 0.3011 | ATO J303.5545+43.5235 (EB candidate)                                                                |
| 33                    | 2086292772201176320 | 1881864796 | 17.26 | 1.9530 | 1.62 $\mu$ Hz+harmonic: 2MASS<br>J19514349+4637130 (RotV*);<br>other signal: TYC 3557-955-1 (RotV*) |
| 34                    | 2088590094368104448 | 1973148204 | 18.17 | 0.7242 | TIC 351295092                                                                                       |
| 35                    | 2089872678980572032 | 1714844032 | 17.88 | 5.6149 | TIC 425914150                                                                                       |
| 36                    | 2091796510791468288 | 68673218   | 13.71 | 0.3164 | TIC 68673212                                                                                        |
| 37                    | 2101329963798339968 | 1716151993 | 18.68 | 0.3907 | UCAC4 654-070475 (Eruptive V)                                                                       |
| 38                    | 2125305094015307520 | 21018674   | 13.41 | 1.5079 | none                                                                                                |
| 39                    | 2126639381440599552 | 1882566921 | 17.71 | 0.8298 | HD 182805 (F0V, RotV*)                                                                              |
| 40                    | 2135864872411150720 | 26665817   | 14.75 | 1.9827 | none                                                                                                |

|                               |                     |            |       |        |                                         |
|-------------------------------|---------------------|------------|-------|--------|-----------------------------------------|
| 41                            | 2149604919464450944 | 353989024  | 14.94 | 1.0026 | none                                    |
| 42                            | 2160276263927353600 | 233733792  | 12.46 | 2.5694 | none                                    |
| 43                            | 2187704543559462784 | 1978995005 | 17.73 | 0.1560 | V2477 Cyg (F8, EB)                      |
| 44                            | 2221479066861091840 | 305721914  | 17.04 | 0.2348 | none                                    |
| 45                            | 2233741920045058944 | 417763975  | 15.26 | 2.4500 | TYC 4606-830-1                          |
| 46                            | 2234314074112207872 | 1883795387 | 17.84 | 0.5660 | TYC 3943-1962-1 (V)                     |
| 47                            | 2243609212271977088 | 467268413  | 16.99 | 0.1860 | TIC 467268412                           |
| 48                            | 2248022166610310144 | 1981211186 | 18.16 | 0.1158 | TYC 4244-667-1                          |
| 49                            | 2265587418916463104 | 229763894  | 15.08 | 0.5257 | none                                    |
| 50                            | 2303705631625361024 | 397532904  | 12.89 | 0.4204 | none                                    |
| 51                            | 333069804659746560  | 184690162  | 12.87 | 0.7554 | none                                    |
| 52                            | 3662392216154435200 | 392877333  | 12.89 | 0.9526 | none                                    |
| 53                            | 431408849046443264  | 359433191  | 16.50 | 0.4417 | TIC 359433277                           |
| 54                            | 4501536260662226560 | 264050369  | 13.20 | 1.5903 | none                                    |
| 55                            | 4525959987335693056 | 1684609529 | 16.91 | 0.1213 | ATO J277.6248+20.9722 (EB)              |
| 56                            | 4539247241754918400 | 337071076  | 13.14 | 1.5048 | none                                    |
| 57                            | 4585910377796460288 | 84835513   | 13.54 | 3.1513 | none                                    |
| 58                            | 4598451682297980288 | 310989305  | 14.01 | 2.4847 | none                                    |
| 59                            | 562213078769245440  | 396484881  | 15.79 | 0.6073 | none                                    |
| 60                            | 564551735705888384  | 609725827  | 16.58 | 0.1068 | none                                    |
| 61                            | 893386457796229504  | 741295718  | 16.72 | 1.2233 | none                                    |
| 62                            | 925671353297509632  | 29118824   | 13.37 | 2.2698 | none                                    |
| 63                            | 946065369848575872  | 16600409   | 15.40 | 1.1703 | none                                    |
| <b>One asymmetric maximum</b> |                     |            |       |        |                                         |
| 1                             | 1328057149815681920 | 1270359835 | 14.42 | 1.4561 | CI* NGC 6205 SAW V56                    |
| 2                             | 1328058043172963456 | 1270366381 | 16.37 | 0.7509 | NGC 6205 206 (RR Lyr)                   |
| 3                             | 1360405537821429504 | 1270837578 | 16.27 | 0.7026 | CI* NGC 6341 HAC 1 (RR Lyr)             |
| 4                             | 1360405572181155712 | 334899908  | 15.77 | 0.7018 | CI* NGC 6341 HAC 1 (RR Lyr)             |
| 5                             | 1360408320957344512 | 1270842390 | 16.57 | 0.6298 | CI* NGC 6341 SAW V4 (RR Lyr)            |
| 6                             | 1418837537086251264 | 1271027428 | 18.96 | 0.4771 | ROTSE1 J171520.08+525441.2 (RR Lyr)     |
| 7                             | 1702017375296326528 | 1102619251 | 18.72 | 4.8500 | TIC 257024839                           |
| 8                             | 1705393833770160128 | 288381009  | 16.43 | 1.8706 | TIC 288381017                           |
| 9                             | 1939433718495541632 | 177243718  | 13.64 | 1.1822 | none                                    |
| 10                            | 2093534465017435776 | 258279532  | 10.89 | 3.9000 | none                                    |
| 11                            | 2105187256745838080 | 1716561881 | 17.74 | 4.3001 | 2MASS J18515292+4305429 (RotV*)         |
| 12                            | 2167371859151731712 | 195728426  | 16.22 | 3.1822 | TIC 195728444                           |
| 13                            | 2198794939398092160 | 330843247  | 16.29 | 0.6260 | TYC 3990-344-1                          |
| 14                            | 4534814663708775552 | 1814743619 | 17.55 | 3.1277 | ATO J284.6835+26.1722 (V)               |
| 15                            | 4607722936142361216 | 1508465315 | 18.80 | 0.5967 | [SHM2017] J267.46836+35.35881 (RR Lyr)  |
| 16                            | 524799859180542080  | 54051804   | 14.24 | 2.1242 | ASASSN-V J011429.92+643910.3 (deltaCep) |
| <b>Two maxima</b>             |                     |            |       |        |                                         |
| 1                             | 1816862670495460352 | 1943342834 | 18.11 | 0.3207 | TIC 1943342821                          |
| 2                             | 1907427033790181248 | 2003766169 | 18.24 | 0.7305 | HD 213872 (A3)                          |
| 3                             | 1962740066464303744 | 2006587293 | 7.58  | 2.4021 | V1942 Cyg (alpha2 CVn)                  |
| 4                             | 1976684313460272128 | 2010382498 | 17.00 | 2.5714 | TIC 326709771                           |

|    |                     |            |       |        |                          |
|----|---------------------|------------|-------|--------|--------------------------|
| 5  | 1979662924824022528 | 2011878719 | 16.11 | 0.3919 | TIC 384371809            |
| 6  | 2039164989422375168 | 1712800054 | 16.68 | 0.8764 | TIC 403535217            |
| 7  | 2100480767163455360 | 121107327  | 16.26 | 0.5772 | TYC 3124-382-1 (EB)      |
| 8  | 2242271072260536832 | 229463748  | 13.82 | 1.2363 | none                     |
| 9  | 2288995609155671936 | 1884532373 | 16.56 | 0.4107 | TIC 237211570            |
| 10 | 3974187703469677568 | 156952109  | 13.39 | 0.5971 | none                     |
| 11 | 4532553445024997376 | 1813751285 | 18.16 | 3.2319 | TIC 314483554            |
| 12 | 4554252723613727872 | 1506996219 | 16.82 | 0.4738 | ASAS J173105+2025.1 (EB) |
| 13 | 498498166646842496  | 310922669  | 11.81 | 0.5656 | none                     |
| 14 | 504667698197248640  | 445526365  | 10.12 | 2.0482 | none                     |
